# Supplementary material for: Data-driven and constrained optimization of semi-local exchange and non-local correlation functionals for materials and surface chemistry
Source: arXiv:2201.11106 ancillary file (2022-04-07)
Supplement: Supplementary file 1 [file SI.pdf]

# Supporting Information: Data-driven and constrained optimization of semi-local exchange and non-local correlation functionals for materials and surface chemistry

Kai Trepte*† , Johannes Voss*‡

April 7, 2022

## Contents

**1 Further details for rVV10** **2**

**2 Transformation functions for $s$ and $\alpha$** **2**

**3 Functional fitting procedure** **3**

**4 Fitting weights** **4**

**5 Final exchange enhancement expansion coefficients $c_{ij}$** **6**

**6 Additional results** **7**

6.1 Mean and mean absolute errors . . . . . . . . . . . . . . . . . . . . . . . . . 7

6.2 All values for all functionals . . . . . . . . . . . . . . . . . . . . . . . . . 8

6.3 All errors for all functionals . . . . . . . . . . . . . . . . . . . . . . . . . 34

*SUNCAT Center for Interface Science and Catalysis, SLAC National Accelerator Laboratory, 2575 Sand Hill Road, Menlo Park, CA 94025, USA

†ktrepte@slac.stanford.edu

‡vossj@slac.stanford.edu

# 1 Further details for rVV10

Note that, in atomic units,

$$\omega_0(\mathbf{r}) = \sqrt{\omega_g^2(\mathbf{r}) + \frac{\omega_p^2(\mathbf{r})}{3}} \tag{1}$$

$$\omega_g^2(\mathbf{r}) = C\left|\frac{\boldsymbol{\nabla} n(\mathbf{r})}{n(\mathbf{r})}\right|^4 \tag{2}$$

$$\omega_p^2(\mathbf{r}) = 4\pi n(\mathbf{r}) \tag{3}$$

with $\omega_0$ being introduced in the main manuscript. Here, $\omega_g$ is the so-called local band gap which depends on the parameter $C$. Similar to Sabatini et al.[1] and Peng et al.,[2] we keep $C = 0.0093$ fixed at the value proposed by Vydrov and Van Voorhis.[3]

# 2 Transformation functions for $s$ and $\alpha$

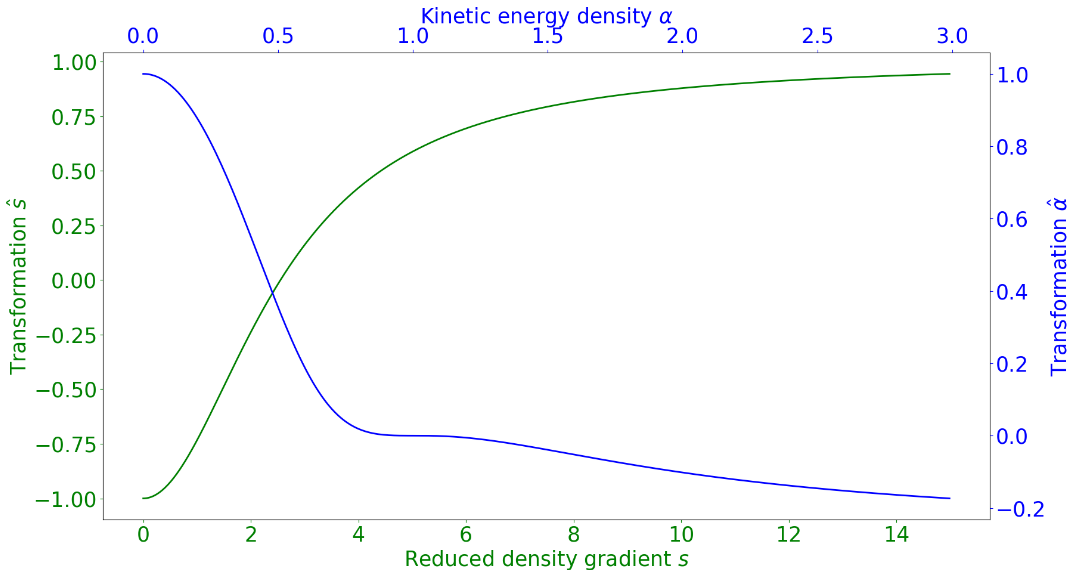


Figure SF1: Transformation of $s$ (green) and $\alpha$ (blue) from their semi-infinite intervals to the finite intervals as used in the Legendre polynomial expansion of the exchange-enhancement factor.

# 3 Functional fitting procedure

The exchange-enhancement factor fitting procedure has been outlined in Brown et al.[4] for MCML. This procedure is summarized below. Reaction energies, e.g., for DBH24 or RE42, are computed as

$$E_{\text{react}} = \sum_{n}^{N_{\text{P}}} p_n E_n - \sum_{m}^{N_{\text{R}}} p_m E_m, \tag{4}$$

where $N_{\text{P}}$ and $N_{\text{R}}$ are the number of products and reactants in the reaction, $p$ are the stochiometric prefactors and $E$ are the total energies.

Given that by fitting $F_{\text{X}}$ only the exchange energy is affected, the fitting itself does not change any other energy contribution. Also, given that no changes are imposed upon the atomic arrangements as well as the self-consistent density, no terms other than the exchange energy are affected by the fitting. As such, one can extract all contributions besides the exchange energy, non-X (including nuclear-nuclear, nuclear-electron, kinetic as well as correlation terms), as they are not going to change during fitting

$$E_{\text{react}} = \sum_{n}^{N_{\text{P}}} p_n (E_{\text{X},n} + E_{\text{non-X},n}) - \sum_{m}^{N_{\text{R}}} p_m (E_{\text{X},m} + E_{\text{non-X},m}), \tag{5}$$

Consequently, one can represent the reaction energy in terms of the exchange energy contributions for the products and reactants, keeping the non-X terms constant. The exchange contributions are then modified when refitting $F_{\text{X}}$. Thus, one obtains a non-self-consistent (nonSCF) estimate of the reaction energy

$$E_{\text{react}}^{\text{nonSCF}} = \sum_{n}^{N_{\text{P}}} p_n (E_{\text{X},n}^{\text{nonSCF}} + E_{\text{non-X},n}) - \sum_{m}^{N_{\text{R}}} p_m (E_{\text{X},m}^{\text{nonSCF}} - E_{\text{non-X},m}), \tag{6}$$

which can be used to get a nonSCF estimate of the errors per data set. The $F_{\text{X}}$, and consequently all $E_{\text{X}}^{\text{nonSCF}}$ contributions, is modified until all errors are as small as possible. In more detail, the exchange energy contributions for any system $k$ having a self-consistent density $n_k(\mathbf{r})$ can be calculated as

$$E_{\text{X},k}^{\text{nonSCF}} = \sum_{i=0}^{7} \sum_{j=0}^{7} c_{ij} I_{ij,k} \tag{7}$$

with the 64 volume integrals

$$I_{ij,k} = \int \mathrm{d}^3 r P_i\left(\hat{s}(\mathbf{r})\right) P_j\left(\hat{\alpha}(\mathbf{r})\right) \cdot n_k(\mathbf{r}) \cdot \epsilon_{\text{X}}^{\text{HEG}}[n_k(\mathbf{r})]. \tag{8}$$

By keeping the electronic densities fixed at their computed level of theory during the optimization of the $c_{ij}$, evaluating the exchange energy estimates requires little computational effort, as the integrals in Eq. (8) are only evaluated once per system. This strategy for generating a $c_{ij}$-parameterized estimate for the exchange component of any reaction energy allows for the non-self-consistent prediction of the error.

This strategy can similarly be applied to lattice constants as well as bulk moduli. Having the equilibrium unit cell volume $V_{\mathrm{eq}}$ for any solid, one can compute energies around this equilibrium volume by adjusting $V_{\mathrm{eq}}$ by a small perturbation $\pm v\Delta V$, where $v$ is an integer. Using the energy at equilibrium, $E_{\mathrm{eq}}$, as well as the energies at the modified volumes, $E_{\mathrm{eq}\pm v}$, the bulk modulus can be approximated using a five-point stencil with constant volume spacing $\Delta V$

$$B_{\mathrm{approx}} = V_{\mathrm{eq}} \frac{-E_{\mathrm{eq}-2} + 16E_{\mathrm{eq}-1} - 30E_{\mathrm{eq}} + 16E_{\mathrm{eq}+1} - E_{\mathrm{eq}+2}}{12(\Delta V)^2}. \tag{9}$$

The lattice constant, or rather the unit cell volume, can equally be approximated by the minimum of a parabola through the three volumes around $V_{\mathrm{eq}}$

$$V_{\mathrm{approx}} = -\frac{V_{\mathrm{eq}}}{2(\Delta V)^2 B_{\mathrm{approx}}} \left((-2V_{\mathrm{eq}} - \Delta V)E_{\mathrm{eq}-1} + 4V_{\mathrm{eq}}E_{\mathrm{eq}} + (-2V_{\mathrm{eq}} + \Delta V)E_{\mathrm{eq}+1}\right). \tag{10}$$

With these approximations, nonSCF predictions of the bulk moduli as well as the lattice constants can be obtained for any set of $c_{ij}$ in analogy to Eq. (5) by subtracting the self-consistent energies from $E_{\mathrm{eq}\pm v}$ and adding the respective exchange energies, Eq. (7). The equations (5), (9) and (10) are linear in $c_{ij}$, making the optimization of the functional efficient.

As a note, for the final optimization step to arrive at VCML, we made sure that the nonSCF errors on the S66x8 remain small (by adjusting the increase in the corresponding weight from 0.0075 to 0.23, and also lowering the respective threshold to 5 meV instead of the original 19 meV, see next section), which avoids re-optimizing the $b$ parameter a third time.

# 4 Fitting weights

As mentioned in the main text, the weights for the fitting procedure were adjusted in an automated fashion. In Tab. ST1, we present the thresholds for each data set, as well as the increase in the corresponding weight if the predicted MAE is larger than the threshold. The same data sets as used in Brown et al.[4] were employed. The thresholds and the increase in weights were chosen so that the fit gives the best compromise between the errors of all data sets. Such a fit is biased towards certain data sets. The weights in the end are chosen to give the best errors, and they need to be carefully adjusted given certain trade-offs between errors of different data sets; for example, decreasing the errors in the cohesive energies or the chemisorption data in ADS41 is typically associated with an increase in the error for the lattice constants. The final weights represent the best compromise we could find between all these trade-offs, aiming at a functional with optimal performance for reaction energies between molecules and surfaces and bulk lattice and elastic properties.

Table ST1: Thresholds $\delta$ and increase in weight $\Delta w$ for the automated procedure to obtain the weights described in the main manuscript. The starting values of all weights are 1. The weights were adjusted according to the importance of the data set for the fit. $^{\dagger}$Values for $\delta$ and $\Delta w$ for lattice constants and bulk moduli as computed using finite volume differences (rather than equation of state (EOS) fits used for self-consistent evaluation of these properties with the optimized VCML-rVV10 and all other functionals considered here).

| Data set | $\delta$ | $\Delta w$ |
|---|---|---|
| DBH24 | 0.265 eV | 0.005 |
| RE42 | 0.270 eV | 0.005 |
| S66x8 | 0.019 eV | 0.0075 |
| $a_{\text{lat}}$@SOL62 $^{\dagger}$ | 0.042 Å | 0.19 |
| $E_{\text{coh}}$@SOL62 | 0.235 eV | 0.22 |
| $B$@SOL62 $^{\dagger}$ | 11.0 GPa | 0.005 |
| $E_{\text{ads}}^{\text{phy}}$@ADS41 | 0.145 eV | 0.0075 |
| $E_{\text{ads}}^{\text{che}}$@ADS41 | 0.255 eV | 0.275 |

The final weights, after final brute-force individual parameter adjustments, for the VCML exchange functional are given in Tab. ST2. Note that in our procedure we add the W4-11 data set, as the original MCML functional[4] performed poorly on this set. Accordingly, it was added to improve the performance on the atomization energies.

Table ST2: Final weights in the fitting procedure to obtain the VCML exchange functional.

| Data set | $w_{\text{final}}$ |
|---|---|
| DBH24 | 1.000 |
| RE42 | 1.090 |
| S66x8 | 10.900 |
| W4-11 | 0.050 |
| $a_{\text{lat}}$@SOL62 | 11.532 |
| $E_{\text{coh}}$@SOL62 | 10.842 |
| $B$@SOL62 | 1.000 |
| $E_{\text{ads}}^{\text{phy}}$@ADS41 | 1.270 |
| $E_{\text{ads}}^{\text{che}}$@ADS41 | 24.143 |

## 5 Final exchange enhancement expansion coefficients $c_{ij}$

The final, optimized coefficients defining the semi-local exchange part of VCML-rVV10 are given in Tab. ST3.

Table ST3: Final coefficients $c_{ij}$. Index $i$ corresponds to Legendre polynomials for $s$, while index $j$ corresponds to Legendre polynomials for $\alpha$ (see main manuscript for additional details).

| | | | | | | | |
|---|---|---|---|---|---|---|---|
| $c_{00}$ | 1.1050362267560025 | $c_{20}$ | -0.00068200282327089 | $c_{40}$ | -0.001432652476750007 | $c_{60}$ | 0.00030574929164576756 |
| $c_{01}$ | -0.1304673327239498 | $c_{21}$ | 0.0012341314639045392 | $c_{41}$ | 0.0050995906979556666 | $c_{61}$ | 0.0005970286163074767 |
| $c_{02}$ | -0.25273044468938444 | $c_{22}$ | -0.000835331263170036 | $c_{42}$ | 0.0003180493235941731 | $c_{62}$ | -0.0009048853909642742 |
| $c_{03}$ | 0.0020345583050872945 | $c_{23}$ | -7.823588139015819e-05 | $c_{43}$ | -0.004704436332280876 | $c_{63}$ | -0.000689695394243961 |
| $c_{04}$ | 0.009705556829333915 | $c_{24}$ | -0.0014878680171769923 | $c_{44}$ | 0.0009891355730978566 | $c_{64}$ | 0.0001331797359718674 |
| $c_{05}$ | -0.0018727613481398786 | $c_{25}$ | 0.005061925051098745 | $c_{45}$ | -0.0010249162124576494 | $c_{65}$ | -0.007555456486598222 |
| $c_{06}$ | 0.005056319358478653 | $c_{26}$ | -0.007631605623646023 | $c_{46}$ | 0.0008367073496483024 | $c_{66}$ | 0.001864317026752979 |
| $c_{07}$ | -0.0014994572626212954 | $c_{27}$ | -0.01006770315965861 | $c_{47}$ | -0.00031389079758955066 | $c_{67}$ | -0.00019095139973664826 |
| $c_{10}$ | 0.19526954394443446 | $c_{30}$ | -0.00217177716567727 | $c_{50}$ | -0.004500541251076788 | $c_{70}$ | -0.002025317083565653 |
| $c_{11}$ | 0.12131628073942294 | $c_{31}$ | 0.0024977311122498513 | $c_{51}$ | 0.0016437722411542371 | $c_{71}$ | 0.0023160016166370034 |
| $c_{12}$ | -0.013135604251829597 | $c_{32}$ | -0.0008670535705479461 | $c_{52}$ | 8.482767148525194e-05 | $c_{72}$ | 0.00018939021743243079 |
| $c_{13}$ | -0.016823429546012295 | $c_{33}$ | 0.0027822064319562786 | $c_{53}$ | -0.00019375881298946268 | $c_{73}$ | 0.0004308565933608885 |
| $c_{14}$ | -0.0021100890252897446 | $c_{34}$ | -0.0002571281595426713 | $c_{54}$ | -7.261106354828029e-05 | $c_{74}$ | -1.792697304428732e-05 |
| $c_{15}$ | -0.0016609256494831233 | $c_{35}$ | -3.656012084198544e-05 | $c_{55}$ | -0.0038541498256550073 | $c_{75}$ | -0.0005194058669188706 |
| $c_{16}$ | 0.0028206838819829017 | $c_{36}$ | -0.009195715678311926 | $c_{56}$ | -0.0031296536914037784 | $c_{76}$ | -0.00018156466410673526 |
| $c_{17}$ | 0.00017309630990864668 | $c_{37}$ | 0.010726279571787276 | $c_{57}$ | 0.0038758929812102785 | $c_{77}$ | -0.00029476504977320184 |

# 6 Additional results

In the following tables, we abbreviate rVV10 with -v to save space.

## 6.1 Mean and mean absolute errors

Table ST4: Mean errors for all data sets used within this study. Functionals with '-v' employ the rVV10 methodology. Units are provided.

| Data Set | Unit | PBE | PBE-D3 | MS2 | SCAN | $r^2$SCAN | SCAN-v | MCML | MCML-v | VCML-v |
|---|---|---|---|---|---|---|---|---|---|---|
| DBH24 | eV | −0.356 | −0.365 | −0.260 | −0.311 | −0.295 | −0.314 | −0.262 | −0.266 | −0.246 |
| RE42 | eV | −0.089 | −0.100 | 0.013 | −0.063 | −0.037 | −0.071 | 0.100 | 0.093 | 0.154 |
| S66x8 | eV | 0.069 | −0.008 | 0.045 | 0.020 | 0.031 | −0.005 | 0.018 | −0.002 | 0.007 |
| W4-11 | eV | 0.520 | 0.528 | −0.226 | −0.099 | −0.071 | −0.081 | −0.320 | −0.307 | −0.297 |
| $a_{\mathrm{lat}}$@SOL62 | Å | 0.059 | 0.017 | 0.010 | 0.014 | 0.029 | 0.004 | 0.014 | 0.007 | 0.018 |
| $E_{\mathrm{coh}}$@SOL62 | eV | 0.138 | −0.153 | −0.009 | 0.078 | 0.137 | −0.053 | 0.001 | −0.108 | −0.059 |
| $B$@SOL62 | GPa | −7.729 | 1.362 | 7.874 | 5.982 | 3.224 | 8.205 | 6.202 | 8.638 | 5.026 |
| $E_{\mathrm{ads}}^{\mathrm{phy}}$@ADS41 | eV | 0.478 | −0.215 | 0.237 | 0.092 | 0.213 | −0.202 | 0.130 | −0.117 | −0.061 |
| $E_{\mathrm{ads}}^{\mathrm{che}}$@ADS41 | eV | −0.210 | −0.382 | −0.244 | −0.409 | −0.351 | −0.493 | −0.226 | −0.311 | −0.263 |

Table ST5: Mean absolute errors for all data sets used within this study. Functionals with '-v' employ the rVV10 methodology. Units are provided.

| Data Set | Unit | PBE | PBE-D3 | MS2 | SCAN | $r^2$SCAN | SCAN-v | MCML | MCML-v | VCML-v |
|---|---|---|---|---|---|---|---|---|---|---|
| DBH24 | eV | 0.356 | 0.365 | 0.272 | 0.317 | 0.301 | 0.320 | 0.268 | 0.272 | 0.250 |
| RE42 | eV | 0.307 | 0.312 | 0.375 | 0.300 | 0.275 | 0.307 | 0.276 | 0.280 | 0.271 |
| S66x8 | eV | 0.069 | 0.015 | 0.046 | 0.032 | 0.036 | 0.017 | 0.024 | 0.018 | 0.019 |
| W4-11 | eV | 0.590 | 0.595 | 0.328 | 0.177 | 0.179 | 0.171 | 0.425 | 0.420 | 0.400 |
| $a_{\mathrm{lat}}$@SOL62 | Å | 0.063 | 0.039 | 0.032 | 0.033 | 0.038 | 0.030 | 0.035 | 0.031 | 0.035 |
| $E_{\mathrm{coh}}$@SOL62 | eV | 0.204 | 0.195 | 0.210 | 0.202 | 0.214 | 0.215 | 0.240 | 0.254 | 0.226 |
| $B$@SOL62 | GPa | 12.733 | 11.792 | 10.326 | 9.676 | 8.620 | 10.617 | 9.948 | 11.003 | 9.051 |
| $E_{\mathrm{ads}}^{\mathrm{phy}}$@ADS41 | eV | 0.479 | 0.240 | 0.260 | 0.210 | 0.234 | 0.239 | 0.183 | 0.159 | 0.127 |
| $E_{\mathrm{ads}}^{\mathrm{che}}$@ADS41 | eV | 0.288 | 0.396 | 0.266 | 0.409 | 0.363 | 0.493 | 0.240 | 0.313 | 0.268 |

## 6.2 All values for all functionals

Table ST6: Systems in the DBH24 data set. Identifiers are provided, which are used in Tab. ST7 and Figs. SF2 (PBE, PBE-D3), SF5 (MS2, MCML), SF8 (SCAN, r$^2$SCAN), and SF11 (all functional using rVV10).

| Identifier | System |
|---|---|
| 1 | $H^\bullet + N_2O \rightarrow OH^\bullet + N_2$ |
| 2 | $H^\bullet + N_2O \leftarrow OH^\bullet + N_2$ |
| 3 | $H^\bullet + ClH \rightarrow H^\bullet + HCl$ |
| 4 | $H^\bullet + ClH \leftarrow H^\bullet + HCl$ |
| 5 | $CH_3^\bullet + FCl \rightarrow CH_3F + Cl^\bullet$ |
| 6 | $CH_3^\bullet + FCl \leftarrow CH_3F + Cl^\bullet$ |
| 7 | $Cl^- + CH_3Cl \rightarrow CH_3Cl + Cl^-$ |
| 8 | $Cl^- + CH_3Cl \leftarrow CH_3Cl + Cl^-$ |
| 9 | $CH_3Cl + F^- \rightarrow CH_3OH + F^-$ |
| 10 | $CH_3Cl + F^- \leftarrow CH_3OH + F^-$ |
| 11 | $OH^- + CH_3F \rightarrow CH_3OH + F^-$ |
| 12 | $OH^- + CH_3F \leftarrow CH_3OH + F^-$ |
| 13 | $H^\bullet + N_2 \rightarrow N_2H^\bullet$ |
| 14 | $H^\bullet + N_2 \leftarrow N_2H^\bullet$ |
| 15 | $H^\bullet + C_2H_4 \rightarrow CH_3CH_2^\bullet$ |
| 16 | $H^\bullet + C_2H_4 \leftarrow CH_3CH_2^\bullet$ |
| 17 | $HCN \rightarrow HNC$ |
| 18 | $HCN \leftarrow HNC$ |
| 19 | $OH^\bullet + CH_4 \rightarrow H_2O + CH_3^\bullet$ |
| 20 | $OH^\bullet + CH_4 \leftarrow H_2O + CH_3^\bullet$ |
| 21 | $H^\bullet + OH^\bullet \rightarrow O^{\bullet\bullet} + H_2$ |
| 22 | $H^\bullet + OH^\bullet \leftarrow O^{\bullet\bullet} + H_2$ |
| 23 | $H^\bullet + H_2S \rightarrow H_2 + HS^\bullet$ |
| 24 | $H^\bullet + H_2S \leftarrow H_2 + HS^\bullet$ |

Table ST7: Barrier heights for the DBH24 data set. Functionals with '-v' employ the rVV10 methodology. The units are eV, and the reference values are provided in the last column. The identifiers are defined in Tab. ST6.

| System | PBE | PBE-D3 | MS2 | SCAN | $r^2$SCAN | SCAN-v | MCML | MCML-v | VCML-v | REF |
|---|---|---|---|---|---|---|---|---|---|---|
| 1 | 0.386 | 0.378 | 0.389 | 0.342 | 0.392 | 0.337 | 0.358 | 0.354 | 0.397 | 0.743 |
| 2 | 2.260 | 2.249 | 3.140 | 2.820 | 2.725 | 2.806 | 3.202 | 3.191 | 3.095 | 3.576 |
| 3 | 0.429 | 0.427 | 0.531 | 0.363 | 0.394 | 0.359 | 0.544 | 0.540 | 0.556 | 0.781 |
| 4 | 0.429 | 0.427 | 0.531 | 0.363 | 0.394 | 0.359 | 0.544 | 0.540 | 0.556 | 0.781 |
| 5 | −0.246 | −0.278 | −0.157 | −0.140 | −0.144 | −0.151 | −0.147 | −0.158 | −0.141 | 0.293 |
| 6 | 1.731 | 1.708 | 1.869 | 1.929 | 1.915 | 1.920 | 1.804 | 1.796 | 1.828 | 2.602 |
| 7 | 0.330 | 0.332 | 0.334 | 0.323 | 0.362 | 0.320 | 0.426 | 0.423 | 0.425 | 0.582 |
| 8 | 0.330 | 0.332 | 0.334 | 0.323 | 0.362 | 0.320 | 0.426 | 0.423 | 0.425 | 0.582 |
| 9 | 0.004 | 0.006 | −0.046 | −0.040 | −0.008 | −0.041 | 0.024 | 0.022 | 0.029 | 0.149 |
| 10 | 0.860 | 0.863 | 0.935 | 1.005 | 0.993 | 1.002 | 0.948 | 0.945 | 0.959 | 1.276 |
| 11 | −0.278 | −0.302 | −0.396 | −0.415 | −0.303 | −0.369 | −0.421 | −0.431 | −0.297 | −0.106 |
| 12 | 0.528 | 0.505 | 0.438 | 0.479 | 0.529 | 0.466 | 0.446 | 0.435 | 0.489 | 0.766 |
| 13 | 0.185 | 0.183 | 0.238 | 0.135 | 0.152 | 0.131 | 0.261 | 0.259 | 0.295 | 0.623 |
| 14 | 0.438 | 0.436 | 0.505 | 0.465 | 0.456 | 0.464 | 0.458 | 0.458 | 0.442 | 0.460 |
| 15 | −0.008 | −0.023 | −0.020 | −0.202 | −0.153 | −0.206 | 0.003 | −0.000 | 0.014 | 0.075 |
| 16 | 1.754 | 1.744 | 1.917 | 1.875 | 1.879 | 1.875 | 1.882 | 1.882 | 1.864 | 1.810 |
| 17 | 1.974 | 1.976 | 1.978 | 2.002 | 1.989 | 2.001 | 1.810 | 1.810 | 1.827 | 2.084 |
| 18 | 1.354 | 1.355 | 1.336 | 1.423 | 1.401 | 1.422 | 1.210 | 1.210 | 1.218 | 1.423 |
| 19 | −0.234 | −0.258 | 0.136 | −0.062 | −0.035 | −0.072 | 0.131 | 0.124 | 0.126 | 0.290 |
| 20 | 0.379 | 0.355 | 0.302 | 0.493 | 0.556 | 0.483 | 0.282 | 0.275 | 0.358 | 0.850 |
| 21 | 0.125 | 0.120 | 0.192 | 0.096 | 0.096 | 0.093 | 0.265 | 0.263 | 0.237 | 0.464 |
| 22 | −0.057 | −0.061 | 0.211 | 0.119 | 0.115 | 0.115 | 0.137 | 0.134 | 0.214 | 0.568 |
| 23 | −0.046 | −0.055 | 0.037 | −0.114 | −0.113 | −0.117 | 0.037 | 0.034 | 0.052 | 0.156 |
| 24 | 0.416 | 0.406 | 0.610 | 0.526 | 0.533 | 0.520 | 0.661 | 0.657 | 0.705 | 0.750 |

Table ST8: Systems in the RE42 data set. Identifiers are provided, which are used in Tab. ST9 and Figs. SF2 (PBE, PBE-D3), SF5 (MS2, MCML), SF8 (SCAN, r$^2$SCAN), and SF11 (all functionals using rVV10).

| Identifier | System |
|---|---|
| 1 | 1-4-cyclo-$C_6H_8$+2$H_2$ $\rightarrow$ cyclo-$C_6H_{12}$ |
| 2 | $CH_4$+$NH_3$ $\rightarrow$ HCN+3$H_2$ |
| 3 | $CO_2$+3$H_2$ $\rightarrow$ $CH_3OH$+$H_2O$ |
| 4 | $CH_4$+2$Cl_2$ $\rightarrow$ $CCl_4$+2$H_2$ |
| 5 | $O_2^{\bullet\bullet}$+$H_2$ $\rightarrow$ 2$OH^{\bullet}$ |
| 6 | $CH_4$+$CO_2$ $\rightarrow$ 2CO+2$H_2$ |
| 7 | CO+$H_2O$ $\rightarrow$ $CO_2$+$H_2$ |
| 8 | $CH_4$+$H_2O$ $\rightarrow$ $CH_3OH$+$H_2$ |
| 9 | CO+2$H_2$ $\rightarrow$ $CH_3OH$ |
| 10 | $CH_2OCH_2$ + $H_2$ $\rightarrow$ $C_2H_4$+$H_2O$ |
| 11 | CO+3$H_2$ $\rightarrow$ $CH_4$+$H_2O$ |
| 12 | 2$N_2$+$O_2^{\bullet\bullet}$ $\rightarrow$ 2$N_2O^{\bullet}$ |
| 13 | $O_2^{\bullet\bullet}$+2$H_2$ $\rightarrow$ 2$H_2O$ |
| 14 | $CO_2$+4$H_2$ $\rightarrow$ $CH_4$+2$H_2O$ |
| 15 | 1-4-cyclo-$C_6H_8$ $\rightarrow$ 1-3-cyclo-$C_6H_8$ |
| 16 | 2CO+$O_2^{\bullet\bullet}$ $\rightarrow$ 2$CO_2$ |
| 17 | $C_6H_6$+$H_2$ $\rightarrow$ 1-4-cyclo-$C_6H_8$ |
| 18 | $CH_4$+2$F_2$ $\rightarrow$ $CF_4$+2$H_2$ |
| 19 | 3$O_2^{\bullet\bullet}$ $\rightarrow$ 2$O_3$ |
| 20 | $N_2$+2$O_2^{\bullet\bullet}$ $\rightarrow$ 2$NO_2$ |
| 21 | $C_3H_4$-C3v+$H_2$ $\rightarrow$ $C_3H_6$ |
| 22 | $N_2$+3$H_2$ $\rightarrow$ 3$NH_3$ |
| 23 | $CH_4$+CO+$H_2$ $\rightarrow$ $C_2H_5OH$ |
| 24 | $CH_3NH_2$+$H_2$ $\rightarrow$ $CH_4$+$NH_3$ |
| 25 | $N_2$+2$H_2$ $\rightarrow$ $N_2H_4$ |
| 26 | $O_2^{\bullet\bullet}$+4HCl $\rightarrow$ 2$Cl_2$ 2$H_2O$ |
| 27 | $C_3H_4$-D2d+2$H_2$ $\rightarrow$ $C_3H_8$ |
| 28 | $C_3H_6$+$H_2$ $\rightarrow$ $C_3H_8$ |
| 29 | CO+$H_2O$ $\rightarrow$ HCOOH |
| 30 | $C_2H_5OH$ $\rightarrow$ $CH_3OCH_3$ |
| 31 | $C_2H_4$+2$H_2$ $\rightarrow$ $C_2H_4$ |
| 32 | CO+9$H_2$ $\rightarrow$ trans-$C_4H_{10}$+4$H_2O$ |
| 33 | $H_2CCO$+$H_2$ $\rightarrow$ $C_2H_4$+$H_2O$ |
| 34 | iso-$C_4H_{10}$ $\rightarrow$ trans-$C_4H_{10}$ |
| 35 | $N_2$+$O_2^{\bullet\bullet}$ $\rightarrow$ 2$NO^{\bullet}$ |
| 36 | $CH_4$+$CO_2$ $\rightarrow$ $CH_3COOH$ |
| 37 | 2$OH^{\bullet}$+$H_2$ $\rightarrow$ 2$H_2O$ |
| 38 | $H_2$+$O_2^{\bullet\bullet}$ $\rightarrow$ $H_2O_2$ |
| 39 | $CH_3CH_2SH$+$H_2$ $\rightarrow$ $H_2S$+$C_2H_6$ |
| 40 | 2$CH_3OH$+$O_2^{\bullet\bullet}$ $\rightarrow$ 2$CO_2$+4$H_2$ |
| 41 | 2CO+2$NO^{\bullet}$ $\rightarrow$ 2$CO_2$+$N_2$ |
| 42 | $SO_2$+3$H_2$ $\rightarrow$ $H_2S$+2$H_2O$ |

Table ST9: Reaction energies for the RE42 data set. Functionals with '-v' employ the rVV10 methodology. The units are eV, and the reference values are provided in the last column. The identifiers are defined in Tab. ST8.

| System | PBE | PBE-D3 | MS2 | SCAN | $r^2$SCAN | SCAN-v | MCML | MCML-v | VCML-v | REF |
|---|---|---|---|---|---|---|---|---|---|---|
| 1 | −2.884 | −2.971 | −3.299 | −3.122 | −3.027 | −3.150 | −3.093 | −3.115 | −2.968 | −2.939 |
| 2 | 3.573 | 3.573 | 3.715 | 3.627 | 3.596 | 3.633 | 3.461 | 3.464 | 3.223 | 3.320 |
| 3 | −1.175 | −1.188 | −1.482 | −1.303 | −1.183 | −1.310 | −1.324 | −1.330 | −1.013 | −1.171 |
| 4 | 0.376 | 0.347 | 0.540 | 0.154 | 0.173 | 0.107 | 0.275 | 0.237 | 0.099 | 0.189 |
| 5 | 1.158 | 1.158 | 0.474 | 0.643 | 0.798 | 0.647 | 0.433 | 0.439 | 0.668 | 0.738 |
| 6 | 3.888 | 3.893 | 3.661 | 3.801 | 3.790 | 3.812 | 3.228 | 3.234 | 3.117 | 3.110 |
| 7 | −0.718 | −0.720 | −0.517 | −0.642 | −0.665 | −0.648 | −0.392 | −0.396 | −0.522 | −0.305 |
| 8 | 1.278 | 1.265 | 1.145 | 1.213 | 1.278 | 1.206 | 1.119 | 1.112 | 1.060 | 1.329 |
| 9 | −1.893 | −1.908 | −1.999 | −1.946 | −1.848 | −1.958 | −1.716 | −1.726 | −1.535 | −1.476 |
| 10 | −1.354 | −1.341 | −1.110 | −1.294 | −1.358 | −1.283 | −1.109 | −1.097 | −1.053 | −1.559 |
| 11 | −3.170 | −3.172 | −3.144 | −3.159 | −3.125 | −3.164 | −2.836 | −2.838 | −2.595 | −2.805 |
| 12 | 0.355 | 0.349 | 1.348 | 0.933 | 0.790 | 0.920 | 1.509 | 1.499 | 1.432 | 1.567 |
| 13 | −5.043 | −5.043 | −4.721 | −5.044 | −4.987 | −5.044 | −4.659 | −4.659 | −4.523 | −5.448 |
| 14 | −2.453 | −2.452 | −2.627 | −2.517 | −2.460 | −2.517 | −2.443 | −2.442 | −2.073 | −2.500 |
| 15 | 0.015 | 0.021 | 0.011 | 0.010 | 0.017 | 0.012 | 0.005 | 0.006 | 0.011 | −0.013 |
| 16 | −6.478 | −6.483 | −5.755 | −6.329 | −6.317 | −6.339 | −5.443 | −5.451 | −5.567 | −6.058 |
| 17 | 0.131 | 0.100 | −0.052 | 0.083 | 0.165 | 0.072 | 0.021 | 0.012 | 0.096 | −0.011 |
| 18 | −7.892 | −7.904 | −7.038 | −8.454 | −8.385 | −8.480 | −7.038 | −7.062 | −7.439 | −8.595 |
| 19 | 2.568 | 2.565 | 3.086 | 3.622 | 3.604 | 3.606 | 2.966 | 2.953 | 2.961 | 2.920 |
| 20 | −0.380 | −0.383 | 0.330 | 0.199 | 0.113 | 0.184 | 0.462 | 0.451 | 0.384 | 0.622 |
| 21 | −2.082 | −2.102 | −2.362 | −2.159 | −2.118 | −2.168 | −2.227 | −2.234 | −2.140 | −1.995 |
| 22 | −2.128 | −2.129 | −1.938 | −2.111 | −2.095 | −2.116 | −1.733 | −1.738 | −1.451 | −1.677 |
| 23 | −1.292 | −1.337 | −1.381 | −1.384 | −1.270 | −1.409 | −1.203 | −1.224 | −1.063 | −0.907 |
| 24 | −1.142 | −1.127 | −1.098 | −1.118 | −1.154 | −1.110 | −1.056 | −1.047 | −0.992 | −1.146 |
| 25 | −0.126 | −0.137 | −0.039 | −0.075 | −0.048 | −0.089 | 0.148 | 0.138 | 0.356 | 0.408 |
| 26 | −1.365 | −1.365 | −1.154 | −1.157 | −1.112 | −1.173 | −1.276 | −1.288 | −1.225 | −1.515 |
| 27 | −3.542 | −3.587 | −3.978 | −3.748 | −3.654 | −3.767 | −3.734 | −3.748 | −3.597 | −3.640 |
| 28 | −1.588 | −1.613 | −1.768 | −1.688 | −1.644 | −1.697 | −1.667 | −1.674 | −1.602 | −1.576 |
| 29 | −0.872 | −0.886 | −0.884 | −0.907 | −0.823 | −0.921 | −0.727 | −0.738 | −0.731 | −0.393 |
| 30 | 0.499 | 0.500 | 0.357 | 0.453 | 0.499 | 0.453 | 0.429 | 0.429 | 0.406 | 0.535 |
| 31 | −2.256 | −2.263 | −2.504 | −2.309 | −2.275 | −2.316 | −2.355 | −2.356 | −2.269 | −2.097 |
| 32 | −10.395 | −10.502 | −10.246 | −10.428 | −10.237 | −10.488 | −9.270 | −9.317 | −8.453 | −9.003 |
| 33 | −1.719 | −1.719 | −1.892 | −1.747 | −1.725 | −1.747 | −1.743 | −1.739 | −1.563 | −1.925 |
| 34 | 0.033 | 0.046 | 0.044 | 0.057 | 0.056 | 0.061 | 0.061 | 0.064 | 0.058 | 0.077 |
| 35 | 1.890 | 1.890 | 1.866 | 1.921 | 1.969 | 1.922 | 1.896 | 1.896 | 1.866 | 1.881 |
| 36 | 0.259 | 0.218 | 0.070 | 0.085 | 0.204 | 0.063 | −0.020 | −0.039 | 0.075 | 0.285 |
| 37 | −6.201 | −6.201 | −5.196 | −5.686 | −5.785 | −5.691 | −5.092 | −5.098 | −5.191 | −6.186 |
| 38 | −1.522 | −1.527 | −1.562 | −1.463 | −1.384 | −1.469 | −1.571 | −1.575 | −1.417 | −1.680 |
| 39 | −0.748 | −0.722 | −0.775 | −0.721 | −0.728 | −0.706 | −0.676 | −0.664 | −0.619 | −0.710 |
| 40 | −2.693 | −2.667 | −1.757 | −2.438 | −2.622 | −2.423 | −2.010 | −1.999 | −2.496 | −3.106 |
| 41 | −8.368 | −8.373 | −7.621 | −8.249 | −8.286 | −8.261 | −7.339 | −7.347 | −7.433 | −7.939 |
| 42 | −2.308 | −2.305 | −2.197 | −2.275 | −2.311 | −2.266 | −2.099 | −2.092 | −1.837 | −2.620 |

Table ST10: Systems in the S66x8 data set. Identifiers are provided, which are used in Tabs. ST11 (PBE), ST12 (PBE-D3), ST13 (MS2), ST14 (SCAN), ST15 ($r^2$SCAN), ST16 (SCAN-v), ST17 (MCML), ST18 (MCML-v), ST19 (VCML-v), and ST20 (Reference values) as well as Figs. SF2 (PBE, PBE-D3), SF5 (MS2, MCML), SF8 (SCAN, $r^2$SCAN), and SF11 (all functionals using rVV10).

| Identifier | System |
|---|---|
| 1 | $AcNH_2 \cdots AcNH_2$ |
| 2 | $AcNH_2 \cdots$ Uracil |
| 3 | $AcOH \cdots AcOH$ |
| 4 | $AcOH \cdots$ Uracil |
| 5 | $C_6H_6 \cdots AcNH_2$ |
| 6 | $C_6H_6 \cdots AcOH$ (∥) |
| 7 | $C_6H_6 \cdots AcOH$ (⊥) |
| 8 | $C_6H_6 \cdots C_6H_6$ (∥) |
| 9 | $C_6H_6 \cdots C_6H_6$ (⊥) |
| 10 | $C_6H_6 \cdots$ Cyclo-$C_5H_{10}$ |
| 11 | $C_6H_6 \cdots C_2H_4$ |
| 12 | $C_6H_6 \cdots C_2H_2$ |
| 13 | $C_6H_6 \cdots CH_3NH_2$ |
| 14 | $C_6H_6 \cdots CH_3OH$ |
| 15 | $C_6H_6 \cdots$ Neo-$C_5H_{12}$ |
| 16 | $C_6H_6 \cdots$ Peptide |
| 17 | $C_6H_6 \cdots$ Pyridine (∥) |
| 18 | $C_6H_6 \cdots$ Pyridine (⊥) |
| 19 | $C_6H_6 \cdots$ Uracil |
| 20 | $C_6H_6 \cdots H_2O$ |
| 21 | Cyclo-$C_5H_{10} \cdots$ Cyclo-$C_5H_{10}$ |
| 22 | Cyclo-$C_5H_{10} \cdots$ Neo-$C_5H_{12}$ |
| 23 | $C_2H_4 \cdots C_5H_{12}$ |
| 24 | $C_2H_2 \cdots AcOH$ |
| 25 | $C_2H_2 \cdots C_2H_2$ (⊥) |
| 26 | $C_2H_2 \cdots C_5H_{12}$ |
| 27 | $C_2H_2 \cdots H_2O$ |
| 28 | $CH_3NH_2 \cdots CH_3NH_2$ |
| 29 | $CH_3NH_2 \cdots CH_3OH$ |
| 30 | $CH_3NH_2 \cdots$ Peptide |
| 31 | $CH_3NH_2 \cdots$ Pyridine |
| 32 | $CH_3NH_2 \cdots H_2O$ |
| 33 | $CH_3OH \cdots CH_3NH_2$ |
| 34 | $CH_3OH \cdots CH_3OH$ |
| 35 | $CH_3OH \cdots$ Peptide |
| 36 | $CH_3OH \cdots$ Pyridine |
| 37 | $CH_3OH \cdots H_2O$ |
| 38 | Neo-$C_5H_{12} \cdots$ Neo-$C_5H_{12}$ |
| 39 | Neo-$C_5H_{12} \cdots C_5H_{12}$ |
| 40 | $C_5H_{12} \cdots AcNH_2$ |
| 41 | $C_5H_{12} \cdots AcOH$ |
| 42 | $C_5H_{12} \cdots C_5H_{12}$ |
| 43 | Peptide $\cdots C_2H_4$ |
| 44 | Peptide $\cdots CH_3NH_2$ |
| 45 | Peptide $\cdots CH_3OH$ |
| 46 | Peptide $\cdots C_5H_{12}$ |
| 47 | Peptide $\cdots$ Peptide |
| 48 | Peptide $\cdots H_2O$ |
| 49 | Pyridine $\cdots C_2H_4$ |
| 50 | Pyridine $\cdots C_2H_2$ |
| 51 | Pyridine $\cdots$ Pyridine (in-plane) |
| 52 | Pyridine $\cdots$ Pyridine (∥) |
| 53 | Pyridine $\cdots$ Pyridine (⊥) |
| 54 | Pyridine $\cdots$ Uracil |
| 55 | Uracil $\cdots$ Cyclopentane |
| 56 | Uracil $\cdots C_2H_4$ |
| 57 | Uracil $\cdots C_2H_2$ |
| 58 | Uracil $\cdots$ Neo-$C_5H_{12}$ |
| 59 | Uracil $\cdots C_5H_{12}$ |
| 60 | Uracil $\cdots$ Uracil (in-plane) |
| 61 | Uracil $\cdots$ Uracil (∥) |
| 62 | $H_2O \cdots CH_3NH_2$ |
| 63 | $H_2O \cdots CH_3OH$ |
| 64 | $H_2O \cdots$ Peptide |
| 65 | $H_2O \cdots$ Pyridine |
| 66 | $H_2O \cdots H_2O$ |

Table ST11: Interaction energies for the S66x8 data set using PBE. The units are eV. Distances in the first row are relative to the equilibrium distance. The identifiers are defined in Tab. ST10.

| System | 0.900 | 0.950 | 1.000 | 1.050 | 1.100 | 1.250 | 1.500 | 2.000 |
|---|---|---|---|---|---|---|---|---|
| 1 | −0.611 | −0.653 | −0.660 | −0.645 | −0.617 | −0.500 | −0.323 | −0.121 |
| 2 | −0.722 | −0.769 | −0.778 | −0.765 | −0.736 | −0.612 | −0.411 | −0.187 |
| 3 | −0.772 | −0.820 | −0.825 | −0.802 | −0.764 | −0.611 | −0.382 | −0.148 |
| 4 | −0.756 | −0.803 | −0.810 | −0.792 | −0.758 | −0.617 | −0.399 | −0.167 |
| 5 | −0.058 | −0.089 | −0.103 | −0.108 | −0.106 | −0.086 | −0.050 | −0.014 |
| 6 | 0.078 | 0.011 | −0.025 | −0.042 | −0.049 | −0.043 | −0.022 | −0.006 |
| 7 | −0.047 | −0.087 | −0.105 | −0.111 | −0.109 | −0.088 | −0.051 | −0.017 |
| 8 | 0.098 | 0.032 | −0.003 | −0.021 | −0.029 | −0.029 | −0.015 | −0.004 |
| 9 | 0.276 | 0.149 | 0.078 | 0.038 | 0.017 | −0.001 | 0.001 | 0.002 |
| 10 | 0.146 | 0.064 | 0.016 | −0.009 | −0.021 | −0.025 | −0.012 | −0.002 |
| 11 | 0.135 | 0.074 | 0.040 | 0.021 | 0.011 | 0.003 | 0.004 | 0.003 |
| 12 | 0.016 | −0.031 | −0.053 | −0.061 | −0.062 | −0.049 | −0.026 | −0.008 |
| 13 | 0.031 | −0.012 | −0.036 | −0.048 | −0.052 | −0.044 | −0.024 | −0.007 |
| 14 | −0.025 | −0.064 | −0.084 | −0.091 | −0.092 | −0.076 | −0.045 | −0.016 |
| 15 | 0.104 | 0.040 | 0.004 | −0.014 | −0.022 | −0.024 | −0.012 | −0.002 |
| 16 | 0.053 | −0.030 | −0.072 | −0.091 | −0.096 | −0.083 | −0.049 | −0.018 |
| 17 | 0.078 | 0.012 | −0.023 | −0.040 | −0.046 | −0.043 | −0.024 | −0.008 |
| 18 | 0.262 | 0.129 | 0.056 | 0.018 | −0.002 | −0.016 | −0.007 | −0.001 |
| 19 | 0.217 | 0.091 | 0.020 | −0.018 | −0.036 | −0.041 | −0.019 | −0.001 |
| 20 | −0.052 | −0.079 | −0.089 | −0.090 | −0.087 | −0.068 | −0.039 | −0.014 |
| 21 | 0.087 | 0.035 | 0.002 | −0.015 | −0.022 | −0.022 | −0.010 | −0.001 |
| 22 | 0.092 | 0.037 | 0.007 | −0.008 | −0.016 | −0.018 | −0.009 | −0.001 |
| 23 | 0.043 | 0.010 | −0.007 | −0.015 | −0.019 | −0.017 | −0.007 | −0.001 |
| 24 | −0.159 | −0.179 | −0.183 | −0.177 | −0.166 | −0.124 | −0.068 | −0.021 |
| 25 | −0.038 | −0.050 | −0.054 | −0.053 | −0.049 | −0.035 | −0.017 | −0.005 |
| 26 | 0.054 | 0.015 | −0.005 | −0.015 | −0.020 | −0.018 | −0.008 | −0.001 |
| 27 | −0.105 | −0.115 | −0.117 | −0.113 | −0.107 | −0.082 | −0.049 | −0.018 |
| 28 | −0.108 | −0.129 | −0.136 | −0.135 | −0.128 | −0.099 | −0.048 | −0.014 |
| 29 | −0.082 | −0.096 | −0.100 | −0.098 | −0.093 | −0.071 | −0.040 | −0.014 |
| 30 | −0.114 | −0.140 | −0.151 | −0.152 | −0.148 | −0.103 | −0.046 | −0.015 |
| 31 | −0.033 | −0.063 | −0.078 | −0.084 | −0.085 | −0.071 | −0.043 | −0.014 |
| 32 | −0.300 | −0.316 | −0.315 | −0.304 | −0.286 | −0.223 | −0.134 | −0.049 |
| 33 | −0.297 | −0.317 | −0.319 | −0.309 | −0.293 | −0.230 | −0.140 | −0.052 |
| 34 | −0.208 | −0.225 | −0.227 | −0.221 | −0.209 | −0.164 | −0.100 | −0.039 |
| 35 | −0.294 | −0.315 | −0.319 | −0.311 | −0.297 | −0.240 | −0.142 | −0.043 |
| 36 | −0.287 | −0.306 | −0.308 | −0.298 | −0.283 | −0.223 | −0.136 | −0.053 |
| 37 | −0.201 | −0.214 | −0.214 | −0.206 | −0.195 | −0.152 | −0.093 | −0.037 |
| 38 | 0.042 | 0.013 | −0.002 | −0.011 | −0.014 | −0.013 | −0.006 | −0.001 |
| 39 | 0.085 | 0.030 | 0.001 | −0.013 | −0.019 | −0.019 | −0.009 | −0.001 |
| 40 | 0.040 | −0.000 | −0.022 | −0.034 | −0.039 | −0.036 | −0.019 | −0.004 |
| 41 | 0.038 | 0.009 | −0.009 | −0.019 | −0.024 | −0.025 | −0.011 | −0.001 |
| 42 | 0.124 | 0.052 | 0.012 | −0.010 | −0.021 | −0.026 | −0.013 | −0.001 |
| 43 | −0.001 | −0.031 | −0.047 | −0.053 | −0.055 | −0.045 | −0.023 | −0.005 |
| 44 | −0.237 | −0.262 | −0.270 | −0.267 | −0.257 | −0.210 | −0.135 | −0.057 |
| 45 | −0.172 | −0.196 | −0.204 | −0.203 | −0.196 | −0.162 | −0.107 | −0.049 |
| 46 | 0.073 | 0.021 | −0.009 | −0.026 | −0.035 | −0.037 | −0.019 | −0.003 |
| 47 | −0.245 | −0.273 | −0.283 | −0.282 | −0.274 | −0.231 | −0.158 | −0.066 |
| 48 | −0.173 | −0.190 | −0.194 | −0.191 | −0.183 | −0.149 | −0.098 | −0.046 |
| 49 | 0.107 | 0.054 | 0.023 | 0.006 | −0.003 | −0.008 | −0.002 | 0.001 |
| 50 | −0.146 | −0.159 | −0.160 | −0.155 | −0.146 | −0.112 | −0.066 | −0.023 |
| 51 | −0.034 | −0.084 | −0.110 | −0.110 | −0.101 | −0.066 | −0.030 | −0.006 |
| 52 | 0.055 | −0.001 | −0.030 | −0.045 | −0.051 | −0.047 | −0.027 | −0.009 |
| 53 | 0.237 | 0.112 | 0.042 | 0.004 | −0.015 | −0.027 | −0.015 | −0.004 |
| 54 | 0.219 | 0.053 | −0.030 | −0.069 | −0.085 | −0.077 | −0.043 | −0.015 |
| 55 | 0.147 | 0.063 | 0.016 | −0.008 | −0.020 | −0.025 | −0.012 | −0.002 |
| 56 | 0.067 | 0.011 | −0.020 | −0.035 | −0.042 | −0.039 | −0.022 | −0.006 |
| 57 | 0.036 | −0.020 | −0.049 | −0.062 | −0.065 | −0.054 | −0.029 | −0.008 |
| 58 | 0.098 | 0.030 | −0.006 | −0.024 | −0.032 | −0.030 | −0.015 | −0.003 |
| 59 | 0.143 | 0.060 | 0.013 | −0.013 | −0.028 | −0.029 | −0.011 | −0.001 |
| 60 | −0.632 | −0.678 | −0.687 | −0.673 | −0.643 | −0.521 | −0.331 | −0.134 |
| 61 | 0.078 | −0.051 | −0.119 | −0.150 | −0.160 | −0.139 | −0.082 | −0.029 |
| 62 | −0.308 | −0.318 | −0.314 | −0.300 | −0.282 | −0.217 | −0.130 | −0.048 |
| 63 | −0.216 | −0.230 | −0.230 | −0.221 | −0.208 | −0.162 | −0.098 | −0.038 |
| 64 | −0.306 | −0.322 | −0.323 | −0.313 | −0.298 | −0.239 | −0.153 | −0.057 |
| 65 | −0.292 | −0.304 | −0.301 | −0.289 | −0.271 | −0.210 | −0.127 | −0.049 |
| 66 | −0.208 | −0.218 | −0.216 | −0.207 | −0.195 | −0.150 | −0.091 | −0.036 |

Table ST12: Interaction energies for the S66x8 data set using PBE-D3. The units are eV. Distances in the first row are relative to the equilibrium distance. The identifiers are defined in Tab. ST10.

| System | 0.900 | 0.950 | 1.000 | 1.050 | 1.100 | 1.250 | 1.500 | 2.000 |
|---|---|---|---|---|---|---|---|---|
| 1 | −0.690 | −0.730 | −0.734 | −0.716 | −0.685 | −0.560 | −0.365 | −0.133 |
| 2 | −0.812 | −0.856 | −0.863 | −0.846 | −0.814 | −0.680 | −0.462 | −0.207 |
| 3 | −0.840 | −0.887 | −0.891 | −0.868 | −0.828 | −0.669 | −0.428 | −0.167 |
| 4 | −0.839 | −0.884 | −0.889 | −0.869 | −0.832 | −0.682 | −0.450 | −0.188 |
| 5 | −0.163 | −0.187 | −0.195 | −0.193 | −0.184 | −0.141 | −0.078 | −0.021 |
| 6 | −0.084 | −0.137 | −0.157 | −0.159 | −0.151 | −0.110 | −0.051 | −0.012 |
| 7 | −0.162 | −0.195 | −0.206 | −0.204 | −0.194 | −0.147 | −0.081 | −0.024 |
| 8 | −0.041 | −0.096 | −0.118 | −0.124 | −0.120 | −0.089 | −0.042 | −0.010 |
| 9 | 0.044 | −0.058 | −0.104 | −0.118 | −0.117 | −0.080 | −0.028 | −0.004 |
| 10 | −0.066 | −0.129 | −0.156 | −0.161 | −0.154 | −0.109 | −0.048 | −0.009 |
| 11 | 0.002 | −0.045 | −0.064 | −0.068 | −0.065 | −0.042 | −0.013 | −0.000 |
| 12 | −0.062 | −0.105 | −0.122 | −0.124 | −0.118 | −0.088 | −0.043 | −0.012 |
| 13 | −0.101 | −0.135 | −0.148 | −0.148 | −0.139 | −0.101 | −0.048 | −0.012 |
| 14 | −0.148 | −0.180 | −0.191 | −0.190 | −0.181 | −0.138 | −0.076 | −0.023 |
| 15 | −0.074 | −0.120 | −0.136 | −0.137 | −0.129 | −0.090 | −0.040 | −0.009 |
| 16 | −0.135 | −0.203 | −0.230 | −0.232 | −0.221 | −0.165 | −0.087 | −0.027 |
| 17 | −0.060 | −0.115 | −0.138 | −0.142 | −0.137 | −0.103 | −0.051 | −0.015 |
| 18 | 0.030 | −0.080 | −0.128 | −0.142 | −0.140 | −0.099 | −0.038 | −0.007 |
| 19 | −0.060 | −0.163 | −0.208 | −0.221 | −0.214 | −0.155 | −0.068 | −0.012 |
| 20 | −0.130 | −0.152 | −0.157 | −0.152 | −0.142 | −0.104 | −0.056 | −0.018 |
| 21 | −0.100 | −0.137 | −0.153 | −0.152 | −0.143 | −0.101 | −0.046 | −0.010 |
| 22 | −0.082 | −0.118 | −0.131 | −0.130 | −0.122 | −0.087 | −0.041 | −0.009 |
| 23 | −0.074 | −0.096 | −0.103 | −0.102 | −0.096 | −0.068 | −0.030 | −0.006 |
| 24 | −0.213 | −0.231 | −0.233 | −0.225 | −0.211 | −0.160 | −0.088 | −0.026 |
| 25 | −0.065 | −0.077 | −0.079 | −0.076 | −0.070 | −0.050 | −0.024 | −0.006 |
| 26 | −0.049 | −0.079 | −0.089 | −0.090 | −0.084 | −0.057 | −0.024 | −0.005 |
| 27 | −0.124 | −0.134 | −0.136 | −0.131 | −0.124 | −0.095 | −0.055 | −0.020 |
| 28 | −0.176 | −0.194 | −0.197 | −0.191 | −0.181 | −0.139 | −0.066 | −0.018 |
| 29 | −0.142 | −0.152 | −0.152 | −0.146 | −0.137 | −0.101 | −0.055 | −0.018 |
| 30 | −0.215 | −0.236 | −0.242 | −0.238 | −0.228 | −0.156 | −0.068 | −0.020 |
| 31 | −0.145 | −0.167 | −0.175 | −0.174 | −0.167 | −0.133 | −0.076 | −0.023 |
| 32 | −0.342 | −0.357 | −0.354 | −0.341 | −0.321 | −0.252 | −0.152 | −0.055 |
| 33 | −0.363 | −0.380 | −0.378 | −0.364 | −0.343 | −0.270 | −0.164 | −0.060 |
| 34 | −0.254 | −0.269 | −0.270 | −0.261 | −0.247 | −0.196 | −0.120 | −0.045 |
| 35 | −0.365 | −0.383 | −0.384 | −0.374 | −0.357 | −0.291 | −0.175 | −0.050 |
| 36 | −0.353 | −0.368 | −0.365 | −0.352 | −0.332 | −0.263 | −0.162 | −0.062 |
| 37 | −0.228 | −0.240 | −0.238 | −0.230 | −0.217 | −0.171 | −0.105 | −0.041 |
| 38 | −0.093 | −0.106 | −0.106 | −0.100 | −0.091 | −0.062 | −0.028 | −0.006 |
| 39 | −0.093 | −0.130 | −0.140 | −0.137 | −0.127 | −0.088 | −0.040 | −0.009 |
| 40 | −0.136 | −0.162 | −0.170 | −0.167 | −0.158 | −0.118 | −0.058 | −0.014 |
| 41 | −0.122 | −0.139 | −0.143 | −0.141 | −0.134 | −0.102 | −0.046 | −0.009 |
| 42 | −0.115 | −0.167 | −0.188 | −0.190 | −0.181 | −0.133 | −0.062 | −0.014 |
| 43 | −0.109 | −0.132 | −0.139 | −0.137 | −0.131 | −0.099 | −0.047 | −0.009 |
| 44 | −0.332 | −0.352 | −0.354 | −0.345 | −0.329 | −0.267 | −0.169 | −0.068 |
| 45 | −0.255 | −0.273 | −0.277 | −0.271 | −0.260 | −0.213 | −0.137 | −0.058 |
| 46 | −0.143 | −0.179 | −0.193 | −0.194 | −0.187 | −0.144 | −0.067 | −0.014 |
| 47 | −0.365 | −0.387 | −0.391 | −0.383 | −0.369 | −0.309 | −0.207 | −0.080 |
| 48 | −0.216 | −0.230 | −0.232 | −0.226 | −0.216 | −0.175 | −0.113 | −0.050 |
| 49 | −0.022 | −0.064 | −0.082 | −0.086 | −0.082 | −0.057 | −0.022 | −0.003 |
| 50 | −0.188 | −0.197 | −0.196 | −0.188 | −0.177 | −0.136 | −0.079 | −0.027 |
| 51 | −0.105 | −0.152 | −0.172 | −0.166 | −0.150 | −0.099 | −0.045 | −0.010 |
| 52 | −0.077 | −0.123 | −0.143 | −0.148 | −0.144 | −0.112 | −0.058 | −0.017 |
| 53 | 0.007 | −0.098 | −0.145 | −0.160 | −0.157 | −0.115 | −0.049 | −0.011 |
| 54 | −0.056 | −0.197 | −0.254 | −0.266 | −0.255 | −0.181 | −0.085 | −0.024 |
| 55 | −0.090 | −0.153 | −0.177 | −0.180 | −0.172 | −0.123 | −0.055 | −0.012 |
| 56 | −0.080 | −0.124 | −0.141 | −0.142 | −0.136 | −0.099 | −0.048 | −0.012 |
| 57 | −0.083 | −0.129 | −0.148 | −0.151 | −0.145 | −0.107 | −0.052 | −0.013 |
| 58 | −0.103 | −0.150 | −0.166 | −0.165 | −0.155 | −0.108 | −0.049 | −0.011 |
| 59 | −0.124 | −0.185 | −0.209 | −0.212 | −0.200 | −0.132 | −0.053 | −0.010 |
| 60 | −0.734 | −0.776 | −0.782 | −0.763 | −0.729 | −0.595 | −0.385 | −0.154 |
| 61 | −0.237 | −0.344 | −0.387 | −0.392 | −0.376 | −0.285 | −0.151 | −0.046 |
| 62 | −0.344 | −0.353 | −0.346 | −0.331 | −0.310 | −0.240 | −0.144 | −0.052 |
| 63 | −0.250 | −0.263 | −0.262 | −0.252 | −0.238 | −0.187 | −0.113 | −0.042 |
| 64 | −0.354 | −0.370 | −0.369 | −0.358 | −0.341 | −0.278 | −0.181 | −0.065 |
| 65 | −0.335 | −0.345 | −0.339 | −0.324 | −0.304 | −0.237 | −0.144 | −0.054 |
| 66 | −0.228 | −0.237 | −0.235 | −0.225 | −0.212 | −0.166 | −0.101 | −0.039 |

Table ST13: Interaction energies for the S66x8 data set using MS2. The units are eV. Distances in the first row are relative to the equilibrium distance. The identifiers are defined in Tab. ST10.

| System | 0.900 | 0.950 | 1.000 | 1.050 | 1.100 | 1.250 | 1.500 | 2.000 |
|---|---|---|---|---|---|---|---|---|
| 1 | −0.636 | −0.679 | −0.686 | −0.669 | −0.638 | −0.513 | −0.327 | −0.121 |
| 2 | −0.748 | −0.797 | −0.807 | −0.792 | −0.762 | −0.629 | −0.419 | −0.189 |
| 3 | −0.829 | −0.880 | −0.884 | −0.857 | −0.813 | −0.643 | −0.395 | −0.149 |
| 4 | −0.799 | −0.850 | −0.856 | −0.835 | −0.796 | −0.643 | −0.410 | −0.169 |
| 5 | −0.107 | −0.130 | −0.137 | −0.135 | −0.128 | −0.096 | −0.052 | −0.014 |
| 6 | −0.021 | −0.065 | −0.082 | −0.084 | −0.079 | −0.054 | −0.023 | −0.006 |
| 7 | −0.128 | −0.152 | −0.158 | −0.152 | −0.142 | −0.102 | −0.053 | −0.017 |
| 8 | 0.029 | −0.021 | −0.043 | −0.051 | −0.051 | −0.036 | −0.015 | −0.004 |
| 9 | 0.137 | 0.043 | −0.001 | −0.019 | −0.023 | −0.013 | 0.001 | 0.002 |
| 10 | 0.051 | −0.011 | −0.040 | −0.051 | −0.051 | −0.034 | −0.012 | −0.001 |
| 11 | 0.054 | 0.012 | −0.006 | −0.012 | −0.013 | −0.004 | 0.004 | 0.003 |
| 12 | −0.037 | −0.071 | −0.083 | −0.084 | −0.078 | −0.054 | −0.027 | −0.008 |
| 13 | −0.035 | −0.065 | −0.077 | −0.079 | −0.074 | −0.051 | −0.024 | −0.007 |
| 14 | −0.100 | −0.125 | −0.132 | −0.129 | −0.120 | −0.088 | −0.047 | −0.016 |
| 15 | 0.031 | −0.017 | −0.038 | −0.044 | −0.044 | −0.030 | −0.011 | −0.002 |
| 16 | −0.046 | −0.107 | −0.131 | −0.135 | −0.129 | −0.095 | −0.050 | −0.018 |
| 17 | 0.008 | −0.042 | −0.064 | −0.070 | −0.069 | −0.050 | −0.025 | −0.008 |
| 18 | 0.116 | 0.018 | −0.026 | −0.042 | −0.044 | −0.029 | −0.008 | −0.001 |
| 19 | 0.035 | −0.052 | −0.090 | −0.100 | −0.096 | −0.062 | −0.021 | −0.001 |
| 20 | −0.108 | −0.122 | −0.123 | −0.116 | −0.106 | −0.075 | −0.040 | −0.014 |
| 21 | 0.041 | −0.001 | −0.024 | −0.033 | −0.035 | −0.025 | −0.009 | −0.001 |
| 22 | 0.049 | 0.004 | −0.016 | −0.025 | −0.028 | −0.021 | −0.008 | −0.001 |
| 23 | 0.005 | −0.018 | −0.027 | −0.030 | −0.029 | −0.019 | −0.006 | −0.001 |
| 24 | −0.206 | −0.220 | −0.217 | −0.205 | −0.189 | −0.136 | −0.071 | −0.021 |
| 25 | −0.050 | −0.060 | −0.061 | −0.058 | −0.053 | −0.036 | −0.017 | −0.005 |
| 26 | 0.013 | −0.017 | −0.029 | −0.032 | −0.031 | −0.020 | −0.007 | −0.001 |
| 27 | −0.116 | −0.124 | −0.124 | −0.119 | −0.111 | −0.084 | −0.049 | −0.019 |
| 28 | −0.117 | −0.136 | −0.141 | −0.138 | −0.130 | −0.097 | −0.045 | −0.013 |
| 29 | −0.093 | −0.105 | −0.106 | −0.102 | −0.095 | −0.070 | −0.039 | −0.013 |
| 30 | −0.153 | −0.173 | −0.178 | −0.174 | −0.165 | −0.107 | −0.046 | −0.015 |
| 31 | −0.076 | −0.099 | −0.107 | −0.107 | −0.103 | −0.078 | −0.043 | −0.014 |
| 32 | −0.304 | −0.320 | −0.318 | −0.305 | −0.286 | −0.219 | −0.129 | −0.047 |
| 33 | −0.298 | −0.317 | −0.318 | −0.307 | −0.290 | −0.225 | −0.134 | −0.050 |
| 34 | −0.232 | −0.245 | −0.244 | −0.234 | −0.219 | −0.168 | −0.100 | −0.039 |
| 35 | −0.332 | −0.349 | −0.348 | −0.336 | −0.318 | −0.251 | −0.144 | −0.042 |
| 36 | −0.283 | −0.303 | −0.305 | −0.296 | −0.280 | −0.218 | −0.132 | −0.051 |
| 37 | −0.219 | −0.228 | −0.226 | −0.215 | −0.201 | −0.154 | −0.092 | −0.037 |
| 38 | 0.017 | −0.005 | −0.016 | −0.020 | −0.021 | −0.015 | −0.005 | −0.000 |
| 39 | 0.040 | −0.004 | −0.023 | −0.030 | −0.031 | −0.022 | −0.008 | −0.001 |
| 40 | −0.024 | −0.050 | −0.061 | −0.063 | −0.060 | −0.042 | −0.018 | −0.003 |
| 41 | −0.016 | −0.034 | −0.042 | −0.044 | −0.043 | −0.031 | −0.011 | −0.001 |
| 42 | 0.048 | −0.006 | −0.032 | −0.042 | −0.044 | −0.032 | −0.012 | −0.001 |
| 43 | −0.048 | −0.068 | −0.075 | −0.075 | −0.071 | −0.051 | −0.023 | −0.004 |
| 44 | −0.238 | −0.264 | −0.272 | −0.268 | −0.257 | −0.208 | −0.132 | −0.055 |
| 45 | −0.200 | −0.220 | −0.225 | −0.220 | −0.210 | −0.169 | −0.108 | −0.048 |
| 46 | −0.013 | −0.046 | −0.062 | −0.066 | −0.065 | −0.047 | −0.018 | −0.003 |
| 47 | −0.283 | −0.307 | −0.314 | −0.308 | −0.296 | −0.244 | −0.162 | −0.066 |
| 48 | −0.188 | −0.203 | −0.205 | −0.200 | −0.190 | −0.152 | −0.098 | −0.046 |
| 49 | 0.027 | −0.009 | −0.024 | −0.029 | −0.028 | −0.016 | −0.002 | 0.001 |
| 50 | −0.142 | −0.156 | −0.159 | −0.154 | −0.145 | −0.111 | −0.064 | −0.023 |
| 51 | −0.050 | −0.099 | −0.121 | −0.118 | −0.106 | −0.067 | −0.029 | −0.006 |
| 52 | −0.008 | −0.051 | −0.070 | −0.075 | −0.074 | −0.055 | −0.028 | −0.009 |
| 53 | 0.091 | −0.001 | −0.043 | −0.059 | −0.060 | −0.042 | −0.016 | −0.004 |
| 54 | 0.025 | −0.094 | −0.139 | −0.148 | −0.140 | −0.094 | −0.044 | −0.015 |
| 55 | 0.042 | −0.017 | −0.043 | −0.051 | −0.051 | −0.034 | −0.012 | −0.001 |
| 56 | −0.024 | −0.059 | −0.074 | −0.076 | −0.072 | −0.050 | −0.023 | −0.006 |
| 57 | −0.053 | −0.091 | −0.104 | −0.103 | −0.097 | −0.066 | −0.030 | −0.008 |
| 58 | 0.010 | −0.035 | −0.054 | −0.058 | −0.055 | −0.036 | −0.014 | −0.002 |
| 59 | 0.023 | −0.033 | −0.058 | −0.066 | −0.063 | −0.037 | −0.011 | −0.001 |
| 60 | −0.653 | −0.702 | −0.712 | −0.696 | −0.665 | −0.534 | −0.335 | −0.133 |
| 61 | −0.118 | −0.205 | −0.237 | −0.239 | −0.226 | −0.162 | −0.084 | −0.029 |
| 62 | −0.302 | −0.313 | −0.309 | −0.295 | −0.277 | −0.211 | −0.125 | −0.046 |
| 63 | −0.239 | −0.249 | −0.245 | −0.234 | −0.218 | −0.165 | −0.097 | −0.037 |
| 64 | −0.346 | −0.358 | −0.354 | −0.339 | −0.319 | −0.251 | −0.156 | −0.057 |
| 65 | −0.287 | −0.300 | −0.297 | −0.285 | −0.267 | −0.205 | −0.123 | −0.047 |
| 66 | −0.226 | −0.232 | −0.227 | −0.216 | −0.200 | −0.152 | −0.090 | −0.036 |

Table ST14: Interaction energies for the S66x8 data set using SCAN. The units are eV. Distances in the first row are relative to the equilibrium distance. The identifiers are defined in Tab. ST10.

| System | 0.900 | 0.950 | 1.000 | 1.050 | 1.100 | 1.250 | 1.500 | 2.000 |
|---|---|---|---|---|---|---|---|---|
| 1 | −0.731 | −0.758 | −0.751 | −0.725 | −0.685 | −0.544 | −0.342 | −0.125 |
| 2 | −0.858 | −0.888 | −0.884 | −0.857 | −0.817 | −0.666 | −0.438 | −0.195 |
| 3 | −0.953 | −0.979 | −0.965 | −0.925 | −0.872 | −0.683 | −0.417 | −0.155 |
| 4 | −0.913 | −0.941 | −0.932 | −0.899 | −0.852 | −0.680 | −0.429 | −0.174 |
| 5 | −0.144 | −0.162 | −0.165 | −0.159 | −0.148 | −0.107 | −0.056 | −0.015 |
| 6 | −0.070 | −0.110 | −0.121 | −0.117 | −0.106 | −0.066 | −0.026 | −0.006 |
| 7 | −0.167 | −0.189 | −0.191 | −0.182 | −0.167 | −0.117 | −0.058 | −0.017 |
| 8 | −0.002 | −0.050 | −0.068 | −0.071 | −0.066 | −0.042 | −0.016 | −0.003 |
| 9 | 0.081 | −0.009 | −0.047 | −0.057 | −0.054 | −0.026 | −0.001 | 0.002 |
| 10 | −0.007 | −0.061 | −0.083 | −0.085 | −0.077 | −0.045 | −0.014 | −0.001 |
| 11 | 0.023 | −0.017 | −0.031 | −0.033 | −0.029 | −0.010 | 0.004 | 0.003 |
| 12 | −0.056 | −0.089 | −0.099 | −0.097 | −0.088 | −0.058 | −0.027 | −0.009 |
| 13 | −0.076 | −0.102 | −0.109 | −0.106 | −0.096 | −0.061 | −0.026 | −0.007 |
| 14 | −0.141 | −0.163 | −0.166 | −0.158 | −0.146 | −0.101 | −0.051 | −0.016 |
| 15 | −0.009 | −0.051 | −0.066 | −0.068 | −0.062 | −0.037 | −0.012 | −0.002 |
| 16 | −0.101 | −0.157 | −0.175 | −0.173 | −0.160 | −0.111 | −0.055 | −0.019 |
| 17 | −0.024 | −0.072 | −0.089 | −0.091 | −0.085 | −0.056 | −0.025 | −0.008 |
| 18 | 0.058 | −0.037 | −0.075 | −0.083 | −0.078 | −0.044 | −0.010 | −0.001 |
| 19 | −0.054 | −0.135 | −0.164 | −0.163 | −0.149 | −0.087 | −0.026 | −0.001 |
| 20 | −0.137 | −0.149 | −0.146 | −0.137 | −0.124 | −0.085 | −0.043 | −0.015 |
| 21 | −0.008 | −0.040 | −0.053 | −0.053 | −0.048 | −0.027 | −0.008 | −0.001 |
| 22 | 0.004 | −0.029 | −0.041 | −0.043 | −0.039 | −0.024 | −0.007 | −0.000 |
| 23 | −0.028 | −0.043 | −0.046 | −0.043 | −0.038 | −0.021 | −0.006 | −0.000 |
| 24 | −0.228 | −0.239 | −0.234 | −0.221 | −0.202 | −0.144 | −0.074 | −0.022 |
| 25 | −0.051 | −0.059 | −0.060 | −0.057 | −0.052 | −0.034 | −0.016 | −0.005 |
| 26 | −0.016 | −0.040 | −0.047 | −0.046 | −0.041 | −0.024 | −0.007 | −0.001 |
| 27 | −0.119 | −0.126 | −0.125 | −0.119 | −0.111 | −0.083 | −0.048 | −0.019 |
| 28 | −0.157 | −0.170 | −0.169 | −0.161 | −0.148 | −0.105 | −0.046 | −0.013 |
| 29 | −0.117 | −0.124 | −0.122 | −0.114 | −0.104 | −0.074 | −0.039 | −0.014 |
| 30 | −0.204 | −0.217 | −0.216 | −0.207 | −0.193 | −0.118 | −0.047 | −0.015 |
| 31 | −0.125 | −0.140 | −0.143 | −0.138 | −0.128 | −0.091 | −0.046 | −0.014 |
| 32 | −0.356 | −0.363 | −0.354 | −0.335 | −0.312 | −0.235 | −0.135 | −0.048 |
| 33 | −0.351 | −0.361 | −0.354 | −0.337 | −0.315 | −0.239 | −0.139 | −0.051 |
| 34 | −0.269 | −0.276 | −0.270 | −0.256 | −0.238 | −0.179 | −0.104 | −0.040 |
| 35 | −0.384 | −0.393 | −0.387 | −0.370 | −0.347 | −0.270 | −0.152 | −0.043 |
| 36 | −0.335 | −0.345 | −0.340 | −0.324 | −0.303 | −0.232 | −0.136 | −0.052 |
| 37 | −0.242 | −0.248 | −0.242 | −0.229 | −0.212 | −0.160 | −0.094 | −0.038 |
| 38 | −0.003 | −0.020 | −0.025 | −0.026 | −0.024 | −0.014 | −0.004 | −0.001 |
| 39 | −0.006 | −0.039 | −0.049 | −0.049 | −0.044 | −0.024 | −0.007 | −0.000 |
| 40 | −0.081 | −0.097 | −0.099 | −0.093 | −0.084 | −0.052 | −0.019 | −0.003 |
| 41 | −0.066 | −0.076 | −0.076 | −0.072 | −0.065 | −0.041 | −0.012 | −0.001 |
| 42 | −0.028 | −0.067 | −0.079 | −0.078 | −0.070 | −0.040 | −0.012 | −0.000 |
| 43 | −0.082 | −0.097 | −0.099 | −0.094 | −0.086 | −0.057 | −0.023 | −0.005 |
| 44 | −0.299 | −0.315 | −0.315 | −0.304 | −0.287 | −0.226 | −0.138 | −0.057 |
| 45 | −0.244 | −0.258 | −0.257 | −0.248 | −0.234 | −0.183 | −0.114 | −0.050 |
| 46 | −0.087 | −0.110 | −0.115 | −0.109 | −0.099 | −0.062 | −0.020 | −0.003 |
| 47 | −0.343 | −0.359 | −0.358 | −0.348 | −0.331 | −0.267 | −0.172 | −0.068 |
| 48 | −0.212 | −0.223 | −0.222 | −0.214 | −0.202 | −0.159 | −0.101 | −0.047 |
| 49 | −0.007 | −0.040 | −0.052 | −0.052 | −0.047 | −0.024 | −0.004 | 0.002 |
| 50 | −0.156 | −0.165 | −0.164 | −0.157 | −0.146 | −0.109 | −0.062 | −0.023 |
| 51 | −0.072 | −0.115 | −0.131 | −0.124 | −0.108 | −0.065 | −0.028 | −0.006 |
| 52 | −0.045 | −0.084 | −0.097 | −0.098 | −0.092 | −0.063 | −0.029 | −0.009 |
| 53 | 0.029 | −0.059 | −0.095 | −0.102 | −0.097 | −0.059 | −0.018 | −0.004 |
| 54 | −0.067 | −0.181 | −0.215 | −0.211 | −0.191 | −0.117 | −0.049 | −0.016 |
| 55 | −0.036 | −0.084 | −0.098 | −0.095 | −0.084 | −0.047 | −0.013 | −0.001 |
| 56 | −0.072 | −0.103 | −0.112 | −0.107 | −0.098 | −0.061 | −0.025 | −0.007 |
| 57 | −0.094 | −0.129 | −0.138 | −0.133 | −0.120 | −0.078 | −0.033 | −0.008 |
| 58 | −0.051 | −0.089 | −0.099 | −0.094 | −0.084 | −0.048 | −0.016 | −0.003 |
| 59 | −0.067 | −0.111 | −0.123 | −0.118 | −0.103 | −0.051 | −0.012 | −0.000 |
| 60 | −0.764 | −0.793 | −0.788 | −0.760 | −0.720 | −0.570 | −0.352 | −0.138 |
| 61 | −0.256 | −0.332 | −0.349 | −0.335 | −0.305 | −0.204 | −0.096 | −0.032 |
| 62 | −0.342 | −0.345 | −0.335 | −0.317 | −0.294 | −0.222 | −0.128 | −0.047 |
| 63 | −0.274 | −0.278 | −0.270 | −0.255 | −0.235 | −0.175 | −0.101 | −0.039 |
| 64 | −0.394 | −0.400 | −0.390 | −0.372 | −0.348 | −0.270 | −0.166 | −0.059 |
| 65 | −0.327 | −0.333 | −0.324 | −0.307 | −0.285 | −0.215 | −0.126 | −0.048 |
| 66 | −0.246 | −0.250 | −0.242 | −0.228 | −0.211 | −0.157 | −0.092 | −0.037 |

Table ST15: Interaction energies for the S66x8 data set using $r^2$SCAN. The units are eV. Distances in the first row are relative to the equilibrium distance. The identifiers are defined in Tab. ST10.

| System | 0.900 | 0.950 | 1.000 | 1.050 | 1.100 | 1.250 | 1.500 | 2.000 |
|---|---|---|---|---|---|---|---|---|
| 1 | −0.683 | −0.715 | −0.714 | −0.692 | −0.657 | −0.526 | −0.333 | −0.123 |
| 2 | −0.807 | −0.843 | −0.844 | −0.822 | −0.786 | −0.645 | −0.426 | −0.191 |
| 3 | −0.894 | −0.927 | −0.919 | −0.885 | −0.836 | −0.659 | −0.405 | −0.152 |
| 4 | −0.858 | −0.893 | −0.890 | −0.862 | −0.819 | −0.658 | −0.418 | −0.171 |
| 5 | −0.125 | −0.147 | −0.153 | −0.149 | −0.140 | −0.104 | −0.055 | −0.015 |
| 6 | −0.043 | −0.090 | −0.106 | −0.106 | −0.098 | −0.063 | −0.025 | −0.006 |
| 7 | −0.145 | −0.172 | −0.177 | −0.171 | −0.159 | −0.113 | −0.058 | −0.018 |
| 8 | 0.018 | −0.035 | −0.057 | −0.063 | −0.061 | −0.040 | −0.016 | −0.004 |
| 9 | 0.118 | 0.018 | −0.028 | −0.044 | −0.045 | −0.023 | −0.000 | 0.002 |
| 10 | 0.021 | −0.040 | −0.067 | −0.074 | −0.070 | −0.043 | −0.013 | −0.001 |
| 11 | 0.047 | 0.001 | −0.019 | −0.024 | −0.023 | −0.008 | 0.004 | 0.003 |
| 12 | −0.040 | −0.077 | −0.090 | −0.090 | −0.084 | −0.057 | −0.027 | −0.009 |
| 13 | −0.057 | −0.087 | −0.098 | −0.097 | −0.090 | −0.059 | −0.026 | −0.007 |
| 14 | −0.120 | −0.146 | −0.153 | −0.149 | −0.138 | −0.099 | −0.050 | −0.017 |
| 15 | 0.013 | −0.035 | −0.055 | −0.059 | −0.056 | −0.035 | −0.012 | −0.002 |
| 16 | −0.074 | −0.137 | −0.160 | −0.162 | −0.152 | −0.107 | −0.054 | −0.019 |
| 17 | −0.003 | −0.056 | −0.077 | −0.082 | −0.079 | −0.054 | −0.025 | −0.008 |
| 18 | 0.097 | −0.009 | −0.055 | −0.069 | −0.068 | −0.041 | −0.009 | −0.001 |
| 19 | −0.008 | −0.101 | −0.138 | −0.145 | −0.136 | −0.083 | −0.025 | −0.001 |
| 20 | −0.120 | −0.136 | −0.137 | −0.129 | −0.118 | −0.082 | −0.043 | −0.015 |
| 21 | 0.013 | −0.024 | −0.041 | −0.044 | −0.042 | −0.024 | −0.007 | −0.000 |
| 22 | 0.023 | −0.015 | −0.030 | −0.035 | −0.034 | −0.021 | −0.007 | −0.000 |
| 23 | −0.013 | −0.033 | −0.038 | −0.037 | −0.034 | −0.019 | −0.006 | −0.000 |
| 24 | −0.205 | −0.220 | −0.219 | −0.208 | −0.192 | −0.139 | −0.073 | −0.022 |
| 25 | −0.042 | −0.053 | −0.056 | −0.053 | −0.049 | −0.033 | −0.016 | −0.005 |
| 26 | 0.000 | −0.028 | −0.038 | −0.040 | −0.037 | −0.022 | −0.007 | −0.001 |
| 27 | −0.109 | −0.118 | −0.118 | −0.114 | −0.106 | −0.081 | −0.048 | −0.019 |
| 28 | −0.141 | −0.156 | −0.158 | −0.152 | −0.141 | −0.102 | −0.045 | −0.013 |
| 29 | −0.105 | −0.114 | −0.113 | −0.107 | −0.099 | −0.071 | −0.038 | −0.014 |
| 30 | −0.181 | −0.199 | −0.201 | −0.194 | −0.183 | −0.114 | −0.046 | −0.015 |
| 31 | −0.105 | −0.124 | −0.130 | −0.127 | −0.119 | −0.087 | −0.045 | −0.014 |
| 32 | −0.334 | −0.344 | −0.337 | −0.321 | −0.300 | −0.227 | −0.132 | −0.048 |
| 33 | −0.331 | −0.343 | −0.339 | −0.325 | −0.304 | −0.233 | −0.137 | −0.050 |
| 34 | −0.248 | −0.258 | −0.255 | −0.243 | −0.227 | −0.172 | −0.101 | −0.039 |
| 35 | −0.356 | −0.369 | −0.366 | −0.352 | −0.332 | −0.261 | −0.148 | −0.043 |
| 36 | −0.314 | −0.327 | −0.324 | −0.311 | −0.292 | −0.225 | −0.134 | −0.051 |
| 37 | −0.226 | −0.234 | −0.230 | −0.219 | −0.204 | −0.155 | −0.093 | −0.038 |
| 38 | 0.009 | −0.010 | −0.018 | −0.021 | −0.020 | −0.012 | −0.004 | −0.000 |
| 39 | 0.013 | −0.024 | −0.038 | −0.041 | −0.038 | −0.022 | −0.006 | −0.000 |
| 40 | −0.059 | −0.080 | −0.086 | −0.083 | −0.076 | −0.049 | −0.019 | −0.003 |
| 41 | −0.049 | −0.062 | −0.066 | −0.064 | −0.058 | −0.038 | −0.011 | −0.001 |
| 42 | −0.001 | −0.046 | −0.064 | −0.066 | −0.061 | −0.037 | −0.011 | −0.001 |
| 43 | −0.065 | −0.084 | −0.089 | −0.086 | −0.080 | −0.054 | −0.023 | −0.004 |
| 44 | −0.280 | −0.299 | −0.301 | −0.292 | −0.277 | −0.219 | −0.136 | −0.056 |
| 45 | −0.223 | −0.240 | −0.242 | −0.235 | −0.223 | −0.177 | −0.111 | −0.049 |
| 46 | −0.061 | −0.089 | −0.099 | −0.097 | −0.090 | −0.059 | −0.019 | −0.003 |
| 47 | −0.317 | −0.336 | −0.339 | −0.331 | −0.316 | −0.258 | −0.168 | −0.067 |
| 48 | −0.197 | −0.210 | −0.211 | −0.205 | −0.194 | −0.154 | −0.100 | −0.047 |
| 49 | 0.017 | −0.022 | −0.038 | −0.042 | −0.040 | −0.022 | −0.003 | 0.002 |
| 50 | −0.144 | −0.156 | −0.156 | −0.150 | −0.141 | −0.106 | −0.061 | −0.023 |
| 51 | −0.052 | −0.099 | −0.120 | −0.115 | −0.102 | −0.062 | −0.027 | −0.006 |
| 52 | −0.024 | −0.067 | −0.085 | −0.089 | −0.085 | −0.060 | −0.028 | −0.009 |
| 53 | 0.069 | −0.030 | −0.074 | −0.088 | −0.086 | −0.055 | −0.018 | −0.004 |
| 54 | −0.017 | −0.144 | −0.189 | −0.193 | −0.178 | −0.112 | −0.047 | −0.015 |
| 55 | −0.007 | −0.062 | −0.082 | −0.083 | −0.076 | −0.044 | −0.013 | −0.001 |
| 56 | −0.046 | −0.084 | −0.097 | −0.096 | −0.089 | −0.058 | −0.024 | −0.006 |
| 57 | −0.067 | −0.108 | −0.122 | −0.121 | −0.112 | −0.074 | −0.032 | −0.008 |
| 58 | −0.027 | −0.071 | −0.086 | −0.085 | −0.077 | −0.046 | −0.016 | −0.003 |
| 59 | −0.034 | −0.086 | −0.105 | −0.105 | −0.094 | −0.048 | −0.012 | −0.001 |
| 60 | −0.715 | −0.750 | −0.750 | −0.727 | −0.691 | −0.551 | −0.344 | −0.136 |
| 61 | −0.206 | −0.293 | −0.319 | −0.313 | −0.289 | −0.197 | −0.094 | −0.030 |
| 62 | −0.322 | −0.328 | −0.320 | −0.304 | −0.283 | −0.215 | −0.125 | −0.046 |
| 63 | −0.252 | −0.259 | −0.254 | −0.241 | −0.224 | −0.169 | −0.098 | −0.038 |
| 64 | −0.365 | −0.375 | −0.369 | −0.353 | −0.332 | −0.260 | −0.161 | −0.058 |
| 65 | −0.306 | −0.314 | −0.308 | −0.293 | −0.274 | −0.208 | −0.123 | −0.047 |
| 66 | −0.229 | −0.235 | −0.230 | −0.217 | −0.202 | −0.153 | −0.091 | −0.037 |

Table ST16: Interaction energies for the S66x8 data set using SCAN-v. The units are eV. Distances in the first row are relative to the equilibrium distance. The identifiers are defined in Tab. ST10.

| System | 0.900 | 0.950 | 1.000 | 1.050 | 1.100 | 1.250 | 1.500 | 2.000 |
|---|---|---|---|---|---|---|---|---|
| 1 | −0.761 | −0.786 | −0.778 | −0.750 | −0.709 | −0.563 | −0.355 | −0.130 |
| 2 | −0.894 | −0.922 | −0.916 | −0.888 | −0.846 | −0.690 | −0.455 | −0.204 |
| 3 | −0.983 | −1.008 | −0.992 | −0.952 | −0.896 | −0.704 | −0.431 | −0.163 |
| 4 | −0.948 | −0.974 | −0.964 | −0.929 | −0.880 | −0.704 | −0.446 | −0.183 |
| 5 | −0.177 | −0.193 | −0.193 | −0.185 | −0.172 | −0.125 | −0.067 | −0.019 |
| 6 | −0.120 | −0.155 | −0.162 | −0.154 | −0.139 | −0.089 | −0.039 | −0.010 |
| 7 | −0.205 | −0.224 | −0.223 | −0.211 | −0.194 | −0.137 | −0.070 | −0.022 |
| 8 | −0.047 | −0.091 | −0.105 | −0.104 | −0.096 | −0.063 | −0.028 | −0.007 |
| 9 | 0.009 | −0.074 | −0.105 | −0.108 | −0.100 | −0.057 | −0.015 | −0.002 |
| 10 | −0.072 | −0.120 | −0.136 | −0.132 | −0.120 | −0.075 | −0.030 | −0.006 |
| 11 | −0.015 | −0.051 | −0.062 | −0.060 | −0.053 | −0.027 | −0.005 | 0.001 |
| 12 | −0.081 | −0.112 | −0.119 | −0.115 | −0.105 | −0.070 | −0.034 | −0.011 |
| 13 | −0.113 | −0.136 | −0.140 | −0.133 | −0.121 | −0.079 | −0.036 | −0.010 |
| 14 | −0.177 | −0.195 | −0.196 | −0.185 | −0.170 | −0.120 | −0.062 | −0.020 |
| 15 | −0.064 | −0.100 | −0.111 | −0.108 | −0.098 | −0.062 | −0.026 | −0.006 |
| 16 | −0.158 | −0.209 | −0.222 | −0.215 | −0.198 | −0.138 | −0.070 | −0.024 |
| 17 | −0.069 | −0.112 | −0.126 | −0.123 | −0.114 | −0.077 | −0.037 | −0.012 |
| 18 | −0.015 | −0.103 | −0.133 | −0.135 | −0.124 | −0.075 | −0.025 | −0.005 |
| 19 | −0.144 | −0.218 | −0.238 | −0.231 | −0.209 | −0.130 | −0.049 | −0.009 |
| 20 | −0.157 | −0.167 | −0.163 | −0.152 | −0.138 | −0.095 | −0.049 | −0.017 |
| 21 | −0.065 | −0.092 | −0.100 | −0.095 | −0.086 | −0.054 | −0.024 | −0.007 |
| 22 | −0.049 | −0.076 | −0.083 | −0.080 | −0.073 | −0.048 | −0.021 | −0.006 |
| 23 | −0.060 | −0.072 | −0.072 | −0.067 | −0.059 | −0.036 | −0.015 | −0.004 |
| 24 | −0.247 | −0.256 | −0.250 | −0.235 | −0.216 | −0.154 | −0.081 | −0.024 |
| 25 | −0.059 | −0.067 | −0.068 | −0.063 | −0.057 | −0.038 | −0.019 | −0.005 |
| 26 | −0.046 | −0.067 | −0.071 | −0.067 | −0.060 | −0.037 | −0.015 | −0.003 |
| 27 | −0.126 | −0.132 | −0.131 | −0.124 | −0.115 | −0.086 | −0.050 | −0.020 |
| 28 | −0.177 | −0.188 | −0.186 | −0.176 | −0.163 | −0.117 | −0.052 | −0.015 |
| 29 | −0.134 | −0.139 | −0.136 | −0.127 | −0.116 | −0.083 | −0.045 | −0.016 |
| 30 | −0.235 | −0.247 | −0.244 | −0.233 | −0.216 | −0.134 | −0.056 | −0.018 |
| 31 | −0.159 | −0.172 | −0.172 | −0.164 | −0.152 | −0.110 | −0.058 | −0.019 |
| 32 | −0.369 | −0.375 | −0.365 | −0.346 | −0.322 | −0.242 | −0.140 | −0.051 |
| 33 | −0.370 | −0.378 | −0.370 | −0.352 | −0.329 | −0.251 | −0.147 | −0.054 |
| 34 | −0.284 | −0.291 | −0.283 | −0.269 | −0.250 | −0.188 | −0.110 | −0.043 |
| 35 | −0.407 | −0.416 | −0.408 | −0.390 | −0.366 | −0.286 | −0.162 | −0.047 |
| 36 | −0.356 | −0.365 | −0.358 | −0.342 | −0.319 | −0.245 | −0.145 | −0.056 |
| 37 | −0.252 | −0.257 | −0.250 | −0.237 | −0.220 | −0.166 | −0.098 | −0.039 |
| 38 | −0.044 | −0.057 | −0.059 | −0.056 | −0.051 | −0.033 | −0.015 | −0.005 |
| 39 | −0.060 | −0.087 | −0.092 | −0.087 | −0.079 | −0.049 | −0.022 | −0.006 |
| 40 | −0.132 | −0.144 | −0.142 | −0.132 | −0.119 | −0.079 | −0.036 | −0.009 |
| 41 | −0.112 | −0.118 | −0.116 | −0.108 | −0.098 | −0.066 | −0.026 | −0.005 |
| 42 | −0.098 | −0.130 | −0.137 | −0.130 | −0.117 | −0.075 | −0.033 | −0.008 |
| 43 | −0.112 | −0.125 | −0.125 | −0.118 | −0.107 | −0.073 | −0.033 | −0.007 |
| 44 | −0.328 | −0.342 | −0.340 | −0.327 | −0.309 | −0.243 | −0.150 | −0.062 |
| 45 | −0.270 | −0.282 | −0.280 | −0.269 | −0.253 | −0.198 | −0.124 | −0.055 |
| 46 | −0.151 | −0.169 | −0.169 | −0.159 | −0.145 | −0.097 | −0.040 | −0.010 |
| 47 | −0.381 | −0.395 | −0.392 | −0.379 | −0.360 | −0.291 | −0.189 | −0.075 |
| 48 | −0.227 | −0.237 | −0.234 | −0.225 | −0.212 | −0.167 | −0.107 | −0.050 |
| 49 | −0.045 | −0.074 | −0.082 | −0.079 | −0.071 | −0.041 | −0.013 | −0.001 |
| 50 | −0.169 | −0.178 | −0.176 | −0.168 | −0.156 | −0.117 | −0.067 | −0.025 |
| 51 | −0.100 | −0.141 | −0.154 | −0.144 | −0.126 | −0.077 | −0.035 | −0.009 |
| 52 | −0.088 | −0.123 | −0.133 | −0.131 | −0.121 | −0.084 | −0.042 | −0.014 |
| 53 | −0.044 | −0.125 | −0.153 | −0.155 | −0.143 | −0.091 | −0.035 | −0.009 |
| 54 | −0.159 | −0.264 | −0.289 | −0.277 | −0.249 | −0.157 | −0.070 | −0.022 |
| 55 | −0.112 | −0.152 | −0.159 | −0.150 | −0.134 | −0.083 | −0.034 | −0.008 |
| 56 | −0.116 | −0.143 | −0.147 | −0.140 | −0.126 | −0.082 | −0.037 | −0.011 |
| 57 | −0.133 | −0.164 | −0.170 | −0.161 | −0.146 | −0.096 | −0.043 | −0.011 |
| 58 | −0.115 | −0.146 | −0.150 | −0.141 | −0.125 | −0.078 | −0.033 | −0.009 |
| 59 | −0.149 | −0.186 | −0.192 | −0.180 | −0.157 | −0.088 | −0.032 | −0.007 |
| 60 | −0.806 | −0.833 | −0.825 | −0.796 | −0.753 | −0.597 | −0.372 | −0.148 |
| 61 | −0.364 | −0.430 | −0.439 | −0.416 | −0.380 | −0.258 | −0.128 | −0.043 |
| 62 | −0.352 | −0.355 | −0.344 | −0.326 | −0.302 | −0.228 | −0.132 | −0.049 |
| 63 | −0.285 | −0.288 | −0.280 | −0.263 | −0.244 | −0.182 | −0.105 | −0.041 |
| 64 | −0.411 | −0.415 | −0.405 | −0.386 | −0.361 | −0.281 | −0.173 | −0.062 |
| 65 | −0.341 | −0.345 | −0.336 | −0.318 | −0.295 | −0.223 | −0.131 | −0.050 |
| 66 | −0.253 | −0.256 | −0.248 | −0.233 | −0.216 | −0.161 | −0.095 | −0.038 |

Table ST17: Interaction energies for the S66x8 data set using MCML. The units are eV. Distances in the first row are relative to the equilibrium distance. The identifiers are defined in Tab. ST10.

| System | 0.900 | 0.950 | 1.000 | 1.050 | 1.100 | 1.250 | 1.500 | 2.000 |
|---|---|---|---|---|---|---|---|---|
| 1 | −0.606 | −0.661 | −0.676 | −0.665 | −0.638 | −0.524 | −0.341 | −0.122 |
| 2 | −0.724 | −0.781 | −0.799 | −0.790 | −0.764 | −0.640 | −0.434 | −0.192 |
| 3 | −0.818 | −0.863 | −0.869 | −0.854 | −0.821 | −0.664 | −0.418 | −0.158 |
| 4 | −0.782 | −0.834 | −0.847 | −0.835 | −0.804 | −0.660 | −0.430 | −0.175 |
| 5 | −0.142 | −0.166 | −0.173 | −0.171 | −0.162 | −0.122 | −0.063 | −0.015 |
| 6 | −0.101 | −0.143 | −0.154 | −0.150 | −0.137 | −0.086 | −0.030 | −0.005 |
| 7 | −0.203 | −0.224 | −0.224 | −0.213 | −0.196 | −0.139 | −0.068 | −0.017 |
| 8 | −0.016 | −0.067 | −0.087 | −0.091 | −0.085 | −0.055 | −0.019 | −0.003 |
| 9 | 0.011 | −0.076 | −0.110 | −0.116 | −0.108 | −0.060 | −0.008 | 0.002 |
| 10 | −0.010 | −0.074 | −0.101 | −0.107 | −0.101 | −0.064 | −0.019 | −0.001 |
| 11 | −0.027 | −0.066 | −0.079 | −0.077 | −0.069 | −0.035 | −0.003 | 0.003 |
| 12 | −0.065 | −0.101 | −0.112 | −0.110 | −0.101 | −0.066 | −0.028 | −0.008 |
| 13 | −0.096 | −0.125 | −0.134 | −0.131 | −0.120 | −0.079 | −0.031 | −0.006 |
| 14 | −0.169 | −0.191 | −0.194 | −0.186 | −0.173 | −0.122 | −0.059 | −0.016 |
| 15 | −0.021 | −0.069 | −0.087 | −0.089 | −0.083 | −0.052 | −0.016 | −0.002 |
| 16 | −0.115 | −0.177 | −0.199 | −0.198 | −0.187 | −0.131 | −0.061 | −0.018 |
| 17 | −0.034 | −0.085 | −0.105 | −0.108 | −0.102 | −0.068 | −0.028 | −0.008 |
| 18 | −0.009 | −0.101 | −0.136 | −0.141 | −0.131 | −0.078 | −0.018 | −0.001 |
| 19 | −0.134 | −0.214 | −0.240 | −0.236 | −0.217 | −0.135 | −0.041 | −0.001 |
| 20 | −0.167 | −0.176 | −0.172 | −0.161 | −0.146 | −0.100 | −0.048 | −0.014 |
| 21 | 0.045 | −0.006 | −0.034 | −0.044 | −0.045 | −0.030 | −0.008 | 0.000 |
| 22 | 0.047 | −0.003 | −0.026 | −0.035 | −0.036 | −0.025 | −0.007 | 0.000 |
| 23 | −0.008 | −0.035 | −0.045 | −0.047 | −0.044 | −0.027 | −0.008 | −0.000 |
| 24 | −0.225 | −0.243 | −0.243 | −0.232 | −0.216 | −0.158 | −0.083 | −0.022 |
| 25 | −0.052 | −0.063 | −0.065 | −0.062 | −0.056 | −0.036 | −0.016 | −0.004 |
| 26 | −0.030 | −0.059 | −0.069 | −0.069 | −0.062 | −0.037 | −0.010 | −0.001 |
| 27 | −0.103 | −0.116 | −0.119 | −0.117 | −0.110 | −0.084 | −0.047 | −0.018 |
| 28 | −0.112 | −0.137 | −0.146 | −0.145 | −0.139 | −0.106 | −0.047 | −0.012 |
| 29 | −0.108 | −0.120 | −0.123 | −0.119 | −0.111 | −0.082 | −0.042 | −0.013 |
| 30 | −0.177 | −0.200 | −0.207 | −0.204 | −0.195 | −0.126 | −0.048 | −0.014 |
| 31 | −0.114 | −0.138 | −0.147 | −0.146 | −0.140 | −0.106 | −0.053 | −0.014 |
| 32 | −0.287 | −0.310 | −0.314 | −0.306 | −0.290 | −0.226 | −0.134 | −0.047 |
| 33 | −0.274 | −0.301 | −0.309 | −0.303 | −0.290 | −0.229 | −0.138 | −0.049 |
| 34 | −0.242 | −0.261 | −0.262 | −0.253 | −0.238 | −0.185 | −0.110 | −0.039 |
| 35 | −0.341 | −0.363 | −0.367 | −0.358 | −0.341 | −0.273 | −0.157 | −0.042 |
| 36 | −0.258 | −0.285 | −0.294 | −0.290 | −0.278 | −0.221 | −0.136 | −0.050 |
| 37 | −0.225 | −0.239 | −0.239 | −0.230 | −0.216 | −0.167 | −0.099 | −0.037 |
| 38 | 0.020 | −0.005 | −0.017 | −0.021 | −0.021 | −0.014 | −0.004 | 0.000 |
| 39 | 0.033 | −0.017 | −0.038 | −0.045 | −0.044 | −0.028 | −0.008 | 0.000 |
| 40 | −0.075 | −0.102 | −0.111 | −0.110 | −0.102 | −0.068 | −0.025 | −0.003 |
| 41 | −0.069 | −0.086 | −0.091 | −0.090 | −0.084 | −0.057 | −0.016 | −0.000 |
| 42 | 0.027 | −0.036 | −0.065 | −0.075 | −0.074 | −0.050 | −0.015 | −0.000 |
| 43 | −0.082 | −0.103 | −0.110 | −0.107 | −0.099 | −0.068 | −0.026 | −0.004 |
| 44 | −0.233 | −0.264 | −0.275 | −0.273 | −0.264 | −0.217 | −0.138 | −0.055 |
| 45 | −0.221 | −0.243 | −0.249 | −0.246 | −0.236 | −0.192 | −0.120 | −0.049 |
| 46 | −0.070 | −0.107 | −0.122 | −0.124 | −0.118 | −0.082 | −0.026 | −0.002 |
| 47 | −0.307 | −0.334 | −0.342 | −0.337 | −0.326 | −0.271 | −0.179 | −0.067 |
| 48 | −0.199 | −0.216 | −0.220 | −0.215 | −0.206 | −0.166 | −0.105 | −0.046 |
| 49 | −0.053 | −0.086 | −0.097 | −0.095 | −0.086 | −0.051 | −0.012 | 0.002 |
| 50 | −0.102 | −0.123 | −0.132 | −0.132 | −0.127 | −0.101 | −0.059 | −0.022 |
| 51 | 0.000 | −0.063 | −0.101 | −0.106 | −0.099 | −0.063 | −0.026 | −0.006 |
| 52 | −0.042 | −0.088 | −0.107 | −0.111 | −0.106 | −0.075 | −0.032 | −0.008 |
| 53 | −0.036 | −0.123 | −0.156 | −0.161 | −0.150 | −0.094 | −0.027 | −0.004 |
| 54 | −0.140 | −0.253 | −0.286 | −0.280 | −0.255 | −0.157 | −0.057 | −0.015 |
| 55 | −0.045 | −0.104 | −0.125 | −0.125 | −0.115 | −0.070 | −0.019 | −0.001 |
| 56 | −0.109 | −0.142 | −0.151 | −0.146 | −0.134 | −0.087 | −0.033 | −0.006 |
| 57 | −0.144 | −0.179 | −0.186 | −0.178 | −0.163 | −0.106 | −0.041 | −0.008 |
| 58 | −0.068 | −0.113 | −0.127 | −0.124 | −0.113 | −0.069 | −0.021 | −0.002 |
| 59 | −0.073 | −0.130 | −0.151 | −0.151 | −0.137 | −0.075 | −0.017 | −0.001 |
| 60 | −0.637 | −0.695 | −0.712 | −0.701 | −0.673 | −0.551 | −0.352 | −0.136 |
| 61 | −0.320 | −0.399 | −0.419 | −0.406 | −0.374 | −0.253 | −0.110 | −0.029 |
| 62 | −0.275 | −0.294 | −0.296 | −0.287 | −0.272 | −0.212 | −0.127 | −0.045 |
| 63 | −0.248 | −0.263 | −0.262 | −0.252 | −0.236 | −0.181 | −0.106 | −0.037 |
| 64 | −0.361 | −0.379 | −0.379 | −0.367 | −0.348 | −0.277 | −0.173 | −0.058 |
| 65 | −0.257 | −0.279 | −0.283 | −0.276 | −0.262 | −0.206 | −0.125 | −0.046 |
| 66 | −0.230 | −0.241 | −0.239 | −0.228 | −0.213 | −0.164 | −0.097 | −0.036 |

Table ST18: Interaction energies for the S66x8 data set using MCML-v. The units are eV. Distances in the first row are relative to the equilibrium distance. The identifiers are defined in Tab. ST10.

| System | 0.900 | 0.950 | 1.000 | 1.050 | 1.100 | 1.250 | 1.500 | 2.000 |
|---|---|---|---|---|---|---|---|---|
| 1 | −0.630 | −0.684 | −0.698 | −0.685 | −0.657 | −0.540 | −0.352 | −0.127 |
| 2 | −0.752 | −0.808 | −0.825 | −0.815 | −0.787 | −0.660 | −0.448 | −0.200 |
| 3 | −0.842 | −0.886 | −0.891 | −0.875 | −0.841 | −0.681 | −0.430 | −0.164 |
| 4 | −0.810 | −0.861 | −0.873 | −0.860 | −0.827 | −0.680 | −0.444 | −0.182 |
| 5 | −0.169 | −0.191 | −0.197 | −0.192 | −0.181 | −0.137 | −0.073 | −0.018 |
| 6 | −0.141 | −0.179 | −0.188 | −0.180 | −0.164 | −0.106 | −0.042 | −0.009 |
| 7 | −0.234 | −0.253 | −0.251 | −0.237 | −0.218 | −0.156 | −0.078 | −0.021 |
| 8 | −0.053 | −0.100 | −0.117 | −0.118 | −0.110 | −0.073 | −0.030 | −0.007 |
| 9 | −0.047 | −0.128 | −0.157 | −0.158 | −0.145 | −0.085 | −0.021 | −0.002 |
| 10 | −0.062 | −0.121 | −0.144 | −0.146 | −0.136 | −0.089 | −0.034 | −0.006 |
| 11 | −0.057 | −0.093 | −0.103 | −0.099 | −0.088 | −0.049 | −0.010 | 0.001 |
| 12 | −0.085 | −0.119 | −0.128 | −0.125 | −0.114 | −0.076 | −0.034 | −0.010 |
| 13 | −0.126 | −0.151 | −0.158 | −0.153 | −0.140 | −0.093 | −0.040 | −0.009 |
| 14 | −0.198 | −0.217 | −0.218 | −0.208 | −0.193 | −0.138 | −0.068 | −0.019 |
| 15 | −0.066 | −0.109 | −0.123 | −0.122 | −0.113 | −0.073 | −0.029 | −0.006 |
| 16 | −0.161 | −0.219 | −0.237 | −0.233 | −0.218 | −0.155 | −0.075 | −0.023 |
| 17 | −0.070 | −0.118 | −0.135 | −0.135 | −0.126 | −0.085 | −0.038 | −0.011 |
| 18 | −0.067 | −0.154 | −0.183 | −0.183 | −0.168 | −0.104 | −0.032 | −0.005 |
| 19 | −0.207 | −0.280 | −0.300 | −0.291 | −0.267 | −0.171 | −0.061 | −0.008 |
| 20 | −0.183 | −0.191 | −0.186 | −0.174 | −0.158 | −0.108 | −0.053 | −0.016 |
| 21 | −0.001 | −0.048 | −0.071 | −0.079 | −0.076 | −0.053 | −0.022 | −0.005 |
| 22 | 0.005 | −0.041 | −0.061 | −0.066 | −0.064 | −0.046 | −0.020 | −0.005 |
| 23 | −0.033 | −0.058 | −0.066 | −0.066 | −0.061 | −0.040 | −0.015 | −0.003 |
| 24 | −0.240 | −0.257 | −0.256 | −0.244 | −0.227 | −0.167 | −0.088 | −0.024 |
| 25 | −0.059 | −0.069 | −0.071 | −0.067 | −0.061 | −0.040 | −0.018 | −0.005 |
| 26 | −0.053 | −0.081 | −0.088 | −0.086 | −0.078 | −0.048 | −0.017 | −0.003 |
| 27 | −0.108 | −0.121 | −0.124 | −0.121 | −0.114 | −0.086 | −0.049 | −0.019 |
| 28 | −0.127 | −0.151 | −0.159 | −0.158 | −0.151 | −0.116 | −0.052 | −0.014 |
| 29 | −0.121 | −0.133 | −0.134 | −0.129 | −0.121 | −0.089 | −0.047 | −0.015 |
| 30 | −0.202 | −0.224 | −0.229 | −0.225 | −0.214 | −0.140 | −0.056 | −0.017 |
| 31 | −0.141 | −0.163 | −0.170 | −0.168 | −0.160 | −0.121 | −0.064 | −0.018 |
| 32 | −0.297 | −0.319 | −0.323 | −0.314 | −0.297 | −0.232 | −0.139 | −0.049 |
| 33 | −0.289 | −0.315 | −0.322 | −0.316 | −0.301 | −0.238 | −0.144 | −0.052 |
| 34 | −0.255 | −0.272 | −0.273 | −0.263 | −0.248 | −0.193 | −0.115 | −0.041 |
| 35 | −0.360 | −0.381 | −0.384 | −0.374 | −0.356 | −0.285 | −0.166 | −0.045 |
| 36 | −0.275 | −0.301 | −0.309 | −0.304 | −0.291 | −0.232 | −0.144 | −0.054 |
| 37 | −0.233 | −0.247 | −0.246 | −0.236 | −0.222 | −0.172 | −0.102 | −0.038 |
| 38 | −0.013 | −0.035 | −0.044 | −0.046 | −0.044 | −0.030 | −0.013 | −0.004 |
| 39 | −0.010 | −0.056 | −0.074 | −0.077 | −0.073 | −0.050 | −0.021 | −0.005 |
| 40 | −0.116 | −0.140 | −0.146 | −0.142 | −0.131 | −0.090 | −0.039 | −0.008 |
| 41 | −0.106 | −0.120 | −0.123 | −0.119 | −0.111 | −0.078 | −0.029 | −0.005 |
| 42 | −0.028 | −0.087 | −0.112 | −0.118 | −0.113 | −0.079 | −0.033 | −0.007 |
| 43 | −0.106 | −0.126 | −0.130 | −0.126 | −0.117 | −0.081 | −0.034 | −0.006 |
| 44 | −0.256 | −0.285 | −0.294 | −0.292 | −0.281 | −0.231 | −0.148 | −0.059 |
| 45 | −0.242 | −0.263 | −0.268 | −0.263 | −0.252 | −0.204 | −0.129 | −0.053 |
| 46 | −0.121 | −0.155 | −0.166 | −0.165 | −0.155 | −0.111 | −0.044 | −0.009 |
| 47 | −0.338 | −0.363 | −0.369 | −0.363 | −0.350 | −0.291 | −0.194 | −0.073 |
| 48 | −0.210 | −0.227 | −0.230 | −0.225 | −0.215 | −0.173 | −0.110 | −0.048 |
| 49 | −0.083 | −0.113 | −0.121 | −0.117 | −0.106 | −0.065 | −0.020 | −0.001 |
| 50 | −0.113 | −0.133 | −0.141 | −0.141 | −0.135 | −0.107 | −0.063 | −0.023 |
| 51 | −0.023 | −0.085 | −0.120 | −0.123 | −0.113 | −0.073 | −0.032 | −0.008 |
| 52 | −0.077 | −0.120 | −0.137 | −0.138 | −0.131 | −0.093 | −0.043 | −0.013 |
| 53 | −0.095 | −0.176 | −0.204 | −0.203 | −0.189 | −0.122 | −0.042 | −0.008 |
| 54 | −0.213 | −0.319 | −0.346 | −0.334 | −0.302 | −0.191 | −0.076 | −0.021 |
| 55 | −0.106 | −0.159 | −0.175 | −0.171 | −0.156 | −0.100 | −0.037 | −0.007 |
| 56 | −0.143 | −0.173 | −0.179 | −0.172 | −0.158 | −0.105 | −0.043 | −0.009 |
| 57 | −0.175 | −0.207 | −0.211 | −0.202 | −0.184 | −0.122 | −0.050 | −0.011 |
| 58 | −0.119 | −0.160 | −0.169 | −0.163 | −0.148 | −0.094 | −0.036 | −0.007 |
| 59 | −0.139 | −0.191 | −0.207 | −0.202 | −0.182 | −0.107 | −0.035 | −0.006 |
| 60 | −0.671 | −0.728 | −0.743 | −0.731 | −0.701 | −0.574 | −0.369 | −0.145 |
| 61 | −0.406 | −0.478 | −0.492 | −0.472 | −0.435 | −0.299 | −0.137 | −0.039 |
| 62 | −0.283 | −0.302 | −0.303 | −0.294 | −0.278 | −0.217 | −0.130 | −0.047 |
| 63 | −0.257 | −0.271 | −0.270 | −0.259 | −0.243 | −0.186 | −0.109 | −0.039 |
| 64 | −0.374 | −0.391 | −0.390 | −0.378 | −0.358 | −0.285 | −0.179 | −0.060 |
| 65 | −0.267 | −0.289 | −0.293 | −0.285 | −0.270 | −0.213 | −0.130 | −0.048 |
| 66 | −0.235 | −0.246 | −0.243 | −0.233 | −0.217 | −0.167 | −0.099 | −0.037 |

Table ST19: Interaction energies for the S66x8 data set using VCML-v. The units are eV. Distances in the first row are relative to the equilibrium distance. The identifiers are defined in Tab. ST10.

| System | 0.900 | 0.950 | 1.000 | 1.050 | 1.100 | 1.250 | 1.500 | 2.000 |
|---|---|---|---|---|---|---|---|---|
| 1 | −0.567 | −0.630 | −0.652 | −0.649 | −0.629 | −0.529 | −0.354 | −0.129 |
| 2 | −0.687 | −0.751 | −0.776 | −0.774 | −0.754 | −0.646 | −0.449 | −0.202 |
| 3 | −0.776 | −0.829 | −0.840 | −0.832 | −0.804 | −0.662 | −0.428 | −0.167 |
| 4 | −0.743 | −0.803 | −0.822 | −0.817 | −0.792 | −0.663 | −0.443 | −0.185 |
| 5 | −0.148 | −0.176 | −0.187 | −0.186 | −0.179 | −0.139 | −0.076 | −0.019 |
| 6 | −0.113 | −0.161 | −0.177 | −0.175 | −0.163 | −0.110 | −0.044 | −0.010 |
| 7 | −0.211 | −0.235 | −0.238 | −0.229 | −0.213 | −0.157 | −0.081 | −0.022 |
| 8 | −0.030 | −0.086 | −0.110 | −0.115 | −0.111 | −0.077 | −0.032 | −0.008 |
| 9 | −0.012 | −0.104 | −0.142 | −0.150 | −0.142 | −0.089 | −0.024 | −0.002 |
| 10 | −0.030 | −0.101 | −0.134 | −0.142 | −0.137 | −0.095 | −0.037 | −0.007 |
| 11 | −0.033 | −0.077 | −0.093 | −0.094 | −0.086 | −0.051 | −0.012 | 0.001 |
| 12 | −0.065 | −0.106 | −0.122 | −0.122 | −0.115 | −0.079 | −0.035 | −0.010 |
| 13 | −0.103 | −0.136 | −0.148 | −0.148 | −0.139 | −0.097 | −0.042 | −0.010 |
| 14 | −0.176 | −0.202 | −0.208 | −0.202 | −0.190 | −0.140 | −0.071 | −0.020 |
| 15 | −0.042 | −0.096 | −0.117 | −0.121 | −0.115 | −0.079 | −0.032 | −0.007 |
| 16 | −0.129 | −0.197 | −0.223 | −0.226 | −0.215 | −0.158 | −0.079 | −0.024 |
| 17 | −0.047 | −0.103 | −0.127 | −0.132 | −0.126 | −0.089 | −0.040 | −0.012 |
| 18 | −0.030 | −0.128 | −0.167 | −0.174 | −0.165 | −0.108 | −0.034 | −0.005 |
| 19 | −0.161 | −0.248 | −0.280 | −0.279 | −0.261 | −0.175 | −0.066 | −0.009 |
| 20 | −0.167 | −0.180 | −0.178 | −0.169 | −0.155 | −0.110 | −0.054 | −0.016 |
| 21 | 0.021 | −0.037 | −0.070 | −0.083 | −0.084 | −0.061 | −0.026 | −0.006 |
| 22 | 0.026 | −0.032 | −0.059 | −0.070 | −0.071 | −0.053 | −0.024 | −0.006 |
| 23 | −0.020 | −0.052 | −0.066 | −0.069 | −0.066 | −0.045 | −0.018 | −0.004 |
| 24 | −0.215 | −0.238 | −0.241 | −0.234 | −0.220 | −0.166 | −0.090 | −0.025 |
| 25 | −0.052 | −0.066 | −0.070 | −0.068 | −0.062 | −0.042 | −0.019 | −0.005 |
| 26 | −0.039 | −0.073 | −0.085 | −0.086 | −0.080 | −0.051 | −0.019 | −0.003 |
| 27 | −0.094 | −0.112 | −0.118 | −0.118 | −0.113 | −0.088 | −0.050 | −0.019 |
| 28 | −0.103 | −0.133 | −0.147 | −0.150 | −0.146 | −0.117 | −0.054 | −0.015 |
| 29 | −0.106 | −0.122 | −0.128 | −0.126 | −0.120 | −0.091 | −0.049 | −0.015 |
| 30 | −0.175 | −0.203 | −0.215 | −0.215 | −0.208 | −0.143 | −0.058 | −0.017 |
| 31 | −0.116 | −0.145 | −0.158 | −0.160 | −0.155 | −0.123 | −0.067 | −0.018 |
| 32 | −0.275 | −0.300 | −0.307 | −0.301 | −0.287 | −0.229 | −0.140 | −0.050 |
| 33 | −0.266 | −0.295 | −0.306 | −0.303 | −0.291 | −0.235 | −0.146 | −0.053 |
| 34 | −0.233 | −0.255 | −0.259 | −0.253 | −0.241 | −0.191 | −0.117 | −0.042 |
| 35 | −0.332 | −0.359 | −0.366 | −0.360 | −0.345 | −0.282 | −0.169 | −0.046 |
| 36 | −0.252 | −0.281 | −0.293 | −0.291 | −0.280 | −0.229 | −0.145 | −0.055 |
| 37 | −0.213 | −0.231 | −0.234 | −0.227 | −0.215 | −0.170 | −0.104 | −0.039 |
| 38 | −0.007 | −0.036 | −0.049 | −0.052 | −0.051 | −0.036 | −0.016 | −0.004 |
| 39 | 0.010 | −0.048 | −0.074 | −0.082 | −0.080 | −0.057 | −0.024 | −0.006 |
| 40 | −0.095 | −0.129 | −0.142 | −0.142 | −0.135 | −0.097 | −0.043 | −0.009 |
| 41 | −0.091 | −0.113 | −0.121 | −0.120 | −0.114 | −0.084 | −0.032 | −0.005 |
| 42 | 0.003 | −0.071 | −0.107 | −0.120 | −0.120 | −0.089 | −0.038 | −0.009 |
| 43 | −0.090 | −0.116 | −0.126 | −0.125 | −0.118 | −0.085 | −0.036 | −0.007 |
| 44 | −0.226 | −0.261 | −0.275 | −0.276 | −0.270 | −0.229 | −0.151 | −0.061 |
| 45 | −0.214 | −0.241 | −0.251 | −0.251 | −0.244 | −0.203 | −0.131 | −0.054 |
| 46 | −0.094 | −0.139 | −0.159 | −0.164 | −0.158 | −0.118 | −0.049 | −0.010 |
| 47 | −0.307 | −0.338 | −0.350 | −0.349 | −0.340 | −0.290 | −0.197 | −0.075 |
| 48 | −0.188 | −0.209 | −0.217 | −0.216 | −0.209 | −0.173 | −0.111 | −0.048 |
| 49 | −0.059 | −0.096 | −0.111 | −0.111 | −0.103 | −0.067 | −0.022 | −0.002 |
| 50 | −0.092 | −0.118 | −0.131 | −0.134 | −0.132 | −0.108 | −0.065 | −0.024 |
| 51 | 0.009 | −0.064 | −0.110 | −0.120 | −0.114 | −0.076 | −0.033 | −0.009 |
| 52 | −0.053 | −0.104 | −0.128 | −0.134 | −0.131 | −0.097 | −0.046 | −0.013 |
| 53 | −0.056 | −0.149 | −0.187 | −0.194 | −0.184 | −0.125 | −0.045 | −0.009 |
| 54 | −0.161 | −0.284 | −0.325 | −0.322 | −0.298 | −0.195 | −0.080 | −0.021 |
| 55 | −0.073 | −0.140 | −0.166 | −0.169 | −0.160 | −0.107 | −0.042 | −0.009 |
| 56 | −0.118 | −0.156 | −0.169 | −0.167 | −0.156 | −0.107 | −0.046 | −0.010 |
| 57 | −0.150 | −0.189 | −0.200 | −0.195 | −0.181 | −0.124 | −0.053 | −0.011 |
| 58 | −0.094 | −0.146 | −0.163 | −0.162 | −0.150 | −0.100 | −0.040 | −0.008 |
| 59 | −0.102 | −0.168 | −0.195 | −0.199 | −0.185 | −0.115 | −0.039 | −0.007 |
| 60 | −0.606 | −0.672 | −0.696 | −0.692 | −0.671 | −0.562 | −0.371 | −0.147 |
| 61 | −0.353 | −0.442 | −0.468 | −0.459 | −0.429 | −0.305 | −0.144 | −0.040 |
| 62 | −0.263 | −0.284 | −0.289 | −0.283 | −0.269 | −0.214 | −0.132 | −0.048 |
| 63 | −0.236 | −0.255 | −0.257 | −0.249 | −0.236 | −0.185 | −0.111 | −0.040 |
| 64 | −0.348 | −0.370 | −0.373 | −0.364 | −0.348 | −0.282 | −0.181 | −0.061 |
| 65 | −0.246 | −0.270 | −0.278 | −0.273 | −0.261 | −0.209 | −0.131 | −0.049 |
| 66 | −0.217 | −0.232 | −0.232 | −0.224 | −0.212 | −0.166 | −0.100 | −0.037 |

Table ST20: Reference interaction energies for the S66x8 data set. The units are eV. Distances in the first row are relative to the equilibrium distance. The identifiers are defined in Tab. ST10.

| System | 0.900 | 0.950 | 1.000 | 1.050 | 1.100 | 1.250 | 1.500 | 2.000 |
|---|---|---|---|---|---|---|---|---|
| 1 | −0.665 | −0.710 | −0.718 | −0.702 | −0.671 | −0.544 | −0.349 | −0.131 |
| 2 | −0.788 | −0.837 | −0.848 | −0.833 | −0.802 | −0.667 | −0.448 | −0.203 |
| 3 | −0.779 | −0.834 | −0.844 | −0.826 | −0.790 | −0.639 | −0.403 | −0.157 |
| 4 | −0.799 | −0.851 | −0.862 | −0.845 | −0.811 | −0.664 | −0.432 | −0.181 |
| 5 | −0.167 | −0.187 | −0.191 | −0.185 | −0.174 | −0.130 | −0.072 | −0.021 |
| 6 | −0.117 | −0.155 | −0.165 | −0.159 | −0.145 | −0.098 | −0.045 | −0.012 |
| 7 | −0.173 | −0.200 | −0.205 | −0.199 | −0.186 | −0.137 | −0.075 | −0.025 |
| 8 | −0.072 | −0.113 | −0.126 | −0.124 | −0.115 | −0.078 | −0.037 | −0.010 |
| 9 | −0.005 | −0.087 | −0.118 | −0.122 | −0.113 | −0.068 | −0.022 | −0.003 |
| 10 | −0.093 | −0.141 | −0.155 | −0.151 | −0.139 | −0.091 | −0.040 | −0.009 |
| 11 | −0.005 | −0.044 | −0.059 | −0.059 | −0.054 | −0.030 | −0.008 | 0.000 |
| 12 | −0.080 | −0.114 | −0.124 | −0.121 | −0.112 | −0.078 | −0.039 | −0.012 |
| 13 | −0.107 | −0.132 | −0.139 | −0.135 | −0.124 | −0.085 | −0.041 | −0.012 |
| 14 | −0.148 | −0.174 | −0.181 | −0.176 | −0.165 | −0.122 | −0.067 | −0.023 |
| 15 | −0.081 | −0.116 | −0.126 | −0.122 | −0.112 | −0.075 | −0.034 | −0.009 |
| 16 | −0.163 | −0.216 | −0.230 | −0.225 | −0.209 | −0.150 | −0.080 | −0.027 |
| 17 | −0.091 | −0.133 | −0.145 | −0.143 | −0.133 | −0.092 | −0.047 | −0.015 |
| 18 | −0.026 | −0.114 | −0.146 | −0.148 | −0.137 | −0.087 | −0.033 | −0.007 |
| 19 | −0.151 | −0.227 | −0.249 | −0.243 | −0.223 | −0.146 | −0.061 | −0.012 |
| 20 | −0.120 | −0.138 | −0.141 | −0.135 | −0.126 | −0.091 | −0.050 | −0.018 |
| 21 | −0.100 | −0.126 | −0.132 | −0.126 | −0.114 | −0.075 | −0.035 | −0.009 |
| 22 | −0.072 | −0.100 | −0.106 | −0.102 | −0.094 | −0.064 | −0.031 | −0.008 |
| 23 | −0.071 | −0.085 | −0.086 | −0.081 | −0.073 | −0.047 | −0.021 | −0.005 |
| 24 | −0.189 | −0.210 | −0.213 | −0.205 | −0.191 | −0.141 | −0.077 | −0.024 |
| 25 | −0.052 | −0.064 | −0.066 | −0.063 | −0.058 | −0.041 | −0.020 | −0.006 |
| 26 | −0.045 | −0.068 | −0.074 | −0.071 | −0.065 | −0.042 | −0.018 | −0.004 |
| 27 | −0.113 | −0.125 | −0.126 | −0.122 | −0.114 | −0.087 | −0.051 | −0.020 |
| 28 | −0.162 | −0.178 | −0.181 | −0.174 | −0.163 | −0.121 | −0.057 | −0.017 |
| 29 | −0.124 | −0.134 | −0.133 | −0.127 | −0.117 | −0.086 | −0.048 | −0.017 |
| 30 | −0.217 | −0.235 | −0.236 | −0.229 | −0.216 | −0.140 | −0.061 | −0.020 |
| 31 | −0.149 | −0.168 | −0.172 | −0.167 | −0.157 | −0.118 | −0.066 | −0.022 |
| 32 | −0.296 | −0.315 | −0.317 | −0.307 | −0.290 | −0.227 | −0.137 | −0.052 |
| 33 | −0.306 | −0.327 | −0.330 | −0.320 | −0.304 | −0.239 | −0.145 | −0.055 |
| 34 | −0.234 | −0.251 | −0.253 | −0.245 | −0.231 | −0.181 | −0.110 | −0.044 |
| 35 | −0.338 | −0.359 | −0.361 | −0.352 | −0.336 | −0.270 | −0.159 | −0.048 |
| 36 | −0.301 | −0.323 | −0.326 | −0.318 | −0.302 | −0.240 | −0.148 | −0.058 |
| 37 | −0.203 | −0.218 | −0.220 | −0.212 | −0.201 | −0.157 | −0.096 | −0.039 |
| 38 | −0.064 | −0.076 | −0.078 | −0.074 | −0.067 | −0.046 | −0.022 | −0.006 |
| 39 | −0.083 | −0.110 | −0.115 | −0.109 | −0.099 | −0.066 | −0.031 | −0.008 |
| 40 | −0.139 | −0.153 | −0.153 | −0.145 | −0.133 | −0.093 | −0.046 | −0.012 |
| 41 | −0.119 | −0.127 | −0.126 | −0.120 | −0.110 | −0.079 | −0.035 | −0.008 |
| 42 | −0.127 | −0.159 | −0.166 | −0.158 | −0.145 | −0.098 | −0.046 | −0.012 |
| 43 | −0.113 | −0.128 | −0.130 | −0.124 | −0.115 | −0.081 | −0.039 | −0.008 |
| 44 | −0.301 | −0.323 | −0.327 | −0.319 | −0.304 | −0.244 | −0.155 | −0.065 |
| 45 | −0.252 | −0.270 | −0.272 | −0.265 | −0.252 | −0.202 | −0.129 | −0.057 |
| 46 | −0.165 | −0.185 | −0.186 | −0.178 | −0.164 | −0.115 | −0.053 | −0.013 |
| 47 | −0.356 | −0.377 | −0.380 | −0.372 | −0.356 | −0.292 | −0.193 | −0.078 |
| 48 | −0.208 | −0.223 | −0.225 | −0.219 | −0.208 | −0.166 | −0.107 | −0.049 |
| 49 | −0.033 | −0.067 | −0.078 | −0.078 | −0.072 | −0.045 | −0.016 | −0.002 |
| 50 | −0.161 | −0.175 | −0.178 | −0.173 | −0.163 | −0.125 | −0.073 | −0.027 |
| 51 | −0.130 | −0.172 | −0.185 | −0.172 | −0.152 | −0.097 | −0.045 | −0.012 |
| 52 | −0.111 | −0.145 | −0.155 | −0.151 | −0.141 | −0.101 | −0.052 | −0.017 |
| 53 | −0.052 | −0.135 | −0.165 | −0.168 | −0.156 | −0.104 | −0.043 | −0.011 |
| 54 | −0.160 | −0.268 | −0.297 | −0.288 | −0.262 | −0.171 | −0.079 | −0.024 |
| 55 | −0.136 | −0.176 | −0.183 | −0.173 | −0.157 | −0.102 | −0.046 | −0.011 |
| 56 | −0.109 | −0.139 | −0.146 | −0.140 | −0.129 | −0.087 | −0.041 | −0.011 |
| 57 | −0.117 | −0.152 | −0.161 | −0.155 | −0.142 | −0.097 | −0.046 | −0.012 |
| 58 | −0.128 | −0.160 | −0.164 | −0.155 | −0.140 | −0.091 | −0.041 | −0.011 |
| 59 | −0.171 | −0.208 | −0.214 | −0.203 | −0.180 | −0.109 | −0.044 | −0.010 |
| 60 | −0.704 | −0.753 | −0.762 | −0.747 | −0.714 | −0.579 | −0.367 | −0.147 |
| 61 | −0.346 | −0.418 | −0.433 | −0.416 | −0.384 | −0.270 | −0.139 | −0.045 |
| 62 | −0.285 | −0.301 | −0.300 | −0.290 | −0.274 | −0.214 | −0.129 | −0.050 |
| 63 | −0.230 | −0.244 | −0.244 | −0.236 | −0.222 | −0.172 | −0.104 | −0.041 |
| 64 | −0.336 | −0.353 | −0.353 | −0.343 | −0.326 | −0.261 | −0.167 | −0.062 |
| 65 | −0.283 | −0.300 | −0.300 | −0.291 | −0.275 | −0.215 | −0.131 | −0.052 |
| 66 | −0.202 | −0.215 | −0.215 | −0.207 | −0.195 | −0.151 | −0.092 | −0.038 |

Table ST21: Systems in the W4-11 data set. Identifiers are provided, which are used in Tab. ST22 and Figs. SF4 (PBE, PBE-D3), SF7 (MS2, MCML), SF10 (SCAN, r$^2$SCAN), and SF13 (all functionals using rVV10).

| Identifier | System |
|---|---|
| 1 | $H_3C{-}C(=O)H$ |
| 2 | $CH_3C(=O)OH$ |
| 3 | AlCl |
| 4 | $AlCl_3$ |
| 5 | AlF |
| 6 | $AlF_3$ |
| 7 | AlH |
| 8 | $AlH_3$ |
| 9 | $H_2C{=}C{=}CH_2$ |
| 10 | $B_2$ |
| 11 | $B_2H_6$ |
| 12 | $Be_2$ |
| 13 | $BeCl_2$ |
| 14 | $BeF_2$ |
| 15 | BF |
| 16 | $BF_3$ |
| 17 | BH |
| 18 | $BH_3$ |
| 19 | $HBF_2$ |
| 20 | BN $^1\Sigma^+$ |
| 21 | BN $^3\Pi$ |
| 22 | cis-H(HO)$C^{\bullet\bullet}$ |
| 23 | cis-HON=O |
| 24 | cis-$HO_3^{\bullet}$ |
| 25 | cis-$H_2N_2$ |
| 26 | $C_2$ |
| 27 | $C_2H_2$ |
| 28 | $C_2H_3F$ |
| 29 | $C_2H_4$ |
| 30 | $C_2H_5F$ |
| 31 | $C_2H_6$ |
| 32 | $C{\equiv}C^{\bullet}$ |
| 33 | $Cl_2C^{\bullet\bullet}$ |
| 34 | $FC^{\bullet}$ |
| 35 | $^{\bullet\bullet}CF_2$ |
| 36 | $CF_4$ |
| 37 | $HC^{\bullet}$ |
| 38 | $H_2C^{\bullet\bullet}$ ($^1A_1$) |
| 39 | $H_2C^{\bullet\bullet}$ ($^3B_2$) |
| 40 | $H_2C{=}C^{\bullet\bullet}$ |
| 41 | $H_2C{=}HC^{\bullet}$ |
| 42 | $CH_2F_2$ |
| 43 | $H_2C{=}NH$ |
| 44 | $H_2N{-}CH_2^{\bullet}$ |
| 45 | $H_3C^{\bullet}$ |
| 46 | $CH_3F$ |
| 47 | $H_3C{-}NH^{\bullet}$ |

Table ST21: Systems in the W4-11 data set. Continued.

| Identifier | System |
|---|---|
| 48 | $CH_3NH_2$ |
| 49 | $CH_4$ |
| 50 | $Cl_2$ |
| 51 | ClOCl |
| 52 | ClC≡N |
| 53 | ClF |
| 54 | $ClO^{\bullet}$ |
| 55 | $OOCl^{\bullet}$ |
| 56 | $N{\equiv}C^{\bullet}$ |
| 57 | CO |
| 58 | $CO_2$ |
| 59 | CS |
| 60 | $CS_2$ |
| 61 | $H_2CO_2$ |
| 62 | $C_2H_5OH$ |
| 63 | $F_2$ |
| 64 | $F_2C{=}O$ |
| 65 | FOF |
| 66 | FC≡CF |
| 67 | $OOF^{\bullet}$ |
| 68 | $F_2O_2$ |
| 69 | HC(=O)OH |
| 70 | H(O=)C−C(=O)H |
| 71 | $H_2$ |
| 72 | $H_2C{=}N^{\bullet}$ |
| 73 | $H_2C{=}O$ |
| 74 | $H_2O$ |
| 75 | $H_2S$ |
| 76 | HC≡CF |
| 77 | HCl |
| 78 | HCN |
| 79 | $HN{=}CH^{\bullet}$ |
| 80 | HCNO |
| 81 | $H(O{=})C^{\bullet}$ |
| 82 | HC(=O)F |
| 83 | HF |
| 84 | $HNC^{\bullet\bullet}$ |
| 85 | HNCO |
| 86 | $HN_3$ |
| 87 | HN=O |
| 88 | HOCl |
| 89 | HOCN |
| 90 | HOF |
| 91 | $HONC^{\bullet\bullet}$ |
| 92 | $HOO^{\bullet}$ |
| 93 | $H_2O_2$ |
| 94 | $HS^{\bullet}$ |

Table ST21: Systems in the W4-11 data set. Continued.

| Identifier | System |
|---|---|
| 95 | $H_2C{=}C{=}O$ |
| 96 | $CH_3OH$ |
| 97 | $N_2$ |
| 98 | $HN{\equiv}N^\bullet$ |
| 99 | $N_2H_4$ |
| 100 | $N{\equiv}N\text{-}O$ |
| 101 | $N{\equiv}C{-}C{\equiv}N$ |
| 102 | $NH^\bullet$ |
| 103 | $H_2N^\bullet$ |
| 104 | $H_2NCl$ |
| 105 | $NH_3$ |
| 106 | $ON^\bullet$ |
| 107 | $O_2N^\bullet$ |
| 108 | $O_2^{\bullet\bullet}$ |
| 109 | $O_3$ |
| 110 | $O_2Cl^\bullet$ |
| 111 | OCS |
| 112 | $FO^\bullet$ |
| 113 | $HO^\bullet$ |
| 114 | $C_2H_4O$ |
| 115 | $H_2C_2O$ |
| 116 | $P_2$ |
| 117 | $P_4$ |
| 118 | $PH_3$ |
| 119 | $C_3H_8$ |
| 120 | $C_3H_6$ |
| 121 | $C_3H_4$ |
| 122 | $S_2^{\bullet\bullet}$ |
| 123 | SSO |
| 124 | $S_3$ |
| 125 | $S_4$ |
| 126 | $Si_2H_6$ |
| 127 | $FSi^\bullet$ |
| 128 | $SiF_4$ |
| 129 | $HSi^\bullet$ |
| 130 | $SiH_3F$ |
| 131 | $SiH_4$ |
| 132 | SiO |
| 133 | $SO^{\bullet\bullet}$ |
| 134 | $SO_2$ |
| 135 | $SO_3$ |
| 136 | $HSS^\bullet$ |
| 137 | trans-$H(HO)C^{\bullet\bullet}$ |
| 138 | trans-$HON{=}O$ |
| 139 | trans-$HO_3^\bullet$ |
| 140 | trans-$N_2H_2$ |

Table ST22: Atomization energies for the W4-11 data set. Functionals with '-v' employ the rVV10 methodology. The units are eV, and the reference values are provided in the last column. The identifiers are defined in Tab. ST21.

| System | PBE | PBE-D3 | MS2 | SCAN | $r^2$SCAN | SCAN-v | MCML | MCML-v | VCML-v | REF |
|---|---|---|---|---|---|---|---|---|---|---|
| 1 | 29.993 | 30.021 | 29.098 | 29.280 | 29.251 | 29.312 | 28.738 | 28.761 | 28.745 | 29.395 |
| 2 | 35.715 | 35.760 | 34.172 | 34.729 | 34.713 | 34.778 | 33.977 | 34.012 | 34.023 | 34.865 |
| 3 | 5.213 | 5.213 | 4.953 | 5.146 | 5.149 | 5.156 | 4.869 | 4.877 | 4.900 | 5.317 |
| 4 | 13.205 | 13.242 | 12.750 | 13.367 | 13.391 | 13.409 | 12.431 | 12.463 | 12.527 | 13.558 |
| 5 | 7.057 | 7.057 | 6.500 | 6.883 | 6.921 | 6.890 | 6.471 | 6.475 | 6.514 | 7.102 |
| 6 | 18.425 | 18.438 | 16.953 | 18.242 | 18.388 | 18.268 | 16.711 | 16.728 | 16.865 | 18.689 |
| 7 | 2.993 | 2.993 | 3.093 | 3.026 | 3.021 | 3.027 | 3.013 | 3.014 | 2.995 | 3.190 |
| 8 | 8.803 | 8.809 | 9.202 | 9.184 | 9.170 | 9.190 | 8.917 | 8.921 | 8.877 | 9.244 |
| 9 | 31.349 | 31.369 | 30.495 | 30.598 | 30.570 | 30.627 | 29.949 | 29.970 | 29.932 | 30.533 |
| 10 | 3.324 | 3.324 | 3.202 | 3.022 | 3.069 | 3.028 | 2.888 | 2.891 | 2.893 | 2.925 |
| 11 | 26.355 | 26.381 | 26.735 | 26.752 | 26.601 | 26.775 | 26.263 | 26.279 | 26.098 | 26.323 |
| 12 | 0.420 | 0.424 | 0.363 | 0.372 | 0.367 | 0.376 | 0.291 | 0.304 | 0.276 | 0.116 |
| 13 | 9.939 | 9.951 | 9.521 | 9.998 | 9.998 | 10.013 | 9.308 | 9.325 | 9.346 | 9.769 |
| 14 | 13.714 | 13.718 | 12.538 | 13.500 | 13.584 | 13.509 | 12.403 | 12.414 | 12.479 | 13.404 |
| 15 | 8.021 | 8.021 | 7.358 | 7.736 | 7.763 | 7.742 | 7.404 | 7.407 | 7.452 | 7.915 |
| 16 | 20.628 | 20.637 | 18.886 | 20.166 | 20.252 | 20.193 | 18.800 | 18.818 | 18.954 | 20.423 |
| 17 | 3.511 | 3.511 | 3.592 | 3.448 | 3.435 | 3.450 | 3.470 | 3.471 | 3.470 | 3.686 |
| 18 | 12.064 | 12.067 | 12.325 | 12.277 | 12.244 | 12.282 | 12.058 | 12.061 | 12.004 | 12.198 |
| 19 | 17.978 | 17.990 | 16.904 | 17.714 | 17.749 | 17.732 | 16.752 | 16.764 | 16.834 | 17.822 |
| 20 | 4.843 | 4.843 | 4.073 | 3.929 | 3.939 | 3.935 | 4.082 | 4.087 | 4.096 | 4.564 |
| 21 | 5.305 | 5.305 | 5.136 | 4.933 | 4.904 | 4.939 | 5.217 | 5.221 | 5.116 | 4.589 |
| 22 | 14.141 | 14.144 | 13.429 | 13.559 | 13.562 | 13.573 | 13.337 | 13.347 | 13.381 | 13.774 |
| 23 | 14.753 | 14.758 | 13.248 | 13.252 | 13.415 | 13.277 | 13.508 | 13.526 | 13.559 | 13.539 |
| 24 | 11.569 | 11.575 | 9.996 | 10.193 | 10.379 | 10.219 | 10.396 | 10.414 | 10.391 | 10.108 |
| 25 | 13.370 | 13.372 | 12.895 | 12.274 | 12.312 | 12.288 | 12.877 | 12.886 | 12.780 | 12.625 |
| 26 | 6.222 | 6.222 | 5.161 | 5.221 | 5.268 | 5.227 | 4.992 | 4.996 | 5.129 | 6.375 |
| 27 | 17.963 | 17.968 | 17.269 | 17.399 | 17.397 | 17.411 | 16.964 | 16.973 | 16.986 | 17.585 |
| 28 | 25.486 | 25.506 | 24.520 | 24.856 | 24.794 | 24.883 | 24.059 | 24.078 | 24.122 | 24.886 |
| 29 | 24.755 | 24.767 | 24.376 | 24.377 | 24.340 | 24.396 | 23.898 | 23.911 | 23.867 | 24.462 |
| 30 | 31.651 | 31.689 | 30.979 | 31.259 | 31.157 | 31.295 | 30.364 | 30.390 | 30.386 | 31.287 |
| 31 | 31.049 | 31.076 | 30.881 | 30.889 | 30.812 | 30.915 | 30.287 | 30.306 | 30.218 | 30.922 |
| 32 | 11.985 | 11.986 | 11.308 | 11.503 | 11.502 | 11.512 | 11.095 | 11.101 | 11.128 | 11.542 |
| 33 | 8.423 | 8.428 | 7.617 | 7.717 | 7.738 | 7.743 | 7.497 | 7.517 | 7.621 | 7.691 |
| 34 | 6.199 | 6.199 | 5.456 | 5.734 | 5.756 | 5.741 | 5.333 | 5.337 | 5.454 | 5.755 |
| 35 | 11.809 | 11.811 | 10.422 | 11.023 | 11.034 | 11.041 | 10.266 | 10.278 | 10.484 | 11.222 |
| 36 | 21.431 | 21.443 | 18.964 | 20.440 | 20.458 | 20.492 | 18.718 | 18.754 | 19.128 | 20.761 |
| 37 | 3.675 | 3.675 | 3.735 | 3.558 | 3.619 | 3.560 | 3.552 | 3.553 | 3.563 | 3.652 |
| 38 | 7.745 | 7.745 | 7.807 | 7.599 | 7.576 | 7.603 | 7.588 | 7.591 | 7.575 | 7.869 |
| 39 | 8.435 | 8.435 | 8.335 | 8.534 | 8.541 | 8.538 | 8.087 | 8.090 | 8.098 | 8.271 |
| 40 | 15.997 | 15.999 | 15.565 | 15.492 | 15.478 | 15.505 | 15.321 | 15.330 | 15.314 | 15.608 |
| 41 | 19.835 | 19.842 | 19.416 | 19.531 | 19.494 | 19.547 | 19.037 | 19.048 | 19.016 | 19.344 |
| 42 | 19.388 | 19.402 | 18.244 | 18.846 | 18.799 | 18.872 | 17.846 | 17.864 | 18.013 | 18.979 |
| 43 | 19.559 | 19.566 | 19.138 | 18.878 | 18.853 | 18.894 | 18.885 | 18.896 | 18.823 | 19.056 |
| 44 | 21.499 | 21.511 | 21.101 | 21.040 | 20.992 | 21.060 | 20.818 | 20.832 | 20.708 | 20.913 |
| 45 | 13.437 | 13.438 | 13.416 | 13.549 | 13.508 | 13.555 | 13.116 | 13.120 | 13.092 | 13.351 |
| 46 | 18.540 | 18.550 | 17.999 | 18.265 | 18.203 | 18.281 | 17.605 | 17.616 | 17.660 | 18.341 |
| 47 | 21.110 | 21.121 | 21.007 | 20.757 | 20.677 | 20.777 | 20.679 | 20.694 | 20.570 | 20.582 |

Table ST22: Atomization energies for the W4-11 data set. Continued.

| System | PBE | PBE-D3 | MS2 | SCAN | $r^2$SCAN | SCAN-v | MCML | MCML-v | VCML-v | REF |
|---|---|---|---|---|---|---|---|---|---|---|
| 48 | 25.590 | 25.608 | 25.293 | 25.112 | 25.056 | 25.136 | 24.946 | 24.963 | 24.825 | 25.251 |
| 49 | 18.196 | 18.198 | 18.151 | 18.175 | 18.146 | 18.184 | 17.807 | 17.814 | 17.765 | 18.231 |
| 50 | 2.856 | 2.856 | 2.489 | 2.455 | 2.477 | 2.469 | 2.474 | 2.484 | 2.506 | 2.591 |
| 51 | 5.186 | 5.190 | 4.452 | 4.359 | 4.371 | 4.388 | 4.637 | 4.658 | 4.629 | 4.400 |
| 52 | 13.261 | 13.267 | 12.303 | 12.160 | 12.199 | 12.180 | 12.255 | 12.270 | 12.302 | 12.378 |
| 53 | 3.128 | 3.128 | 2.561 | 2.651 | 2.639 | 2.661 | 2.540 | 2.547 | 2.603 | 2.723 |
| 54 | 3.533 | 3.533 | 3.040 | 3.005 | 3.006 | 3.016 | 3.195 | 3.203 | 3.170 | 2.838 |
| 55 | 6.812 | 6.818 | 5.424 | 5.618 | 5.750 | 5.641 | 5.657 | 5.673 | 5.735 | 5.481 |
| 56 | 8.514 | 8.514 | 7.857 | 7.643 | 7.664 | 7.650 | 7.829 | 7.834 | 7.856 | 7.864 |
| 57 | 11.507 | 11.507 | 10.693 | 10.841 | 10.897 | 10.848 | 10.788 | 10.793 | 10.880 | 11.263 |
| 58 | 17.777 | 17.779 | 16.093 | 16.642 | 16.772 | 16.660 | 16.155 | 16.167 | 16.334 | 16.918 |
| 59 | 7.787 | 7.787 | 7.213 | 7.228 | 7.267 | 7.237 | 7.213 | 7.220 | 7.281 | 7.468 |
| 60 | 13.108 | 13.114 | 12.133 | 12.358 | 12.441 | 12.382 | 12.107 | 12.124 | 12.196 | 12.176 |
| 61 | 18.684 | 18.695 | 17.767 | 17.682 | 17.683 | 17.712 | 17.767 | 17.788 | 17.725 | 17.780 |
| 62 | 35.532 | 35.578 | 34.822 | 35.066 | 34.979 | 35.107 | 34.373 | 34.403 | 34.318 | 35.179 |
| 63 | 2.245 | 2.245 | 1.495 | 1.582 | 1.644 | 1.590 | 1.516 | 1.521 | 1.583 | 1.693 |
| 64 | 19.103 | 19.110 | 17.011 | 17.998 | 18.047 | 18.031 | 16.930 | 16.952 | 17.209 | 18.241 |
| 65 | 5.262 | 5.265 | 3.948 | 4.099 | 4.228 | 4.120 | 4.087 | 4.101 | 4.163 | 4.067 |
| 66 | 17.817 | 17.827 | 15.770 | 16.545 | 16.522 | 16.571 | 15.500 | 15.518 | 15.747 | 16.742 |
| 67 | 7.395 | 7.399 | 5.737 | 5.988 | 6.186 | 6.009 | 5.973 | 5.987 | 6.080 | 5.842 |
| 68 | 8.781 | 8.790 | 6.665 | 6.951 | 7.160 | 6.986 | 6.904 | 6.928 | 7.046 | 6.607 |
| 69 | 22.471 | 22.484 | 21.060 | 21.573 | 21.597 | 21.600 | 21.069 | 21.088 | 21.155 | 21.764 |
| 70 | 28.538 | 28.567 | 26.984 | 27.263 | 27.281 | 27.301 | 26.840 | 26.867 | 26.915 | 27.541 |
| 71 | 4.539 | 4.539 | 4.600 | 4.667 | 4.668 | 4.668 | 4.585 | 4.585 | 4.614 | 4.748 |
| 72 | 15.554 | 15.556 | 15.272 | 15.002 | 14.953 | 15.015 | 15.081 | 15.090 | 15.020 | 14.906 |
| 73 | 16.625 | 16.630 | 15.912 | 16.036 | 16.045 | 16.049 | 15.767 | 15.776 | 15.804 | 16.247 |
| 74 | 10.094 | 10.094 | 9.482 | 9.825 | 9.877 | 9.830 | 9.554 | 9.557 | 9.544 | 10.103 |
| 75 | 7.902 | 7.902 | 7.881 | 7.875 | 7.869 | 7.880 | 7.836 | 7.840 | 7.790 | 7.975 |
| 76 | 18.014 | 18.021 | 16.631 | 17.110 | 17.097 | 17.129 | 16.350 | 16.363 | 16.486 | 17.279 |
| 77 | 4.616 | 4.616 | 4.437 | 4.534 | 4.542 | 4.537 | 4.373 | 4.375 | 4.385 | 4.662 |
| 78 | 14.088 | 14.089 | 13.477 | 13.267 | 13.279 | 13.276 | 13.379 | 13.386 | 13.372 | 13.591 |
| 79 | 15.322 | 15.325 | 14.795 | 14.634 | 14.616 | 14.647 | 14.626 | 14.636 | 14.581 | 14.581 |
| 80 | 17.249 | 17.256 | 15.592 | 15.740 | 15.890 | 15.761 | 15.553 | 15.568 | 15.618 | 15.827 |
| 81 | 12.683 | 12.686 | 11.883 | 12.080 | 12.107 | 12.090 | 11.846 | 11.853 | 11.902 | 12.117 |
| 82 | 18.184 | 18.191 | 16.778 | 17.328 | 17.347 | 17.350 | 16.648 | 16.663 | 16.805 | 17.508 |
| 83 | 6.081 | 6.081 | 5.422 | 5.856 | 5.909 | 5.858 | 5.346 | 5.347 | 5.430 | 6.142 |
| 84 | 13.467 | 13.468 | 12.836 | 12.689 | 12.691 | 12.699 | 12.780 | 12.787 | 12.763 | 12.931 |
| 85 | 19.979 | 19.987 | 18.574 | 18.766 | 18.830 | 18.786 | 18.558 | 18.573 | 18.609 | 18.852 |
| 86 | 16.067 | 16.073 | 14.946 | 14.304 | 14.387 | 14.325 | 15.037 | 15.053 | 14.964 | 14.388 |
| 87 | 9.561 | 9.562 | 8.800 | 8.491 | 8.588 | 8.502 | 8.931 | 8.938 | 8.906 | 8.928 |
| 88 | 7.571 | 7.573 | 6.945 | 7.035 | 7.062 | 7.049 | 7.061 | 7.071 | 7.042 | 7.208 |
| 89 | 18.690 | 18.698 | 17.374 | 17.479 | 17.517 | 17.499 | 17.423 | 17.438 | 17.451 | 17.782 |
| 90 | 7.397 | 7.398 | 6.567 | 6.714 | 6.782 | 6.726 | 6.667 | 6.675 | 6.670 | 6.880 |
| 91 | 16.229 | 16.238 | 14.912 | 14.906 | 15.001 | 14.927 | 15.020 | 15.035 | 15.034 | 15.184 |
| 92 | 8.359 | 8.360 | 7.502 | 7.626 | 7.698 | 7.638 | 7.755 | 7.763 | 7.717 | 7.612 |
| 93 | 12.132 | 12.136 | 11.195 | 11.402 | 11.486 | 11.418 | 11.424 | 11.435 | 11.361 | 11.669 |
| 94 | 3.824 | 3.824 | 3.855 | 3.847 | 3.846 | 3.849 | 3.876 | 3.878 | 3.829 | 3.804 |

Table ST22: Atomization energies for the W4-11 data set. Continued.

| System | PBE | PBE-D3 | MS2 | SCAN | $r^2$SCAN | SCAN-v | MCML | MCML-v | VCML-v | REF |
|---|---|---|---|---|---|---|---|---|---|---|
| 95 | 24.053 | 24.066 | 22.769 | 23.122 | 23.159 | 23.145 | 22.550 | 22.567 | 22.626 | 23.133 |
| 96 | 22.475 | 22.490 | 21.889 | 22.120 | 22.079 | 22.140 | 21.662 | 21.676 | 21.638 | 22.267 |
| 97 | 10.405 | 10.405 | 9.941 | 9.334 | 9.366 | 9.341 | 10.084 | 10.089 | 10.040 | 9.908 |
| 98 | 10.654 | 10.654 | 10.205 | 9.662 | 9.667 | 9.672 | 10.266 | 10.274 | 10.183 | 9.751 |
| 99 | 19.609 | 19.620 | 19.180 | 18.742 | 18.748 | 18.764 | 19.088 | 19.104 | 18.908 | 19.006 |
| 100 | 13.264 | 13.267 | 11.777 | 11.504 | 11.688 | 11.523 | 11.954 | 11.967 | 11.987 | 11.745 |
| 101 | 23.230 | 23.240 | 21.849 | 21.406 | 21.435 | 21.431 | 21.752 | 21.770 | 21.753 | 21.770 |
| 102 | 3.834 | 3.834 | 3.900 | 3.681 | 3.678 | 3.683 | 3.777 | 3.778 | 3.747 | 3.603 |
| 103 | 8.169 | 8.169 | 8.213 | 7.982 | 7.961 | 7.986 | 8.149 | 8.152 | 8.050 | 7.918 |
| 104 | 11.190 | 11.195 | 10.840 | 10.585 | 10.589 | 10.602 | 10.778 | 10.791 | 10.705 | 10.757 |
| 105 | 13.076 | 13.076 | 12.839 | 12.723 | 12.732 | 12.730 | 12.775 | 12.780 | 12.664 | 12.923 |
| 106 | 7.293 | 7.293 | 6.555 | 6.341 | 6.414 | 6.349 | 6.730 | 6.735 | 6.755 | 6.624 |
| 107 | 11.461 | 11.463 | 9.822 | 9.837 | 10.058 | 9.857 | 10.064 | 10.078 | 10.144 | 9.882 |
| 108 | 6.062 | 6.062 | 5.015 | 5.265 | 5.429 | 5.274 | 5.262 | 5.268 | 5.315 | 5.239 |
| 109 | 7.829 | 7.830 | 6.001 | 6.097 | 6.351 | 6.120 | 6.431 | 6.446 | 6.519 | 6.393 |
| 110 | 6.989 | 6.993 | 5.647 | 5.912 | 5.999 | 5.937 | 5.886 | 5.904 | 5.946 | 5.556 |
| 111 | 15.481 | 15.484 | 14.181 | 14.543 | 14.644 | 14.563 | 14.204 | 14.218 | 14.337 | 14.559 |
| 112 | 3.050 | 3.050 | 2.368 | 2.419 | 2.456 | 2.428 | 2.490 | 2.496 | 2.507 | 2.301 |
| 113 | 4.728 | 4.728 | 4.586 | 4.646 | 4.652 | 4.649 | 4.719 | 4.721 | 4.644 | 4.649 |
| 114 | 28.959 | 28.983 | 28.146 | 28.245 | 28.195 | 28.280 | 27.762 | 27.787 | 27.746 | 28.253 |
| 115 | 20.724 | 20.739 | 19.607 | 19.680 | 19.684 | 19.706 | 19.425 | 19.444 | 19.423 | 19.777 |
| 116 | 5.280 | 5.280 | 4.957 | 4.865 | 4.916 | 4.878 | 4.879 | 4.888 | 4.872 | 5.099 |
| 117 | 13.465 | 13.466 | 12.978 | 12.711 | 12.765 | 12.774 | 12.746 | 12.793 | 12.740 | 12.601 |
| 118 | 10.378 | 10.381 | 10.681 | 10.500 | 10.447 | 10.508 | 10.415 | 10.421 | 10.336 | 10.506 |
| 119 | 43.967 | 44.032 | 43.679 | 43.690 | 43.565 | 43.739 | 42.852 | 42.888 | 42.758 | 43.707 |
| 120 | 37.840 | 37.881 | 37.309 | 37.332 | 37.252 | 37.371 | 36.601 | 36.629 | 36.542 | 37.362 |
| 121 | 31.220 | 31.239 | 30.342 | 30.502 | 30.464 | 30.531 | 29.789 | 29.810 | 29.788 | 30.598 |
| 122 | 5.016 | 5.016 | 4.589 | 4.722 | 4.783 | 4.735 | 4.704 | 4.714 | 4.705 | 4.521 |
| 123 | 9.924 | 9.928 | 8.827 | 9.083 | 9.165 | 9.110 | 9.032 | 9.052 | 9.096 | 9.054 |
| 124 | 8.055 | 8.063 | 7.196 | 7.325 | 7.438 | 7.356 | 7.336 | 7.360 | 7.375 | 7.301 |
| 125 | 11.275 | 11.294 | 10.058 | 10.300 | 10.447 | 10.357 | 10.210 | 10.254 | 10.276 | 10.162 |
| 126 | 22.514 | 22.555 | 23.337 | 23.235 | 23.115 | 23.266 | 22.510 | 22.534 | 22.427 | 23.238 |
| 127 | 6.288 | 6.288 | 5.755 | 6.065 | 6.090 | 6.073 | 5.625 | 5.631 | 5.693 | 6.189 |
| 128 | 24.536 | 24.563 | 22.642 | 24.294 | 24.457 | 24.341 | 22.347 | 22.380 | 22.592 | 25.055 |
| 129 | 3.113 | 3.113 | 3.222 | 3.144 | 3.135 | 3.147 | 3.071 | 3.073 | 3.067 | 3.205 |
| 130 | 16.130 | 16.153 | 16.068 | 16.378 | 16.374 | 16.395 | 15.603 | 15.615 | 15.637 | 16.598 |
| 131 | 13.577 | 13.590 | 14.092 | 14.027 | 13.964 | 14.038 | 13.611 | 13.618 | 13.570 | 14.091 |
| 132 | 8.463 | 8.463 | 7.786 | 8.055 | 8.088 | 8.064 | 7.828 | 7.834 | 7.867 | 8.371 |
| 133 | 6.137 | 6.137 | 5.484 | 5.706 | 5.747 | 5.716 | 5.667 | 5.675 | 5.684 | 5.484 |
| 134 | 12.178 | 12.181 | 10.859 | 11.246 | 11.313 | 11.269 | 11.116 | 11.132 | 11.216 | 11.302 |
| 135 | 16.204 | 16.214 | 14.351 | 15.036 | 15.176 | 15.074 | 14.683 | 14.711 | 14.806 | 15.045 |
| 136 | 7.535 | 7.539 | 7.287 | 7.285 | 7.299 | 7.302 | 7.349 | 7.362 | 7.308 | 7.161 |
| 137 | 14.332 | 14.336 | 13.632 | 13.766 | 13.768 | 13.780 | 13.541 | 13.551 | 13.584 | 13.984 |
| 138 | 14.783 | 14.789 | 13.278 | 13.280 | 13.440 | 13.305 | 13.538 | 13.555 | 13.586 | 13.558 |
| 139 | 11.608 | 11.616 | 9.992 | 10.207 | 10.394 | 10.233 | 10.395 | 10.412 | 10.399 | 10.117 |
| 140 | 13.589 | 13.591 | 13.130 | 12.511 | 12.543 | 12.525 | 13.110 | 13.120 | 13.012 | 12.859 |

Table ST23: Lattice constants in the SOL62 data set. Functionals with '-v' employ the rVV10 methodology. The units are Å, and the reference values are provided in the last column. The errors per functional are shown in Figs. SF3 (PBE, PBE-D3), SF6 (MS2, MCML), SF9 (SCAN, $r^2$SCAN), and SF12 (all functional using rVV10).

| System | PBE | PBE-D3 | MS2 | SCAN | $r^2$SCAN | SCAN-v | MCML | MCML-v | VCML-v | REF |
|---|---|---|---|---|---|---|---|---|---|---|
| Ag | 4.147 | 4.073 | 4.066 | 4.085 | 4.107 | 4.069 | 4.086 | 4.073 | 4.087 | 4.063 |
| AlAs | 5.733 | 5.699 | 5.679 | 5.672 | 5.677 | 5.664 | 5.683 | 5.676 | 5.688 | 5.647 |
| AlP | 5.506 | 5.476 | 5.467 | 5.466 | 5.473 | 5.460 | 5.473 | 5.468 | 5.476 | 5.448 |
| AlSb | 6.232 | 6.196 | 6.175 | 6.172 | 6.184 | 6.162 | 6.179 | 6.170 | 6.182 | 6.121 |
| Al | 4.038 | 4.005 | 4.012 | 4.003 | 3.986 | 4.000 | 4.008 | 4.006 | 4.015 | 4.019 |
| Au | 4.157 | 4.099 | 4.074 | 4.090 | 4.128 | 4.079 | 4.089 | 4.080 | 4.088 | 4.061 |
| BAs | 4.817 | 4.790 | 4.777 | 4.779 | 4.787 | 4.774 | 4.776 | 4.772 | 4.781 | 4.765 |
| BN | 3.626 | 3.616 | 3.606 | 3.608 | 3.614 | 3.606 | 3.607 | 3.606 | 3.613 | 3.593 |
| BP | 4.546 | 4.524 | 4.521 | 4.523 | 4.532 | 4.519 | 4.522 | 4.519 | 4.525 | 4.525 |
| Ba | 5.033 | 4.977 | 5.036 | 5.049 | 5.077 | 5.016 | 5.005 | 4.978 | 5.044 | 5.003 |
| C | 3.572 | 3.564 | 3.553 | 3.555 | 3.562 | 3.553 | 3.554 | 3.553 | 3.560 | 3.553 |
| Ca | 5.527 | 5.493 | 5.500 | 5.548 | 5.576 | 5.534 | 5.541 | 5.530 | 5.519 | 5.554 |
| CdS | 5.938 | 5.867 | 5.884 | 5.871 | 5.888 | 5.854 | 5.894 | 5.879 | 5.889 | 5.808 |
| CdSe | 6.207 | 6.122 | 6.128 | 6.126 | 6.143 | 6.107 | 6.129 | 6.113 | 6.138 | 6.044 |
| CdTe | 6.625 | 6.533 | 6.517 | 6.535 | 6.563 | 6.512 | 6.527 | 6.503 | 6.532 | 6.473 |
| Cu | 3.635 | 3.567 | 3.553 | 3.570 | 3.582 | 3.561 | 3.579 | 3.572 | 3.585 | 3.596 |
| Fe | 2.830 | 2.804 | 2.789 | 2.837 | 2.864 | 2.828 | 2.797 | 2.793 | 2.802 | 2.858 |
| GaAs | 5.762 | 5.722 | 5.680 | 5.665 | 5.672 | 5.656 | 5.686 | 5.677 | 5.694 | 5.635 |
| GaN | 4.589 | 4.565 | 4.548 | 4.527 | 4.527 | 4.524 | 4.550 | 4.547 | 4.557 | 4.509 |
| GaP | 5.534 | 5.501 | 5.482 | 5.463 | 5.467 | 5.455 | 5.483 | 5.478 | 5.488 | 5.434 |
| GaSb | 6.223 | 6.178 | 6.118 | 6.118 | 6.136 | 6.105 | 6.130 | 6.119 | 6.137 | 6.076 |
| Ge | 5.782 | 5.758 | 5.689 | 5.684 | 5.681 | 5.676 | 5.698 | 5.691 | 5.707 | 5.646 |
| HfC | 4.647 | 4.621 | 4.613 | 4.613 | 4.630 | 4.610 | 4.616 | 4.614 | 4.621 | 4.629 |
| HfN | 4.533 | 4.504 | 4.495 | 4.494 | 4.509 | 4.490 | 4.502 | 4.500 | 4.504 | 4.510 |
| InAs | 6.211 | 6.163 | 6.121 | 6.122 | 6.131 | 6.109 | 6.129 | 6.119 | 6.135 | 6.030 |
| InP | 6.001 | 5.963 | 5.945 | 5.937 | 5.947 | 5.926 | 5.949 | 5.940 | 5.949 | 5.852 |
| InSb | 6.647 | 6.590 | 6.531 | 6.546 | 6.569 | 6.528 | 6.545 | 6.531 | 6.550 | 6.461 |
| Ir | 3.873 | 3.838 | 3.822 | 3.788 | 3.853 | 3.784 | 3.828 | 3.825 | 3.830 | 3.833 |
| K | 5.286 | 5.228 | 5.317 | 5.307 | 5.351 | 5.277 | 5.279 | 5.256 | 5.292 | 5.208 |
| LiCl | 5.153 | 5.087 | 5.080 | 5.094 | 5.111 | 5.073 | 5.112 | 5.094 | 5.112 | 5.072 |
| LiF | 4.071 | 4.006 | 3.989 | 3.977 | 3.994 | 3.967 | 3.999 | 3.991 | 4.011 | 3.973 |
| Li | 3.440 | 3.374 | 3.428 | 3.470 | 3.480 | 3.467 | 3.408 | 3.412 | 3.424 | 3.451 |
| MgO | 4.247 | 4.209 | 4.197 | 4.186 | 4.196 | 4.181 | 4.208 | 4.203 | 4.215 | 4.189 |
| MgS | 5.223 | 5.190 | 5.180 | 5.185 | 5.193 | 5.176 | 5.184 | 5.178 | 5.189 | 5.188 |
| Mo | 3.151 | 3.123 | 3.129 | 3.136 | 3.144 | 3.133 | 3.134 | 3.131 | 3.133 | 3.141 |
| NaCl | 5.655 | 5.609 | 5.547 | 5.519 | 5.545 | 5.494 | 5.530 | 5.511 | 5.545 | 5.572 |
| NaF | 4.632 | 4.562 | 4.525 | 4.479 | 4.503 | 4.465 | 4.518 | 4.507 | 4.532 | 4.582 |
| Na | 4.193 | 4.161 | 4.171 | 4.180 | 4.199 | 4.171 | 4.115 | 4.143 | 4.132 | 4.209 |
| NbC | 4.507 | 4.482 | 4.494 | 4.501 | 4.508 | 4.497 | 4.496 | 4.493 | 4.496 | 4.461 |
| NbN | 4.454 | 4.424 | 4.439 | 4.442 | 4.450 | 4.437 | 4.442 | 4.438 | 4.439 | 4.371 |
| Nb | 3.322 | 3.281 | 3.305 | 3.311 | 3.320 | 3.306 | 3.309 | 3.305 | 3.312 | 3.293 |
| Ni | 3.518 | 3.476 | 3.460 | 3.465 | 3.479 | 3.457 | 3.471 | 3.462 | 3.477 | 3.507 |
| Pd | 3.940 | 3.885 | 3.879 | 3.893 | 3.912 | 3.884 | 3.894 | 3.886 | 3.889 | 3.876 |
| Pt | 3.967 | 3.918 | 3.905 | 3.897 | 3.943 | 3.891 | 3.916 | 3.912 | 3.915 | 3.913 |
| Rb | 5.671 | 5.617 | 5.698 | 5.709 | 5.752 | 5.678 | 5.701 | 5.660 | 5.661 | 5.577 |
| Rh | 3.824 | 3.786 | 3.776 | 3.778 | 3.804 | 3.772 | 3.784 | 3.779 | 3.784 | 3.794 |
| SiC | 4.379 | 4.366 | 4.352 | 4.351 | 4.355 | 4.349 | 4.353 | 4.351 | 4.356 | 4.347 |
| Si | 5.469 | 5.453 | 5.429 | 5.427 | 5.440 | 5.422 | 5.435 | 5.430 | 5.438 | 5.421 |
| Sn | 6.654 | 6.613 | 6.531 | 6.558 | 6.565 | 6.538 | 6.548 | 6.532 | 6.549 | 6.474 |
| Sr | 6.024 | 5.984 | 6.038 | 6.081 | 6.099 | 6.057 | 6.053 | 6.045 | 6.079 | 6.040 |
| Ta | 3.308 | 3.272 | 3.268 | 3.270 | 3.290 | 3.267 | 3.276 | 3.273 | 3.278 | 3.299 |
| TiC | 4.337 | 4.309 | 4.319 | 4.326 | 4.334 | 4.322 | 4.322 | 4.319 | 4.325 | 4.318 |
| TiN | 4.256 | 4.224 | 4.232 | 4.240 | 4.246 | 4.237 | 4.237 | 4.235 | 4.239 | 4.228 |
| VC | 4.155 | 4.130 | 4.130 | 4.137 | 4.149 | 4.133 | 4.134 | 4.130 | 4.136 | 4.149 |
| VN | 4.120 | 4.091 | 4.093 | 4.101 | 4.110 | 4.097 | 4.097 | 4.094 | 4.098 | 4.122 |
| V | 2.978 | 2.938 | 2.950 | 2.953 | 2.965 | 2.949 | 2.955 | 2.952 | 2.957 | 3.023 |
| W | 3.172 | 3.147 | 3.139 | 3.139 | 3.156 | 3.137 | 3.145 | 3.143 | 3.146 | 3.160 |
| ZnS | 5.448 | 5.385 | 5.382 | 5.374 | 5.389 | 5.361 | 5.378 | 5.369 | 5.384 | 5.392 |
| ZnSe | 5.740 | 5.664 | 5.648 | 5.649 | 5.667 | 5.634 | 5.646 | 5.636 | 5.652 | 5.661 |
| ZnTe | 6.183 | 6.108 | 6.065 | 6.083 | 6.114 | 6.065 | 6.059 | 6.045 | 6.071 | 6.090 |
| ZrC | 4.711 | 4.681 | 4.698 | 4.706 | 4.713 | 4.702 | 4.700 | 4.696 | 4.701 | 4.687 |
| ZrN | 4.597 | 4.564 | 4.577 | 4.583 | 4.588 | 4.578 | 4.582 | 4.577 | 4.582 | 4.575 |

Table ST24: Cohesive energies in the SOL62 data set. Functionals with '-v' employ the rVV10 methodology. The units are eV, and the reference values are provided in the last column. The errors per functional are shown in Figs. SF3 (PBE, PBE-D3), SF6 (MS2, MCML), SF9 (SCAN, r$^2$SCAN), and SF12 (all functional using rVV10).

| System | PBE | PBE-D3 | MS2 | SCAN | r$^2$SCAN | SCAN-v | MCML | MCML-v | VCML-v | REF |
|---|---|---|---|---|---|---|---|---|---|---|
| Ag | −2.520 | −3.010 | −3.110 | −2.886 | −2.881 | −3.083 | −3.237 | −3.402 | −3.297 | −2.970 |
| AlAs | −3.688 | −3.882 | −3.860 | −3.896 | −3.863 | −3.997 | −3.831 | −3.915 | −3.844 | −3.820 |
| AlP | −4.089 | −4.263 | −4.223 | −4.266 | −4.245 | −4.363 | −4.122 | −4.202 | −4.143 | −4.310 |
| AlSb | −3.236 | −3.432 | −3.417 | −3.422 | −3.332 | −3.533 | −3.427 | −3.519 | −3.451 | −3.340 |
| Al | −3.431 | −3.596 | −3.429 | −3.601 | −3.602 | −3.706 | −3.354 | −3.441 | −3.438 | −3.420 |
| Au | −3.037 | −3.693 | −3.814 | −3.557 | −3.420 | −3.788 | −3.951 | −4.144 | −4.006 | −3.830 |
| BAs | −4.625 | −4.813 | −4.724 | −4.708 | −4.626 | −4.814 | −4.757 | −4.846 | −4.767 | −4.780 |
| BN | −6.935 | −7.073 | −6.854 | −6.837 | −6.787 | −6.924 | −6.860 | −6.933 | −6.853 | −6.760 |
| BP | −5.291 | −5.466 | −5.336 | −5.330 | −5.280 | −5.431 | −5.282 | −5.366 | −5.297 | −5.140 |
| Ba | −1.877 | −1.994 | −2.095 | −2.009 | −1.989 | −2.134 | −1.974 | −2.089 | −2.051 | −1.910 |
| C | −7.714 | −7.822 | −7.506 | −7.507 | −7.467 | −7.600 | −7.397 | −7.474 | −7.458 | −7.550 |
| Ca | −1.913 | −2.065 | −1.882 | −1.984 | −1.987 | −2.077 | −1.717 | −1.798 | −1.808 | −1.860 |
| CdS | −2.530 | −2.778 | −2.712 | −2.723 | −2.764 | −2.836 | −2.716 | −2.810 | −2.765 | −2.820 |
| CdSe | −2.300 | −2.555 | −2.513 | −2.497 | −2.545 | −2.613 | −2.523 | −2.621 | −2.554 | −2.480 |
| CdTe | −2.037 | −2.291 | −2.300 | −2.218 | −2.227 | −2.344 | −2.312 | −2.419 | −2.347 | −2.250 |
| Cu | −3.486 | −3.995 | −4.119 | −3.888 | −3.860 | −4.043 | −4.229 | −4.359 | −4.260 | −3.520 |
| Fe | −4.879 | −5.192 | −4.745 | −4.586 | −4.648 | −4.758 | −4.737 | −4.881 | −4.920 | −4.320 |
| GaAs | −3.156 | −3.370 | −3.387 | −3.369 | −3.323 | −3.479 | −3.391 | −3.482 | −3.391 | −3.340 |
| GaN | −4.381 | −4.546 | −4.479 | −4.463 | −4.461 | −4.560 | −4.450 | −4.530 | −4.458 | −4.560 |
| GaP | −3.472 | −3.665 | −3.642 | −3.658 | −3.637 | −3.764 | −3.581 | −3.668 | −3.602 | −3.610 |
| GaSb | −2.837 | −3.055 | −3.101 | −3.059 | −2.938 | −3.178 | −3.138 | −3.238 | −3.143 | −3.030 |
| Ge | −3.719 | −3.883 | −3.925 | −3.978 | −3.886 | −4.086 | −3.910 | −3.999 | −3.912 | −3.910 |
| HfC | −8.128 | −8.406 | −8.258 | −8.124 | −8.160 | −8.270 | −8.161 | −8.283 | −8.234 | −8.180 |
| HfN | −7.632 | −7.949 | −7.856 | −7.570 | −7.596 | −7.720 | −7.777 | −7.902 | −7.816 | −8.080 |
| InAs | −2.886 | −3.093 | −3.135 | −3.031 | −3.020 | −3.148 | −3.160 | −3.258 | −3.166 | −3.080 |
| InP | −3.116 | −3.302 | −3.302 | −3.233 | −3.239 | −3.346 | −3.265 | −3.359 | −3.295 | −3.460 |
| InSb | −2.641 | −2.859 | −2.930 | −2.806 | −2.722 | −2.931 | −2.989 | −3.093 | −2.997 | −2.810 |
| Ir | −7.314 | −8.022 | −8.123 | −7.563 | −7.107 | −7.833 | −8.048 | −8.268 | −8.138 | −6.970 |
| K | −0.869 | −0.997 | −0.884 | −0.858 | −0.850 | −0.911 | −0.890 | −0.935 | −0.943 | −0.930 |
| LiCl | −3.355 | −3.521 | −3.320 | −3.486 | −3.469 | −3.544 | −3.288 | −3.336 | −3.327 | −3.580 |
| LiF | −4.324 | −4.464 | −4.128 | −4.394 | −4.397 | −4.435 | −4.115 | −4.148 | −4.166 | −4.460 |
| Li | −1.606 | −1.708 | −1.548 | −1.566 | −1.575 | −1.597 | −1.459 | −1.485 | −1.502 | −1.670 |
| MgO | −5.006 | −5.212 | −4.966 | −5.261 | −5.257 | −5.337 | −4.978 | −5.041 | −4.984 | −5.190 |
| MgS | −3.715 | −3.945 | −3.811 | −3.985 | −3.979 | −4.079 | −3.739 | −3.817 | −3.779 | −4.040 |
| Mo | −6.365 | −6.904 | −6.677 | −5.929 | −5.701 | −6.164 | −6.662 | −6.858 | −6.772 | −6.860 |
| NaCl | −3.112 | −3.316 | −3.118 | −3.296 | −3.284 | −3.357 | −3.148 | −3.198 | −3.189 | −3.350 |
| NaF | −3.884 | −4.048 | −3.721 | −4.011 | −4.016 | −4.056 | −3.778 | −3.816 | −3.828 | −3.970 |
| Na | −1.088 | −1.247 | −1.090 | −1.103 | −1.090 | −1.143 | −1.113 | −1.146 | −1.154 | −1.130 |
| NbC | −7.856 | −8.172 | −7.745 | −7.596 | −7.516 | −7.760 | −7.740 | −7.877 | −7.859 | −8.330 |
| NbN | −6.944 | −7.290 | −6.913 | −6.603 | −6.520 | −6.769 | −6.910 | −7.048 | −7.003 | −7.530 |
| Nb | −6.942 | −7.492 | −7.054 | −6.583 | −6.363 | −6.806 | −7.136 | −7.321 | −7.265 | −7.600 |
| Ni | −4.732 | −5.135 | −4.652 | −4.421 | −4.642 | −4.581 | −4.713 | −4.851 | −4.866 | −4.480 |
| Pd | −3.741 | −4.318 | −4.460 | −4.367 | −4.165 | −4.592 | −4.614 | −4.802 | −4.670 | −3.910 |
| Pt | −5.489 | −6.254 | −6.399 | −5.926 | −5.714 | −6.180 | −6.495 | −6.705 | −6.557 | −5.870 |
| Rb | −0.775 | −0.903 | −0.797 | −0.768 | −0.744 | −0.826 | −0.826 | −0.881 | −0.891 | −0.850 |
| Rh | −5.754 | −6.331 | −5.731 | −5.425 | −5.493 | −5.662 | −5.894 | −6.091 | −6.037 | −5.780 |
| SiC | −6.406 | −6.550 | −6.354 | −6.449 | −6.430 | −6.550 | −6.242 | −6.326 | −6.311 | −6.470 |
| Si | −4.556 | −4.702 | −4.652 | −4.712 | −4.671 | −4.817 | −4.484 | −4.571 | −4.545 | −4.700 |
| Sn | −3.190 | −3.369 | −3.474 | −3.423 | −3.287 | −3.559 | −3.507 | −3.622 | −3.536 | −3.160 |
| Sr | −1.609 | −1.759 | −1.825 | −1.806 | −1.790 | −1.910 | −1.721 | −1.817 | −1.791 | −1.730 |
| Ta | −8.199 | −8.797 | −9.049 | −8.472 | −8.051 | −8.698 | −8.973 | −9.160 | −9.014 | −8.110 |
| TiC | −7.314 | −7.617 | −7.040 | −7.022 | −7.034 | −7.151 | −6.946 | −7.052 | −7.102 | −7.240 |
| TiN | −6.906 | −7.247 | −6.706 | −6.567 | −6.575 | −6.698 | −6.633 | −6.740 | −6.758 | −6.760 |
| VC | −6.985 | −7.304 | −6.739 | −6.614 | −6.597 | −6.755 | −6.688 | −6.805 | −6.816 | −7.000 |
| VN | −6.235 | −6.586 | −6.087 | −5.801 | −5.803 | −5.943 | −6.053 | −6.171 | −6.145 | −6.300 |
| V | −5.350 | −5.915 | −5.149 | −4.725 | −4.652 | −4.902 | −5.126 | −5.272 | −5.278 | −5.340 |
| W | −8.486 | −9.110 | −9.469 | −9.009 | −8.067 | −9.252 | −9.699 | −9.900 | −9.734 | −8.930 |
| ZnS | −2.884 | −3.150 | −3.084 | −3.151 | −3.156 | −3.259 | −3.081 | −3.171 | −3.136 | −3.210 |
| ZnSe | −2.568 | −2.841 | −2.799 | −2.829 | −2.843 | −2.940 | −2.802 | −2.895 | −2.839 | −2.660 |
| ZnTe | −2.227 | −2.493 | −2.506 | −2.458 | −2.435 | −2.580 | −2.520 | −2.623 | −2.558 | −2.430 |
| ZrC | −7.885 | −8.169 | −7.719 | −7.757 | −7.726 | −7.907 | −7.615 | −7.739 | −7.744 | −7.990 |
| ZrN | −7.471 | −7.792 | −7.393 | −7.291 | −7.251 | −7.445 | −7.312 | −7.440 | −7.405 | −7.580 |

Table ST25: Bulk moduli in the SOL62 data set. Functionals with ’-v’ employ the rVV10 methodology. The units are GPa, and the reference values are provided in the last column. The errors per functional are shown in Figs. SF3 (PBE, PBE-D3), SF6 (MS2, MCML), SF9 (SCAN, $r^2$SCAN), and SF12 (all functional using rVV10).

| System | PBE | PBE-D3 | MS2 | SCAN | $r^2$SCAN | SCAN-v | MCML | MCML-v | VCML-v | REF |
|---|---|---|---|---|---|---|---|---|---|---|
| Ag | 91.391 | 105.869 | 116.619 | 110.596 | 104.534 | 116.166 | 105.185 | 109.810 | 109.449 | 112.600 |
| AlAs | 67.177 | 70.430 | 77.252 | 76.553 | 76.347 | 77.539 | 75.650 | 76.445 | 75.614 | 79.300 |
| AlP | 82.612 | 85.474 | 92.642 | 91.446 | 91.060 | 92.384 | 91.178 | 91.969 | 90.267 | 87.000 |
| AlSb | 49.361 | 52.624 | 57.432 | 56.250 | 55.793 | 57.235 | 56.973 | 57.787 | 56.449 | 59.500 |
| Al | 76.856 | 82.408 | 80.947 | 78.967 | 93.641 | 79.363 | 81.799 | 82.393 | 81.365 | 81.000 |
| Au | 139.712 | 151.390 | 178.572 | 167.064 | 154.506 | 173.792 | 167.615 | 173.044 | 171.420 | 182.900 |
| BAs | 131.820 | 134.657 | 147.584 | 145.770 | 142.114 | 147.227 | 146.934 | 148.165 | 145.498 | 151.000 |
| BN | 372.428 | 378.565 | 397.099 | 394.097 | 390.073 | 395.931 | 395.665 | 397.249 | 390.560 | 388.500 |
| BP | 161.871 | 166.100 | 176.499 | 173.271 | 170.107 | 174.609 | 174.728 | 175.853 | 172.783 | 176.500 |
| Ba | 8.827 | 8.376 | 8.470 | 8.460 | 8.453 | 8.690 | 8.009 | 8.255 | 8.630 | 9.300 |
| C | 433.574 | 436.532 | 465.614 | 458.125 | 449.924 | 460.176 | 462.345 | 464.062 | 456.874 | 453.300 |
| Ca | 17.192 | 15.950 | 17.936 | 17.396 | 17.510 | 17.682 | 17.749 | 18.291 | 18.847 | 18.700 |
| CdS | 53.348 | 59.791 | 59.840 | 61.397 | 60.471 | 63.077 | 60.143 | 61.482 | 58.860 | 65.000 |
| CdSe | 44.772 | 49.996 | 50.844 | 52.223 | 51.607 | 53.794 | 51.317 | 52.615 | 50.359 | 55.500 |
| CdTe | 35.119 | 39.478 | 40.221 | 40.537 | 40.321 | 41.963 | 40.200 | 41.082 | 39.876 | 46.200 |
| Cu | 137.967 | 161.561 | 169.959 | 163.205 | 159.846 | 167.423 | 186.661 | 190.000 | 185.811 | 144.900 |
| Fe | 188.751 | 207.627 | 228.216 | 159.650 | 176.391 | 163.245 | 230.884 | 243.138 | 190.267 | 177.900 |
| GaAs | 61.998 | 66.103 | 73.668 | 74.731 | 73.811 | 76.166 | 72.801 | 73.951 | 72.316 | 78.100 |
| GaN | 182.206 | 189.871 | 201.559 | 212.125 | 211.334 | 214.124 | 201.976 | 203.595 | 197.362 | 204.000 |
| GaP | 78.570 | 82.081 | 90.373 | 91.607 | 90.461 | 93.006 | 89.550 | 90.698 | 88.768 | 89.800 |
| GaSb | 45.357 | 49.420 | 54.296 | 54.105 | 53.736 | 55.451 | 53.701 | 54.787 | 53.122 | 56.800 |
| Ge | 59.021 | 58.880 | 72.522 | 71.747 | 73.117 | 73.033 | 72.110 | 73.160 | 70.672 | 77.900 |
| HfC | 253.080 | 263.613 | 271.400 | 271.701 | 266.588 | 273.668 | 270.863 | 272.458 | 268.793 | 277.900 |
| HfN | 285.467 | 299.535 | 310.640 | 313.228 | 306.259 | 315.956 | 308.561 | 310.764 | 304.941 | 312.300 |
| InAs | 49.498 | 52.883 | 58.574 | 58.839 | 58.933 | 60.232 | 58.175 | 59.299 | 57.579 | 58.400 |
| InP | 60.816 | 63.421 | 70.435 | 70.620 | 70.220 | 72.027 | 69.992 | 71.148 | 69.559 | 73.500 |
| InSb | 37.082 | 41.191 | 44.456 | 43.648 | 44.014 | 44.894 | 43.810 | 44.864 | 43.542 | 47.200 |
| Ir | 349.849 | 379.172 | 400.895 | 406.603 | 378.839 | 413.174 | 384.425 | 389.110 | 392.695 | 385.700 |
| K | 3.591 | 4.351 | 3.497 | 3.378 | 3.435 | 3.513 | 4.003 | 4.056 | 3.343 | 3.730 |
| LiCl | 31.911 | 34.469 | 36.525 | 36.073 | 35.096 | 37.428 | 35.051 | 36.131 | 35.218 | 37.300 |
| LiF | 67.450 | 73.612 | 78.132 | 80.487 | 78.720 | 82.505 | 75.951 | 81.360 | 77.081 | 75.400 |
| Li | 13.945 | 13.681 | 14.087 | 13.204 | 13.117 | 13.264 | 18.936 | 16.261 | 14.277 | 13.400 |
| MgO | 151.732 | 160.681 | 167.431 | 172.192 | 170.825 | 174.071 | 169.344 | 170.782 | 163.942 | 173.000 |
| MgS | 74.688 | 79.364 | 82.278 | 81.730 | 80.913 | 82.885 | 83.346 | 84.721 | 81.356 | 81.000 |
| Mo | 269.034 | 286.685 | 288.234 | 286.761 | 283.653 | 289.963 | 279.924 | 282.562 | 284.979 | 267.900 |
| NaCl | 24.396 | 24.703 | 28.751 | 30.379 | 29.214 | 31.794 | 31.409 | 32.463 | 31.018 | 29.200 |
| NaF | 47.293 | 49.355 | 56.147 | 63.001 | 60.133 | 64.944 | 62.768 | 64.239 | 59.593 | 54.100 |
| Na | 7.889 | 8.238 | 8.066 | 8.029 | 7.946 | 8.136 | 10.434 | 11.211 | 8.884 | 7.700 |
| NbC | 298.578 | 311.675 | 313.039 | 313.605 | 309.030 | 316.271 | 320.063 | 322.388 | 315.704 | 312.300 |
| NbN | 304.327 | 322.194 | 322.663 | 324.504 | 318.507 | 328.380 | 318.923 | 322.008 | 322.827 | 300.500 |
| Nb | 172.549 | 185.986 | 183.403 | 180.617 | 176.422 | 182.774 | 190.455 | 192.249 | 187.379 | 176.200 |
| Ni | 194.641 | 212.467 | 223.711 | 217.701 | 217.320 | 221.785 | 194.451 | 228.642 | 191.749 | 190.700 |
| Pd | 169.639 | 195.449 | 203.557 | 196.243 | 186.808 | 202.854 | 192.373 | 197.225 | 197.332 | 197.400 |
| Pt | 250.001 | 282.632 | 299.186 | 294.822 | 273.241 | 301.272 | 291.420 | 296.600 | 290.504 | 279.200 |
| Rb | 2.793 | 3.349 | 2.670 | 2.850 | 2.626 | 2.838 | 2.959 | 3.165 | 3.184 | 3.110 |
| Rh | 258.287 | 283.772 | 296.246 | 294.811 | 281.497 | 301.123 | 289.849 | 294.909 | 289.680 | 271.600 |
| SiC | 212.390 | 217.556 | 229.551 | 226.133 | 227.046 | 227.477 | 225.770 | 226.880 | 226.635 | 228.900 |
| Si | 88.706 | 87.626 | 101.780 | 99.678 | 97.217 | 100.725 | 97.933 | 98.816 | 98.092 | 100.300 |
| Sn | 36.146 | 38.093 | 44.169 | 41.715 | 43.487 | 43.112 | 42.989 | 44.038 | 43.067 | 53.500 |
| Sr | 11.574 | 10.631 | 12.118 | 11.414 | 11.544 | 11.569 | 11.335 | 12.366 | 12.338 | 12.500 |
| Ta | 201.057 | 216.799 | 216.740 | 216.074 | 209.533 | 218.142 | 216.453 | 218.056 | 213.389 | 195.000 |
| TiC | 265.011 | 279.094 | 281.820 | 280.048 | 277.385 | 282.623 | 280.633 | 282.642 | 278.965 | 249.500 |
| TiN | 293.659 | 314.438 | 317.545 | 314.445 | 312.385 | 317.571 | 316.050 | 316.984 | 311.031 | 295.500 |
| VC | 317.067 | 330.986 | 339.600 | 336.828 | 330.791 | 340.279 | 336.269 | 336.664 | 337.003 | 307.700 |
| VN | 327.620 | 349.287 | 354.150 | 351.702 | 347.174 | 355.576 | 344.005 | 347.333 | 348.701 | 281.300 |
| V | 187.618 | 206.179 | 204.162 | 202.122 | 199.661 | 204.711 | 202.527 | 204.614 | 201.101 | 158.800 |
| W | 312.192 | 332.676 | 338.636 | 340.417 | 328.777 | 343.069 | 330.322 | 332.551 | 333.850 | 315.800 |
| ZnS | 69.366 | 78.690 | 80.520 | 82.389 | 79.101 | 84.281 | 80.884 | 82.460 | 83.316 | 78.100 |
| ZnSe | 56.650 | 64.255 | 67.340 | 67.585 | 65.619 | 69.186 | 65.679 | 66.184 | 69.860 | 65.900 |
| ZnTe | 43.272 | 48.591 | 52.303 | 50.943 | 49.917 | 52.426 | 57.999 | 60.402 | 54.799 | 53.100 |
| ZrC | 221.673 | 232.181 | 232.227 | 231.656 | 229.781 | 233.737 | 231.251 | 232.966 | 230.354 | 229.900 |
| ZrN | 248.870 | 262.224 | 263.908 | 263.925 | 262.479 | 266.913 | 264.330 | 266.719 | 259.345 | 220.300 |

Table ST26: Systems in the ADS41 data set. Identifiers are provided, which are used in Tab. ST27 and Figs. SF4 (PBE, PBE-D3), SF7 (MS2, MCML), SF10 (SCAN, r$^2$SCAN), and SF13 (all functionals using rVV10). Top: physisorption-dominated; bottom: chemisorption-dominated. [a]Calculated as $\frac{5}{3}D_2O + \frac{1}{3}[O@Pt111] \rightarrow \frac{1}{3}[(D_2O \cdots OD)@Pt111] + \frac{1}{6}H_2$.

| Identifier | System |
|---|---|
| 1 | $C_6H_6 + Ag111 \rightarrow C_6H_6@Ag111$ |
| 2 | $C_6H_6 + Au111 \rightarrow C_6H_6@Au111$ |
| 3 | $C_6H_6 + Cu111 \rightarrow C_6H_6@Cu111$ |
| 4 | $C_6H_6 + Pt111 \rightarrow C_6H_6@Pt111$ |
| 5 | $C_2H_6 + Pt111 \rightarrow C_2H_6@Pt111$ |
| 6 | $C_3H_8 + Pt111 \rightarrow C_3H_8@Pt111$ |
| 7 | $C_4H_{10} + Pt111 \rightarrow C_4H_{10}@Pt111$ |
| 8 | $CH_3I + Pt111 \rightarrow CH_3I@Pt111$ |
| 9 | $CH_4 + Pt111 \rightarrow CH_4@Pt111$ |
| 10 | $C_6H_{10} + Pt111 \rightarrow C_6H_{10}@Pt111$ |
| 11[a] | $D_2O + \frac{1}{3}[O@Pt111] \rightarrow \frac{2}{3}[(D_2O \cdots OD)@Pt111]$ |
| 12 | $D_2O + Pt111 \rightarrow D_2O@Pt111$ |
| 13 | $CH_3OH + Pt111 \rightarrow CH_3OH@Pt111$ |
| 14 | $C_{10}H_8 + Pt111 \rightarrow C_{10}H_8@Pt111$ |
| 15 | $NH_3 + Cu100 \rightarrow NH_3@Cu100$ |
| 1 | $C_2H_4 + Pt111 \rightarrow CCH_3@Pt111 + H@Pt111$ |
| 2 | $CH_2I_2 + Pt111 \rightarrow CH@Pt111 + H@Pt111 + 2\ I@Pt111$ |
| 3 | $CH_3I + Pt111 \rightarrow CH_3@Pt111 + I@Pt111$ |
| 4 | $CO + Co001 \rightarrow CO@Co001$ |
| 5 | $CO + Cu111 \rightarrow CO@Cu111$ |
| 6 | $CO + Ir111 \rightarrow CO@Ir111$ |
| 7 | $CO + Ni111 \rightarrow CO@Ni111$ |
| 8 | $CO + Pd100 \rightarrow CO@Pd100$ |
| 9 | $CO + Pd111 \rightarrow CO@Pd111$ |
| 10 | $CO + Pt111 \rightarrow CO@Pt111$ |
| 11 | $CO + Rh111 \rightarrow CO@Rh111$ |
| 12 | $CO + Ru001 \rightarrow CO@Ru001$ |
| 13 | $H_2 + Ni100 \rightarrow 2\ H@Ni100$ |
| 14 | $H_2 + Ni111 \rightarrow 2\ H@Ni111$ |
| 15 | $H_2 + Pd111 \rightarrow 2\ H@Pd111$ |
| 16 | $H_2 + Pt111 \rightarrow 2\ H@Pt111$ |
| 17 | $H_2 + Rh111 \rightarrow 2\ H@Rh111$ |
| 18 | $I_2 + Pt111 \rightarrow 2\ I@Pt111$ |
| 19 | $NO^\bullet + Ni100 \rightarrow N@Ni100 + O@Ni100$ |
| 20 | $NO^\bullet + Pd100 \rightarrow NO@Pd100$ |
| 21 | $NO^\bullet + Pd111 \rightarrow NO@Pd111$ |
| 22 | $NO^\bullet + Pt111 \rightarrow NO@Pt111$ |
| 23 | $O_2^{\bullet\bullet} + Ni100 \rightarrow 2\ O@Ni100$ |
| 24 | $O_2^{\bullet\bullet} + Ni111 \rightarrow 2\ O@Ni111$ |
| 25 | $O_2^{\bullet\bullet} + Pt111 \rightarrow 2\ O@Pt111$ |
| 26 | $O_2^{\bullet\bullet} + Rh100 \rightarrow 2\ O@Rh100$ |

Table ST27: Adsorption energies in the ADS41 data set. Functionals with '-v' employ the rVV10 methodology. The units are eV. Top: physisorption-dominated; bottom: chemisorption-dominated. The reference values are provided in the last column, while the identifiers are defined in Tab. ST26.

| System | PBE | PBE-D3 | MS2 | SCAN | $r^2$SCAN | SCAN-v | MCML | MCML-v | VCML-v | REF |
|---|---|---|---|---|---|---|---|---|---|---|
| 1 | −0.044 | −0.756 | −0.244 | −0.349 | −0.293 | −0.696 | −0.400 | −0.690 | −0.638 | −0.632 |
| 2 | −0.050 | −0.851 | −0.265 | −0.381 | −0.315 | −0.747 | −0.444 | −0.758 | −0.710 | −0.726 |
| 3 | −0.042 | −1.019 | −0.182 | −0.352 | −0.301 | −0.725 | −0.398 | −0.721 | −0.687 | −0.684 |
| 4 | −0.924 | −2.002 | −1.597 | −1.848 | −1.487 | −2.337 | −1.722 | −2.140 | −2.031 | −1.679 |
| 5 | −0.035 | −0.474 | −0.086 | −0.163 | −0.152 | −0.337 | −0.154 | −0.296 | −0.254 | −0.280 |
| 6 | −0.056 | −0.686 | −0.132 | −0.244 | −0.201 | −0.474 | −0.214 | −0.427 | −0.366 | −0.404 |
| 7 | −0.084 | −0.898 | −0.178 | −0.321 | −0.291 | −0.638 | −0.297 | −0.561 | −0.510 | −0.497 |
| 8 | −0.239 | −0.812 | −0.361 | −0.381 | −0.341 | −0.616 | −0.440 | −0.643 | −0.604 | −0.871 |
| 9 | −0.018 | −0.264 | −0.038 | −0.073 | −0.069 | −0.170 | −0.085 | −0.167 | −0.161 | −0.145 |
| 10 | −0.610 | −1.787 | −0.967 | −1.335 | −1.081 | −1.790 | −1.089 | −1.481 | −1.396 | −1.275 |
| 11 | −0.346 | −0.584 | −0.512 | −0.600 | −0.502 | −0.693 | −0.552 | −0.629 | −0.568 | −0.342 |
| 12 | −0.203 | −0.442 | −0.330 | −0.399 | −0.345 | −0.547 | −0.396 | −0.483 | −0.447 | −0.570 |
| 13 | −0.202 | −0.635 | −0.353 | −0.462 | −0.399 | −0.656 | −0.439 | −0.591 | −0.548 | −0.570 |
| 14 | −1.595 | −3.292 | −2.722 | −3.165 | −2.512 | −3.937 | −2.911 | −3.571 | −3.422 | −2.763 |
| 15 | −0.437 | −0.778 | −0.531 | −0.609 | −0.573 | −0.723 | −0.571 | −0.662 | −0.636 | −0.622 |
| 1 | −0.813 | −1.010 | −0.804 | −1.073 | −0.977 | −1.164 | −0.884 | −0.963 | −0.938 | −0.680 |
| 2 | −0.942 | −1.219 | −1.018 | −1.180 | −1.100 | −1.291 | −1.057 | −1.153 | −1.117 | −1.179 |
| 3 | −0.812 | −1.207 | −0.975 | −1.122 | −1.002 | −1.269 | −1.020 | −1.146 | −1.102 | −1.083 |
| 4 | −1.651 | −1.845 | −1.874 | −1.700 | −1.643 | −1.810 | −1.621 | −1.706 | −1.620 | −1.233 |
| 5 | −0.747 | −0.959 | −0.742 | −0.885 | −0.866 | −0.995 | −0.671 | −0.761 | −0.729 | −0.591 |
| 6 | −1.956 | −2.165 | −1.847 | −2.046 | −2.099 | −2.156 | −1.783 | −1.880 | −1.875 | −1.700 |
| 7 | −1.858 | −2.049 | −1.603 | −1.923 | −1.891 | −2.044 | −1.654 | −1.791 | −1.757 | −1.285 |
| 8 | −1.897 | −2.130 | −1.834 | −2.133 | −2.035 | −2.247 | −1.785 | −1.884 | −1.863 | −1.627 |
| 9 | −1.999 | −2.176 | −1.927 | −2.239 | −2.153 | −2.352 | −1.894 | −1.990 | −1.967 | −1.492 |
| 10 | −1.641 | −1.879 | −1.543 | −1.898 | −1.769 | −2.000 | −1.496 | −1.586 | −1.575 | −1.285 |
| 11 | −1.878 | −2.085 | −1.842 | −2.058 | −1.997 | −2.169 | −1.769 | −1.866 | −1.853 | −1.472 |
| 12 | −1.902 | −2.114 | −1.846 | −1.971 | −1.990 | −2.080 | −1.766 | −1.862 | −1.850 | −1.669 |
| 13 | −0.518 | −0.621 | −0.574 | −0.640 | −0.565 | −0.550 | −0.613 | −0.682 | −0.517 | −0.451 |
| 14 | −0.552 | −0.654 | −0.739 | −0.654 | −0.590 | −0.674 | −0.791 | −0.823 | −0.689 | −0.518 |
| 15 | −0.604 | −0.644 | −0.631 | −0.725 | −0.677 | −0.743 | −0.621 | −0.636 | −0.571 | −0.466 |
| 16 | −0.475 | −0.519 | −0.436 | −0.536 | −0.528 | −0.554 | −0.438 | −0.454 | −0.397 | −0.373 |
| 17 | −0.534 | −0.592 | −0.576 | −0.606 | −0.579 | −0.630 | −0.557 | −0.577 | −0.516 | −0.373 |
| 18 | −1.391 | −1.868 | −1.604 | −1.693 | −1.615 | −1.874 | −1.632 | −1.788 | −1.730 | −1.622 |
| 19 | −2.288 | −2.371 | −2.200 | −2.594 | −2.574 | −2.662 | −2.212 | −2.309 | −2.270 | −1.550 |
| 20 | −2.117 | −2.366 | −2.014 | −2.263 | −2.254 | −2.397 | −1.985 | −2.098 | −2.075 | −1.689 |
| 21 | −2.291 | −2.460 | −2.167 | −2.435 | −2.412 | −2.545 | −2.143 | −2.237 | −2.217 | −1.886 |
| 22 | −1.861 | −2.046 | −1.612 | −1.915 | −1.934 | −2.031 | −1.600 | −1.700 | −1.692 | −1.233 |
| 23 | −2.628 | −2.683 | −2.966 | −3.200 | −3.046 | −3.260 | −2.957 | −3.057 | −2.974 | −2.747 |
| 24 | −2.357 | −2.390 | −2.634 | −2.754 | −2.631 | −2.806 | −2.665 | −2.793 | −2.707 | −2.513 |
| 25 | −1.209 | −1.216 | −1.339 | −1.497 | −1.372 | −1.543 | −1.332 | −1.376 | −1.327 | −1.078 |
| 26 | −2.186 | −2.304 | −2.627 | −2.525 | −2.453 | −2.600 | −2.552 | −2.615 | −2.555 | −1.840 |

### 6.3 All errors for all functionals

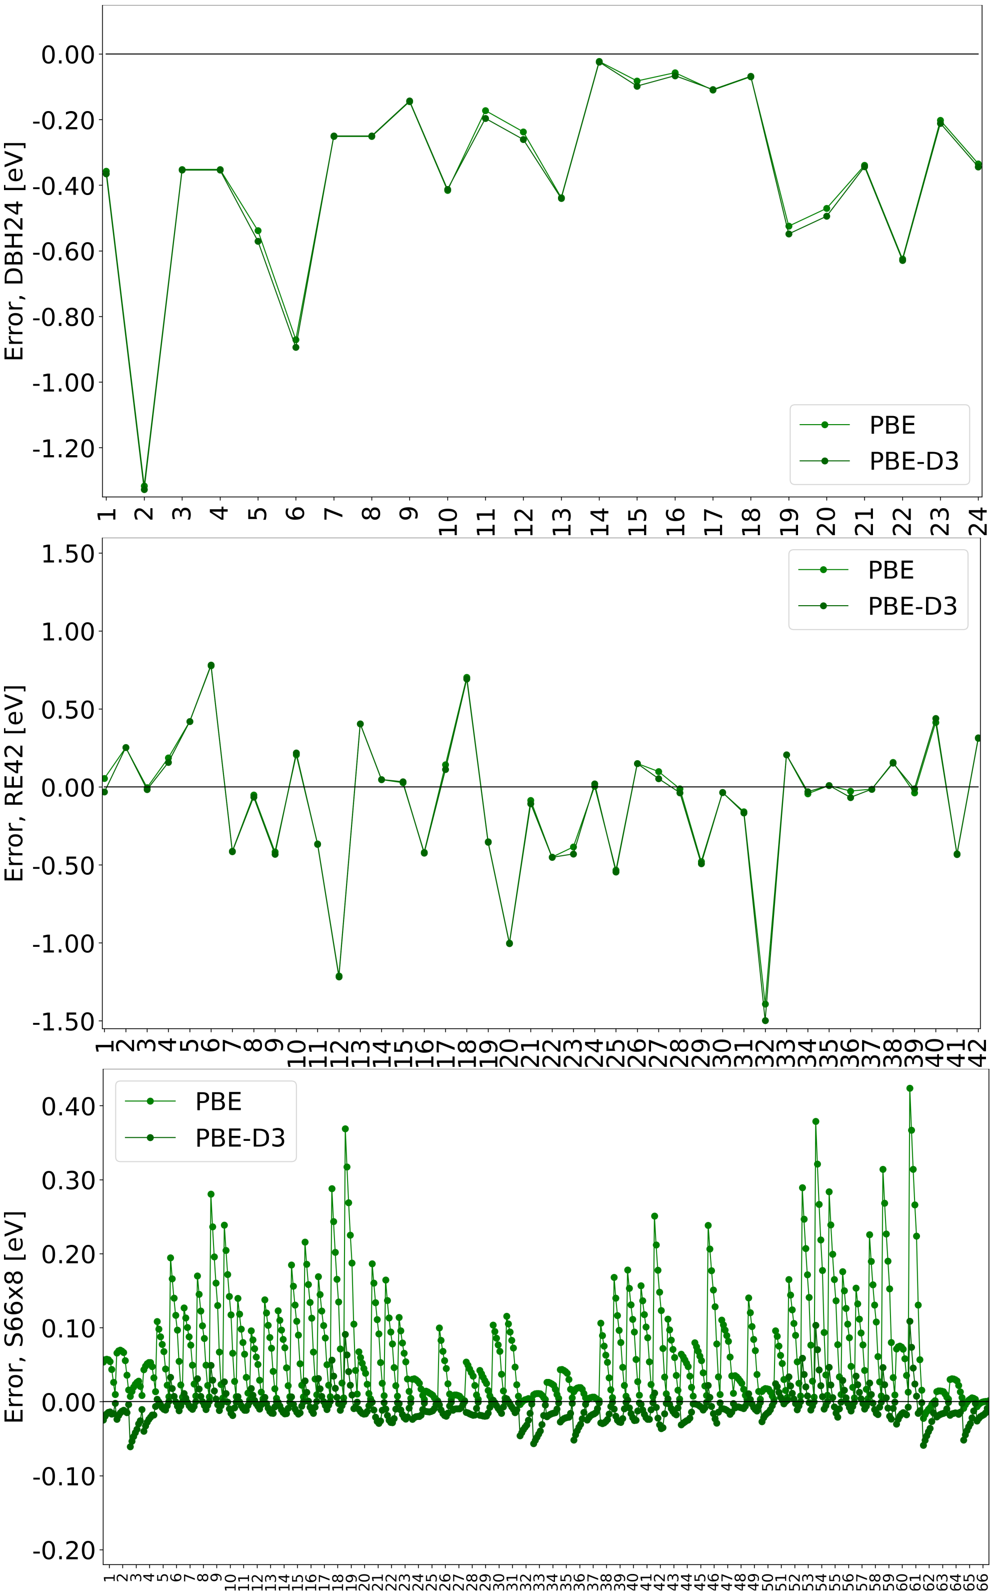


Figure SF2: Errors for all data sets using PBE and PBE-D3. The x-axes denote the identifiers, see Tabs. ST6 (DBH24), ST8 (RE42), and ST10 (S66x8).

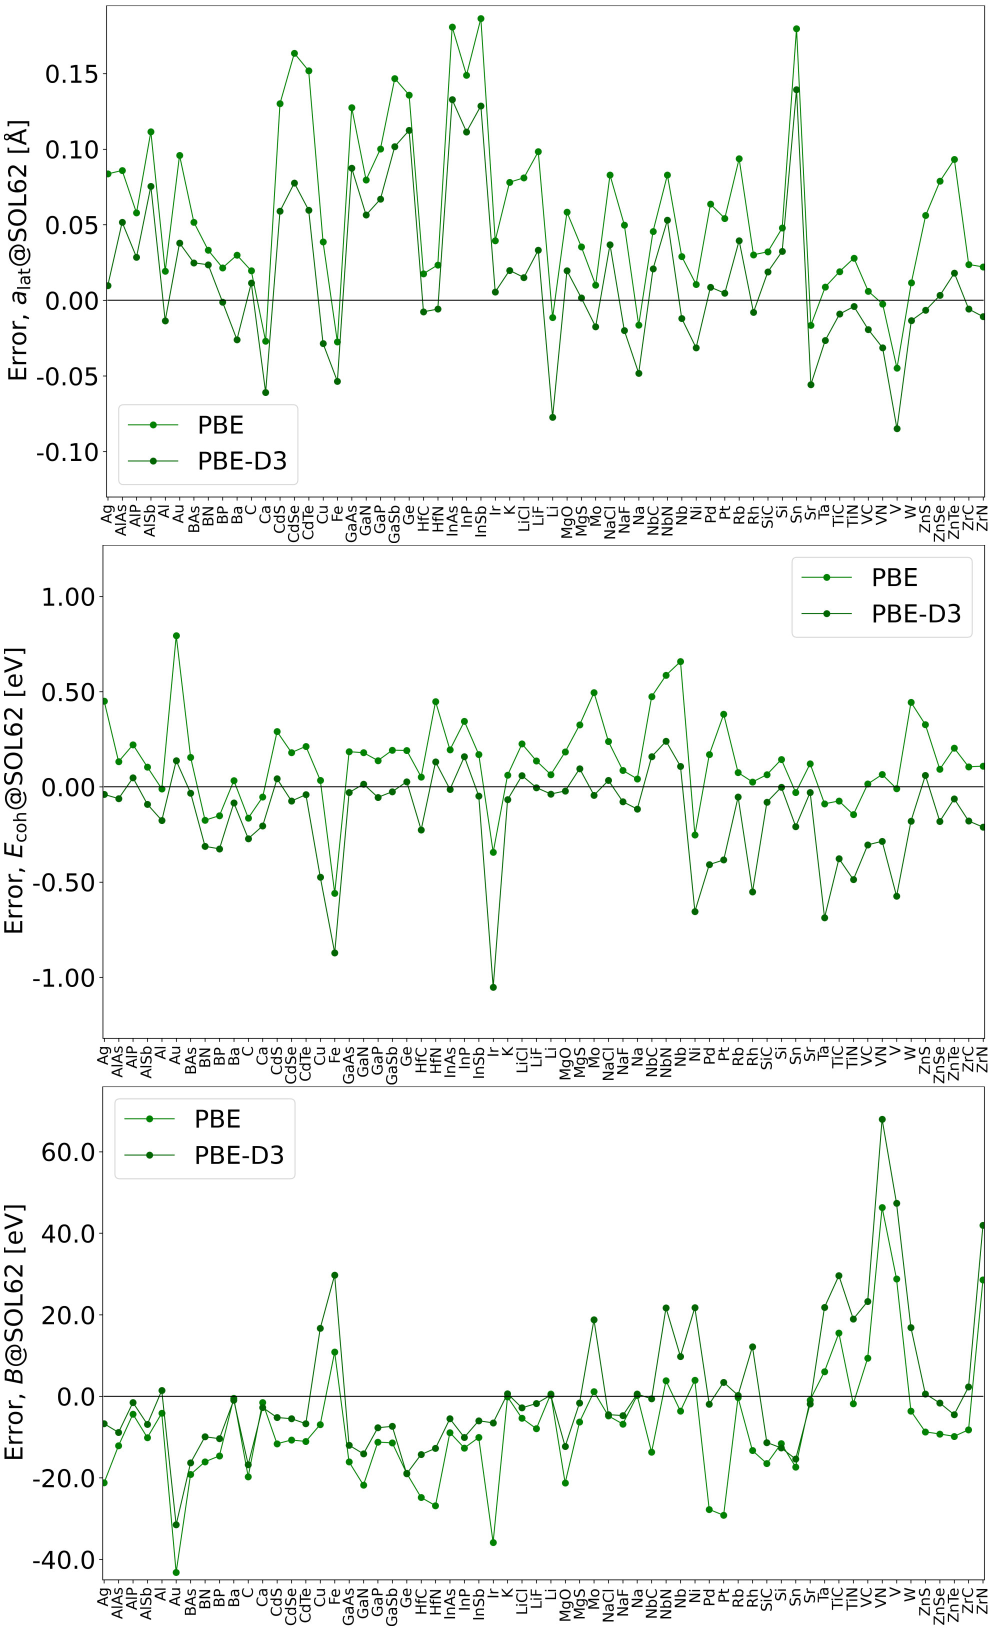


Figure SF3: Errors for all data sets using PBE and PBE-D3. Continued. The x-axes denote the systems. All values can be found in Tabs. ST23, ST24, and ST25.

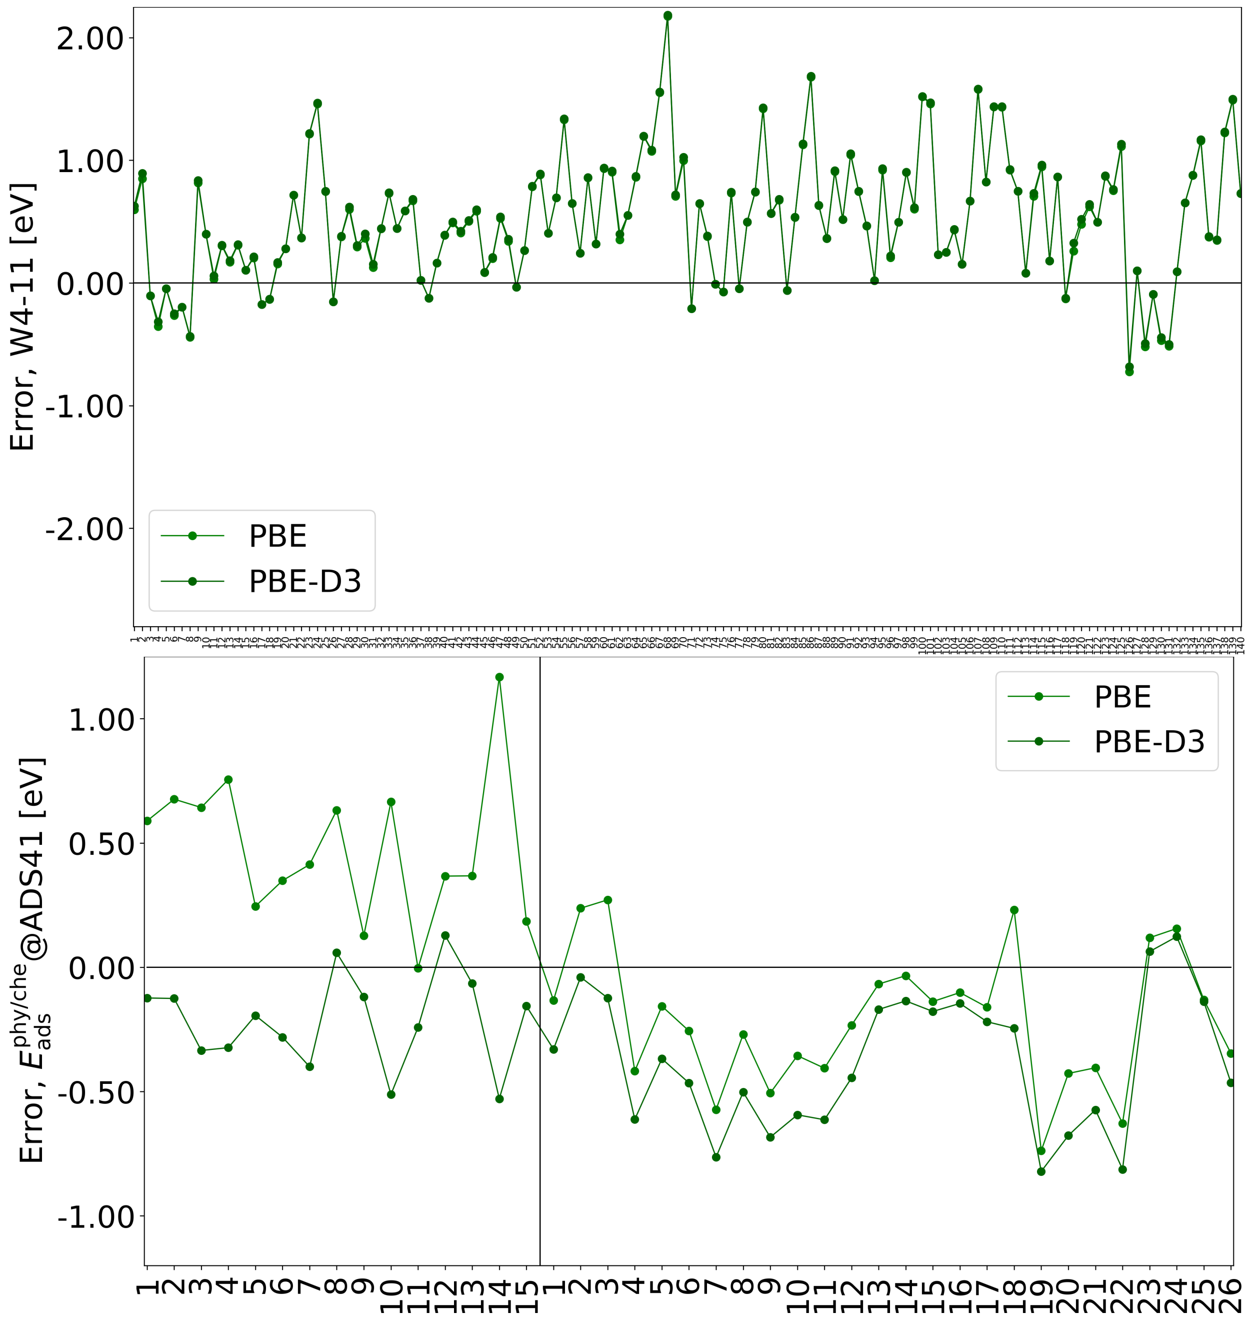


Figure SF4: Errors for all data sets using PBE and PBE-D3. Continued. The line in the ADS41 plot separates $E_{ads}^{phy}$@ADS41 from $E_{ads}^{che}$@ADS41. The x-axes denote the identifiers, see Tabs. ST21 (W4-11) and ST26 (ADS41).

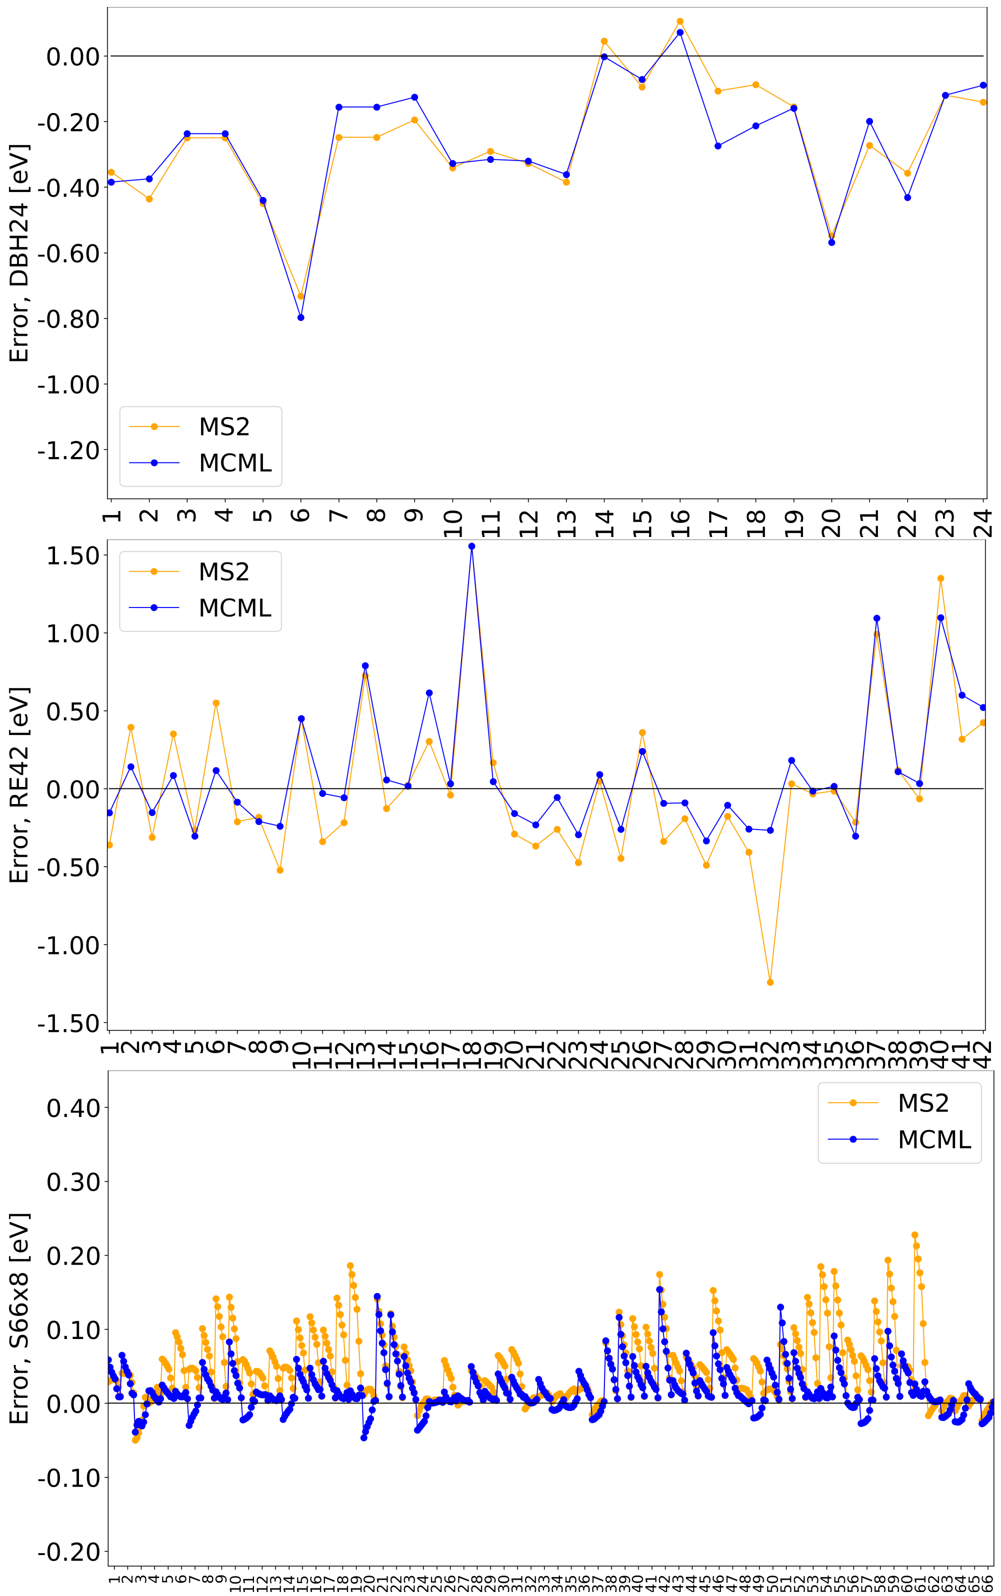


Figure SF5: Errors for all data sets using MS2 and MCML. The x-axes denote the identifiers, see Tabs. ST6 (DBH24), ST8 (RE42), and ST10 (S66x8).

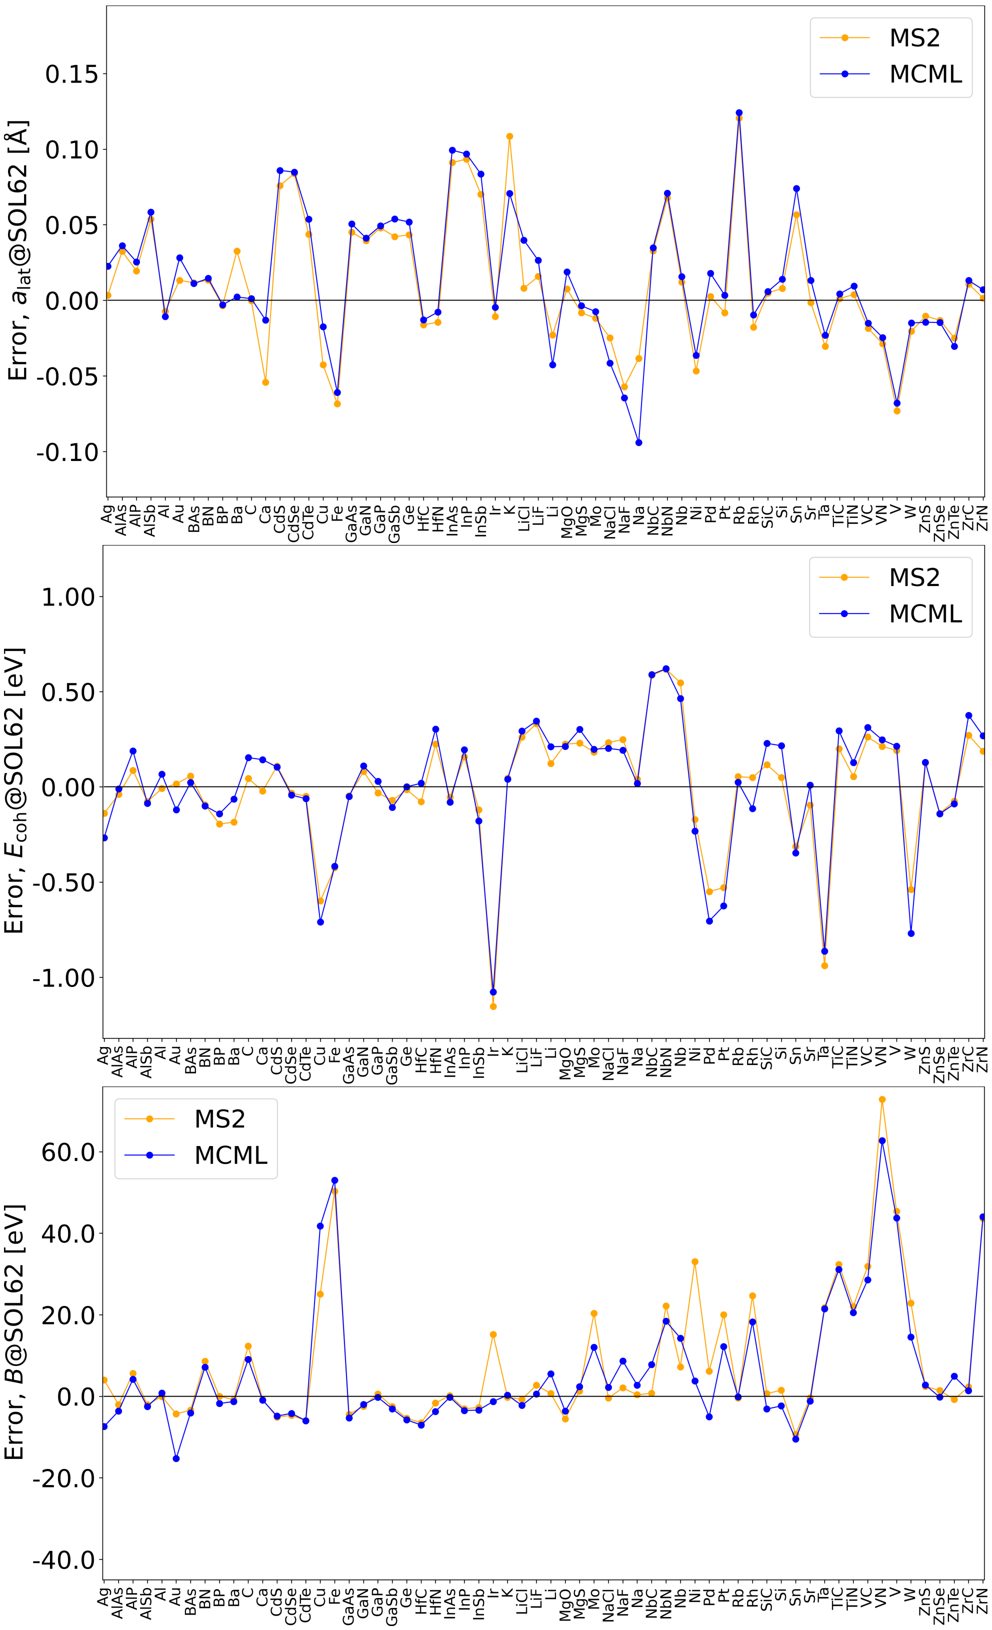


Figure SF6: Errors for all data sets using MS2 and MCML. Continued. The x-axes denote the systems. All values can be found in Tabs. ST23, ST24, and ST25.

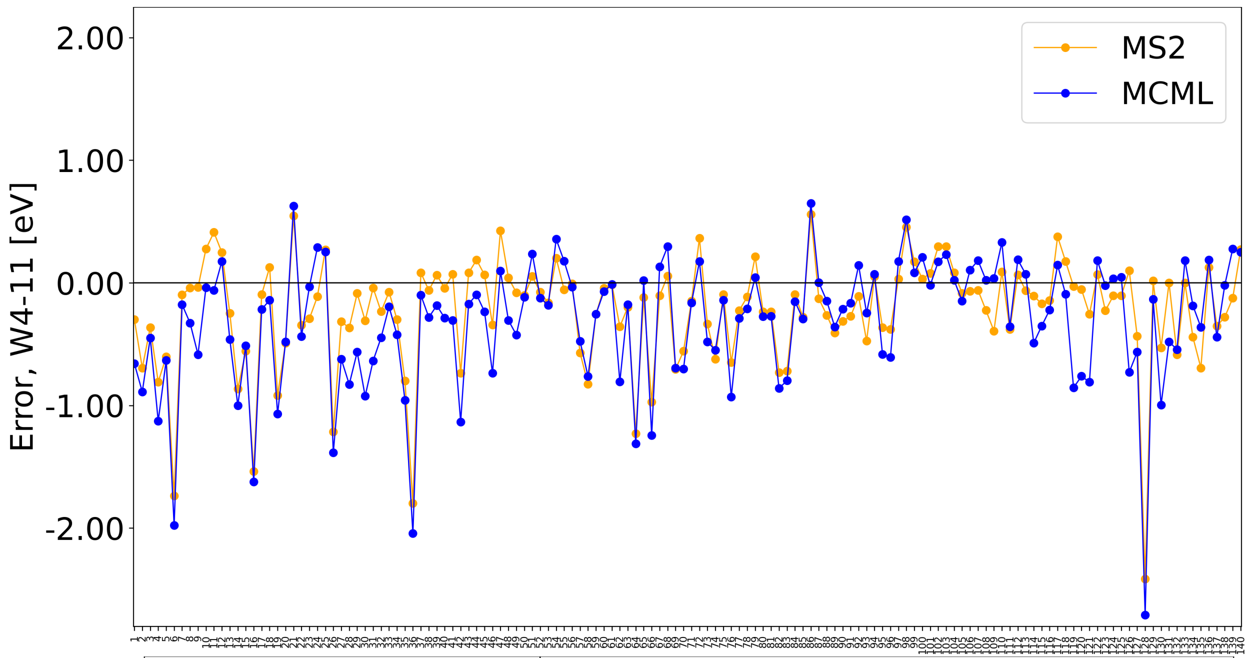


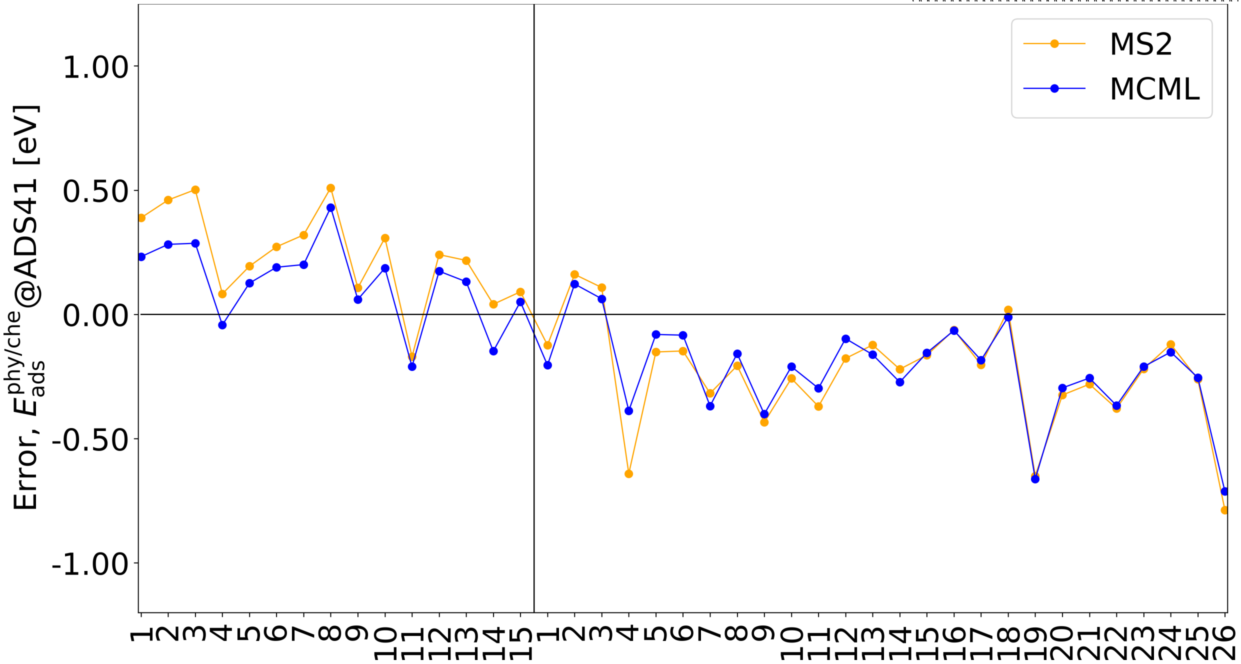


Figure SF7: Errors for all data sets using MS2 and MCML. Continued. The line in the ADS41 plot separates $E_{\mathrm{ads}}^{\mathrm{phy}}$@ADS41 from $E_{\mathrm{ads}}^{\mathrm{che}}$@ADS41. The x-axes denote the identifiers, see Tabs. ST21 (W4-11) and ST26 (ADS41).

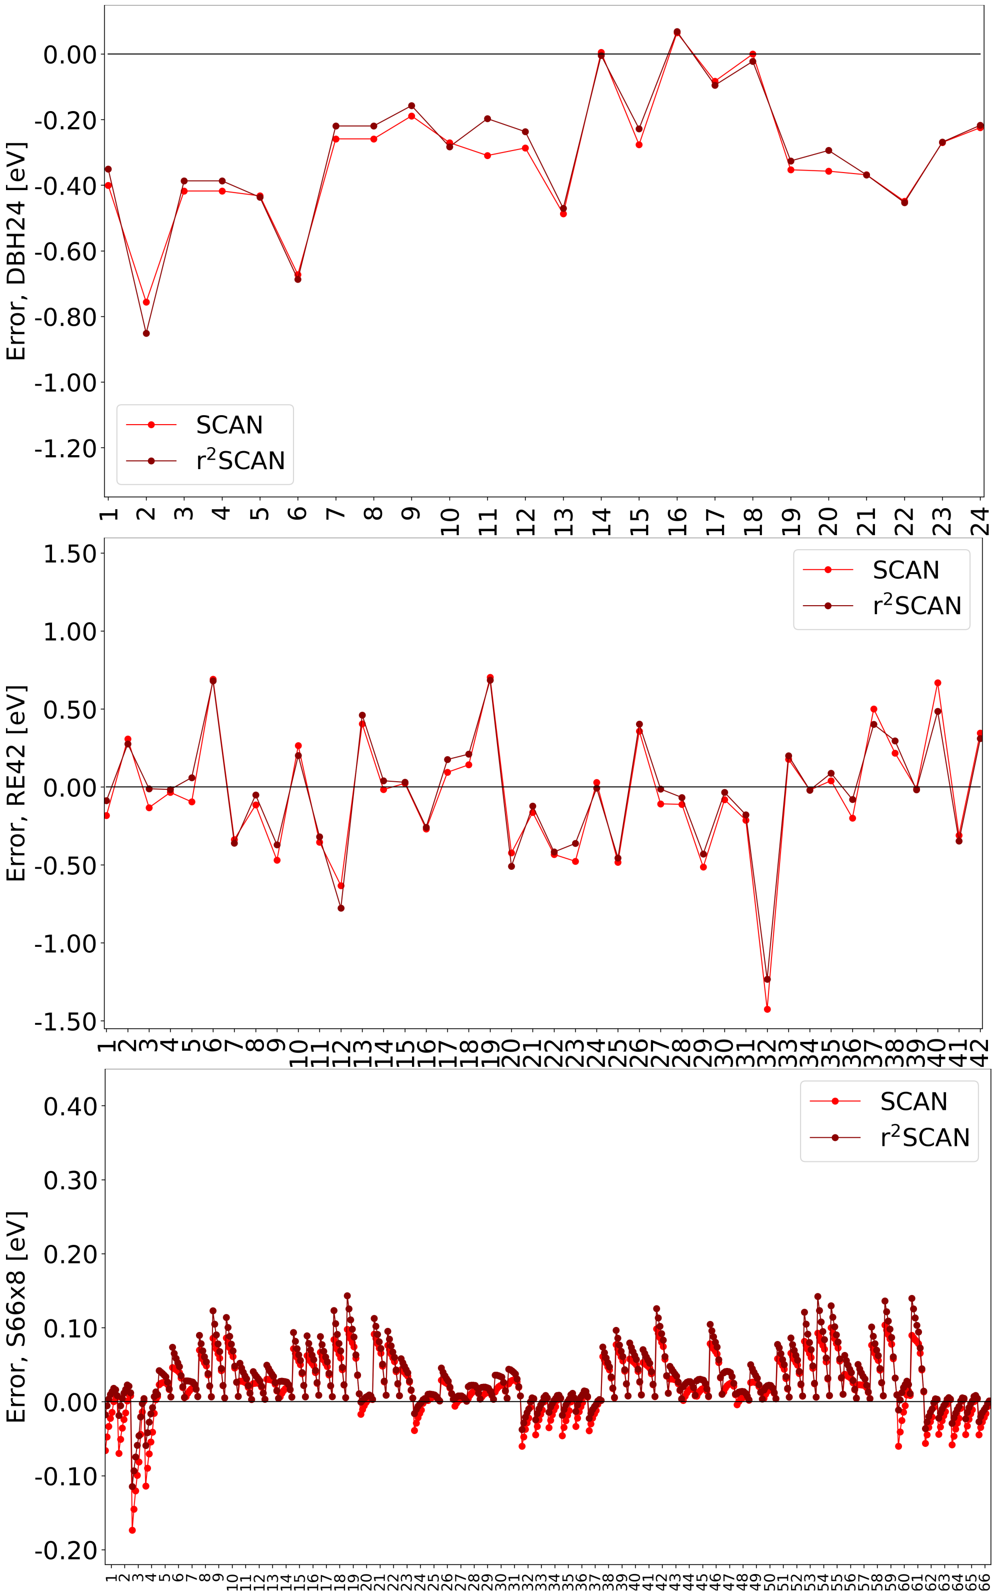


Figure SF8: Errors for all data sets using SCAN and r$^2$SCAN. The x-axes denote the identifiers, see Tabs. ST6 (DBH24), ST8 (RE42), and ST10 (S66x8).

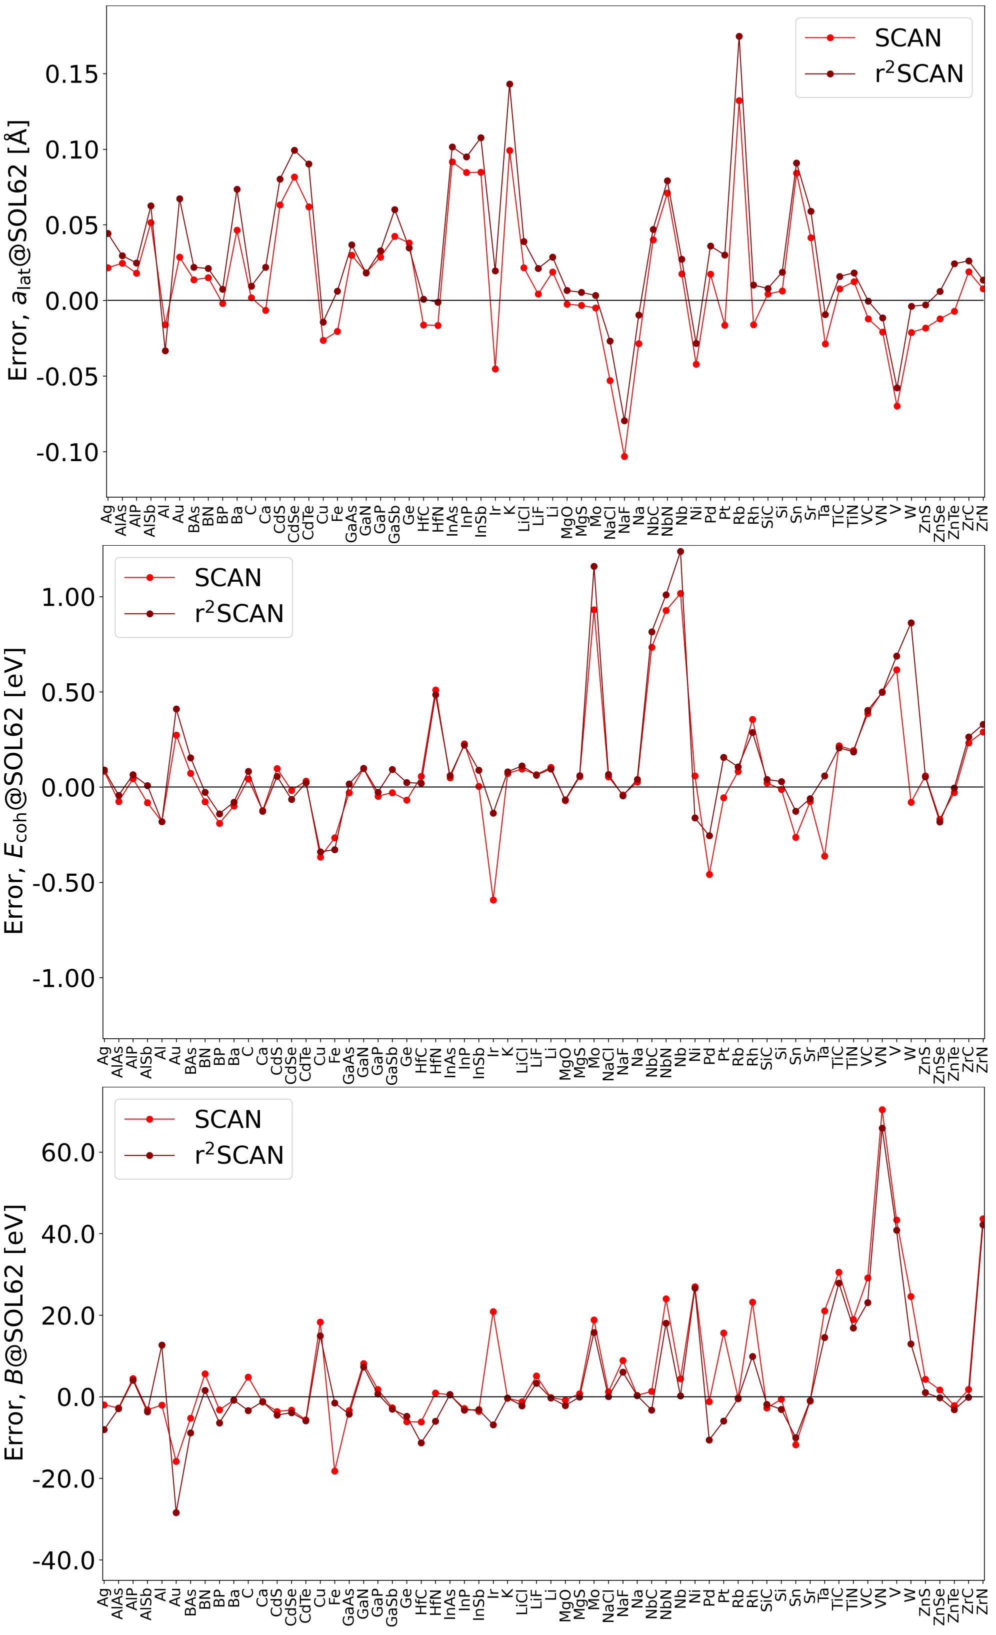


Figure SF9: Errors for all data sets using SCAN and r$^2$SCAN. Continued. The x-axes denote the systems. All values can be found in Tabs. ST23, ST24, and ST25.

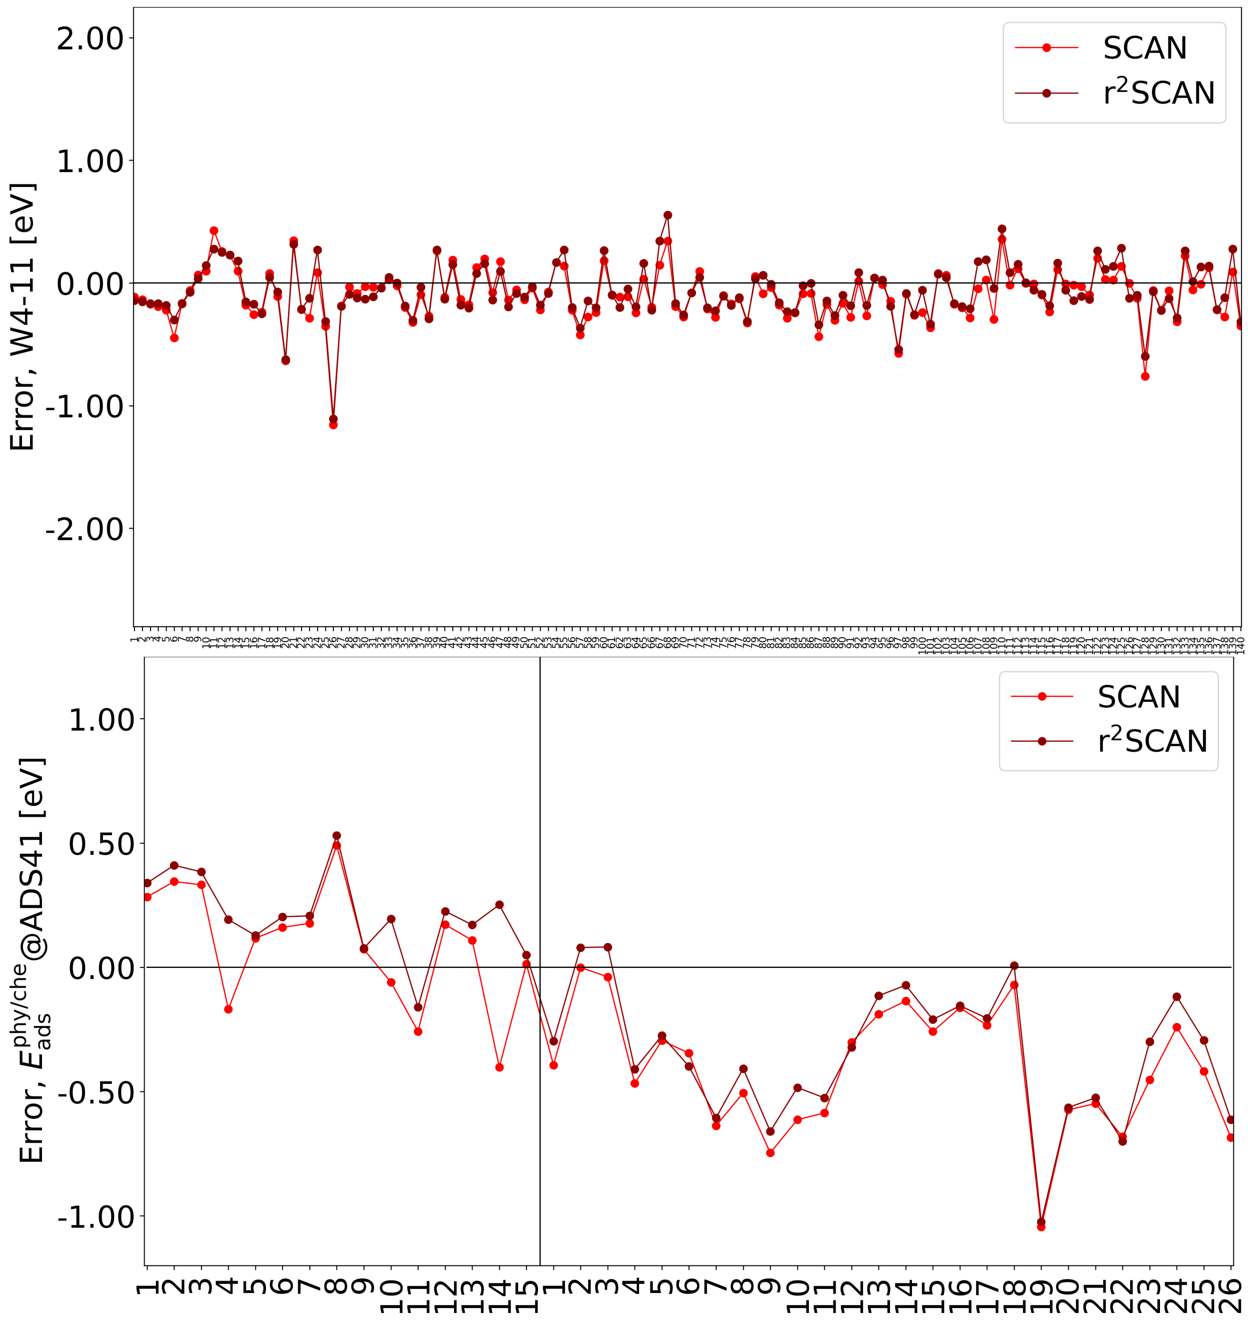


Figure SF10: Errors for all data sets using SCAN and r$^2$SCAN. Continued. The line in the ADS41 plot separates $E_{\text{ads}}^{\text{phy}}$@ADS41 from $E_{\text{ads}}^{\text{che}}$@ADS41. The x-axes denote the identifiers, see Tabs. ST21 (W4-11) and ST26 (ADS41).

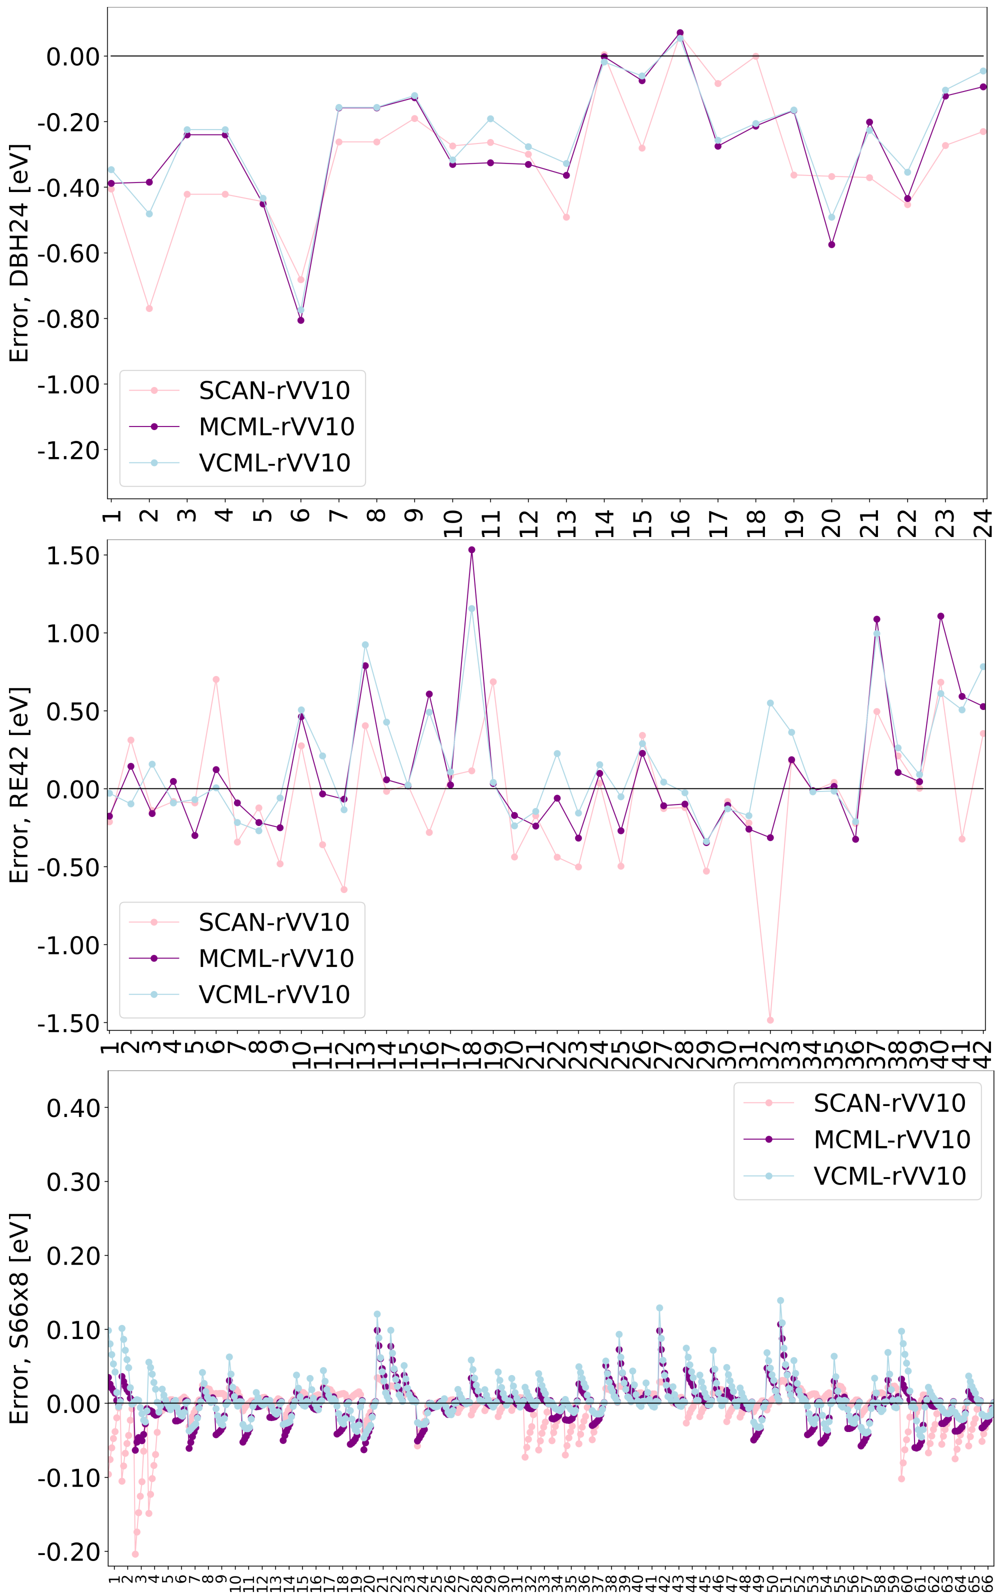


Figure SF11: Errors for all data sets using SCAN-rVV10, MCML-rVV10 and VCML-rVV10. The x-axes denote the identifiers, see Tabs. ST6 (DBH24), ST8 (RE42), and ST10 (S66x8).

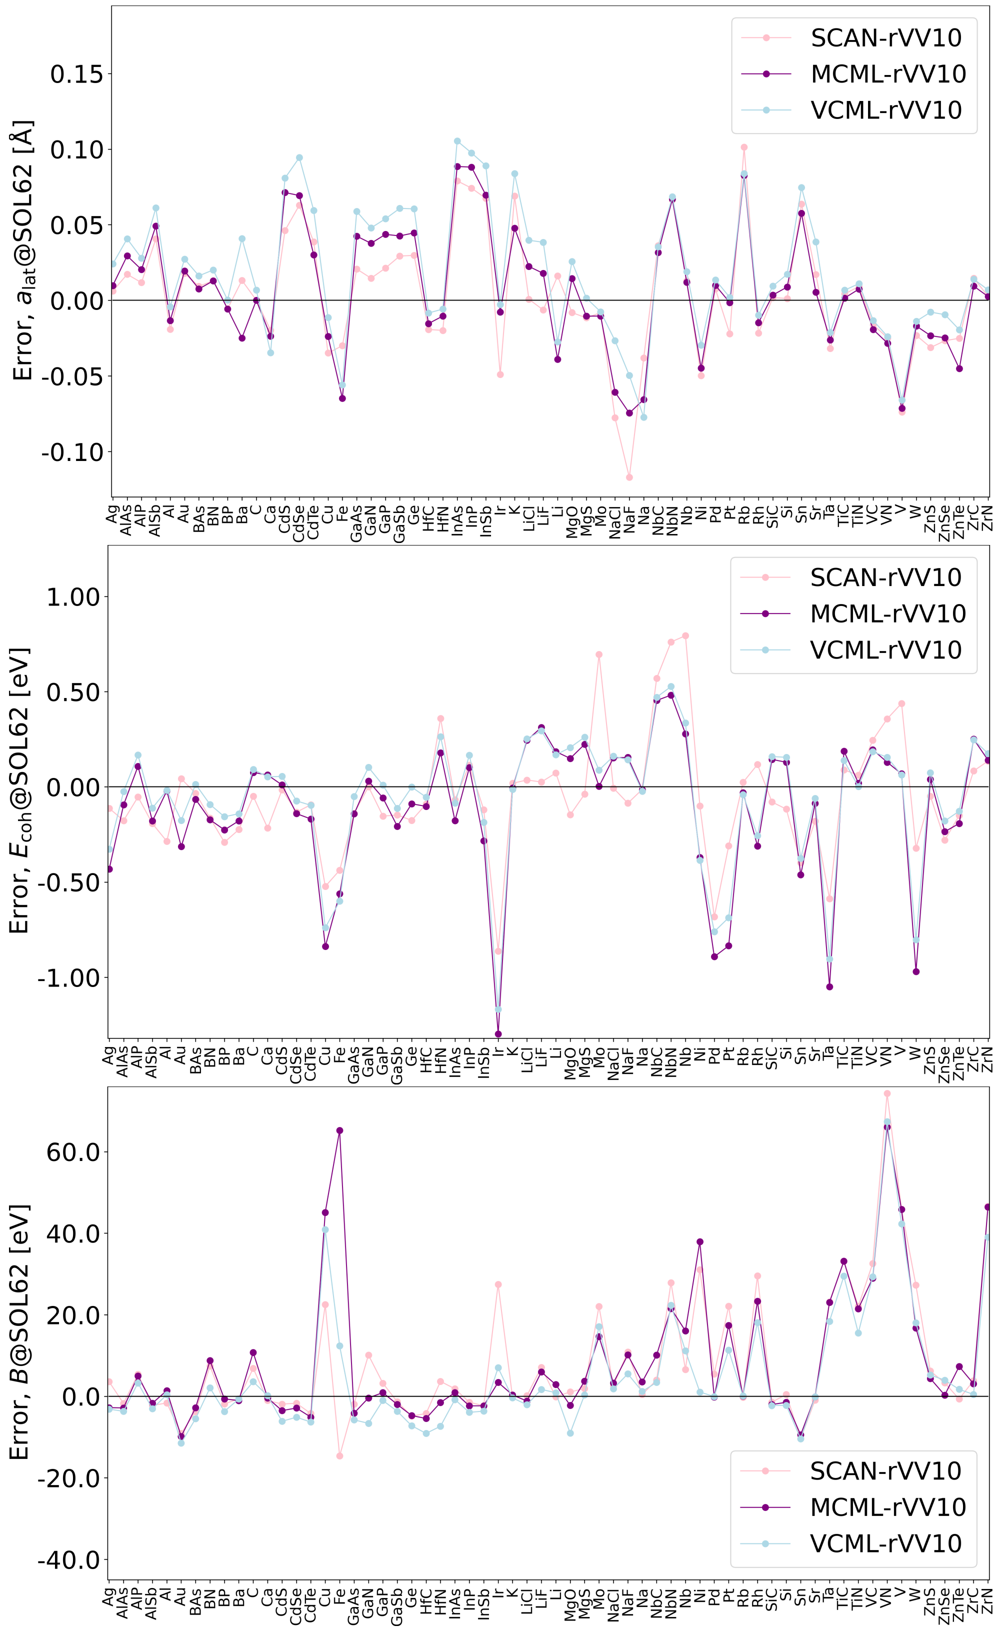


Figure SF12: Errors for all data sets using SCAN-rVV10, MCML-rVV10 and VCML-rVV10. Continued. The x-axes denote the systems. All values can be found in Tabs. ST23, ST24, and ST25.

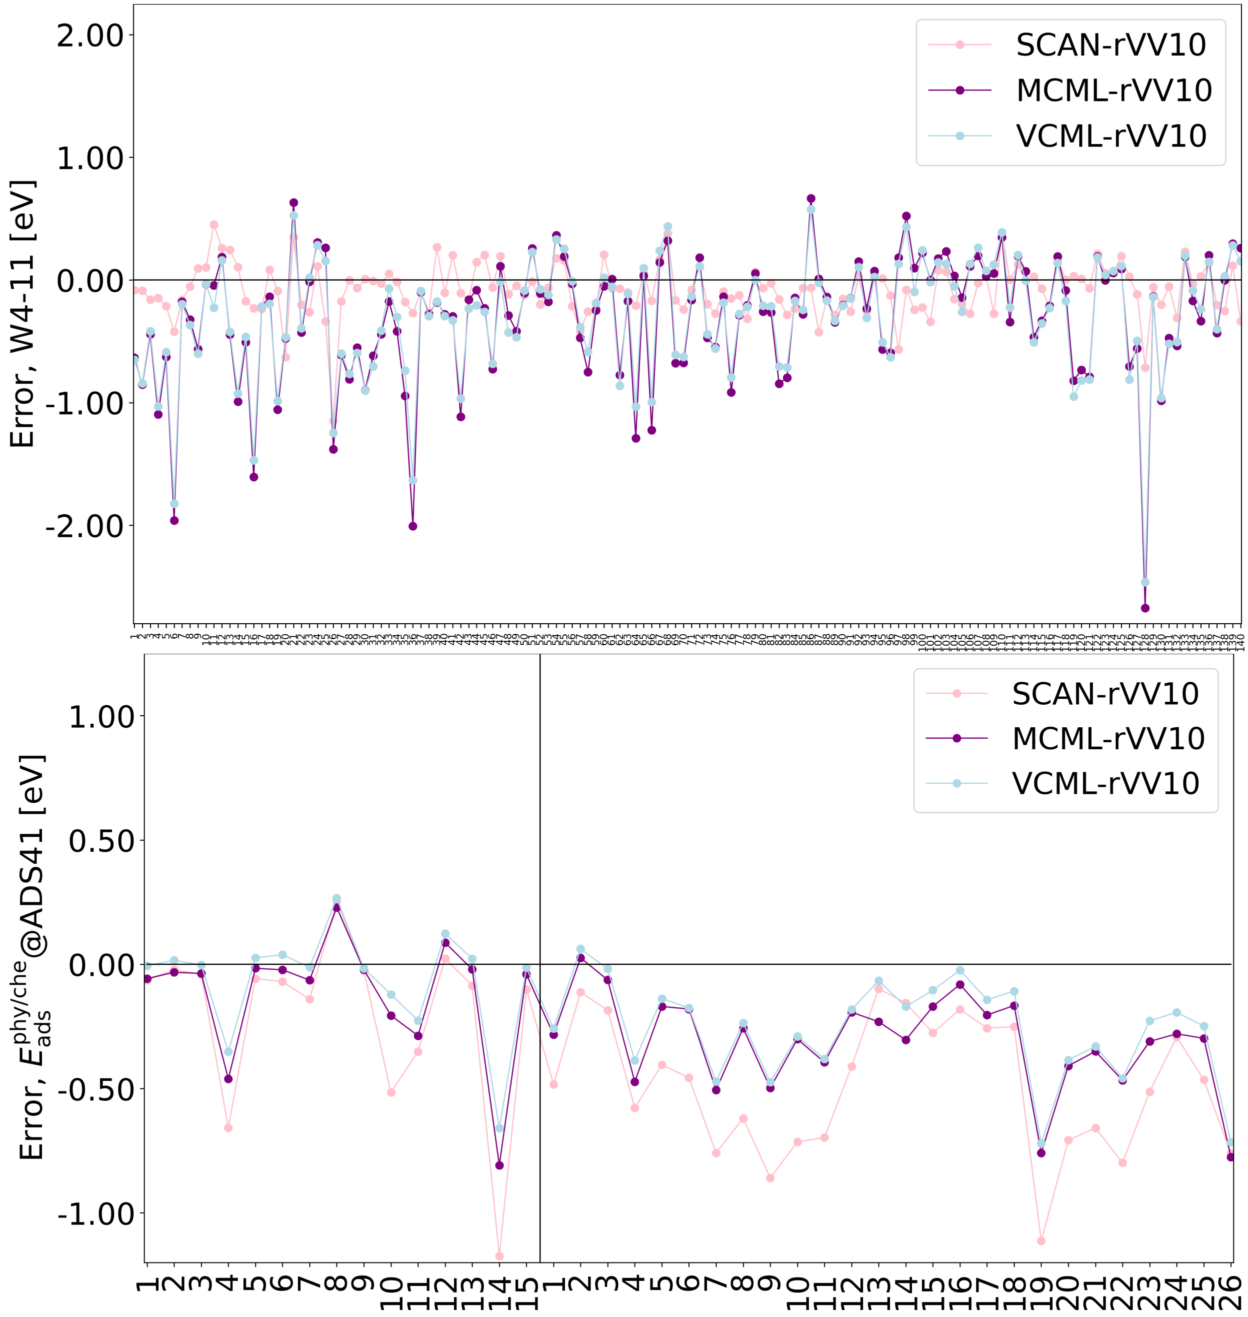


Figure SF13: Errors for all data sets using SCAN-rVV10, MCML-rVV10 and VCML-rVV10. Continued. The line in the ADS41 plot separates $E_{\mathrm{ads}}^{\mathrm{phy}}$@ADS41 from $E_{\mathrm{ads}}^{\mathrm{che}}$@ADS41. The x-axes denote the identifiers, see Tabs. ST21 (W4-11) and ST26 (ADS41). As a note, the $b$ parameter for MCML-rVV10 is larger than for VCML-rVV10, thus having a weaker vdW interaction; however, it overbinds more, showing that reshaping the functional form has made significant improvements possible.

# References


[1] R. Sabatini, T. Gorni, and S. de Gironcoli. Nonlocal van der Waals density functional made simple and efficient. *Phys. Rev. B*, 87:041108, 2013. doi: 10.1103/PhysRevB.87.041108.

[2] H. Peng, Z.-H. Yang, J. P. Perdew, and J. Sun. Versatile van der Waals Density Functional Based on a Meta-Generalized Gradient Approximation. *Phys. Rev. X*, 6:041005, 2016. doi: 10.1103/PhysRevX.6.041005.

[3] O. A. Vydrov and T. Van Voorhis. Nonlocal van der Waals density functional: The simpler the better. *J. Chem. Phys.*, 133:244103, 2010. doi: 10.1063/1.3521275.

[4] K. Brown, Y. Maimaiti, K. Trepte, T. Bligaard, and J. Voss. MCML: Combining physical constraints with experimental data for a multi-purpose meta-generalized gradient approximation. *J. Comput. Chem.*, 42:2004–2013, 2021. doi: https://doi.org/10.1002/jcc.26732.
